# Supplementary material for: Stationary subspace analysis of nonstationary covariance processes: eigenstructure description and testing
Source: arXiv:1904.09420 source file (2019-04-20)
Supplement: Supplementary file 1 [file ssa_appendix_1.tex]

\appendix

\section{Additional figures for Section \ref{s:simulation}}

\subsection{Figures for Section \ref{s:simulation_dimension}}

\begin{figure}[H]
\begin{center}
\includegraphics[scale=0.34]{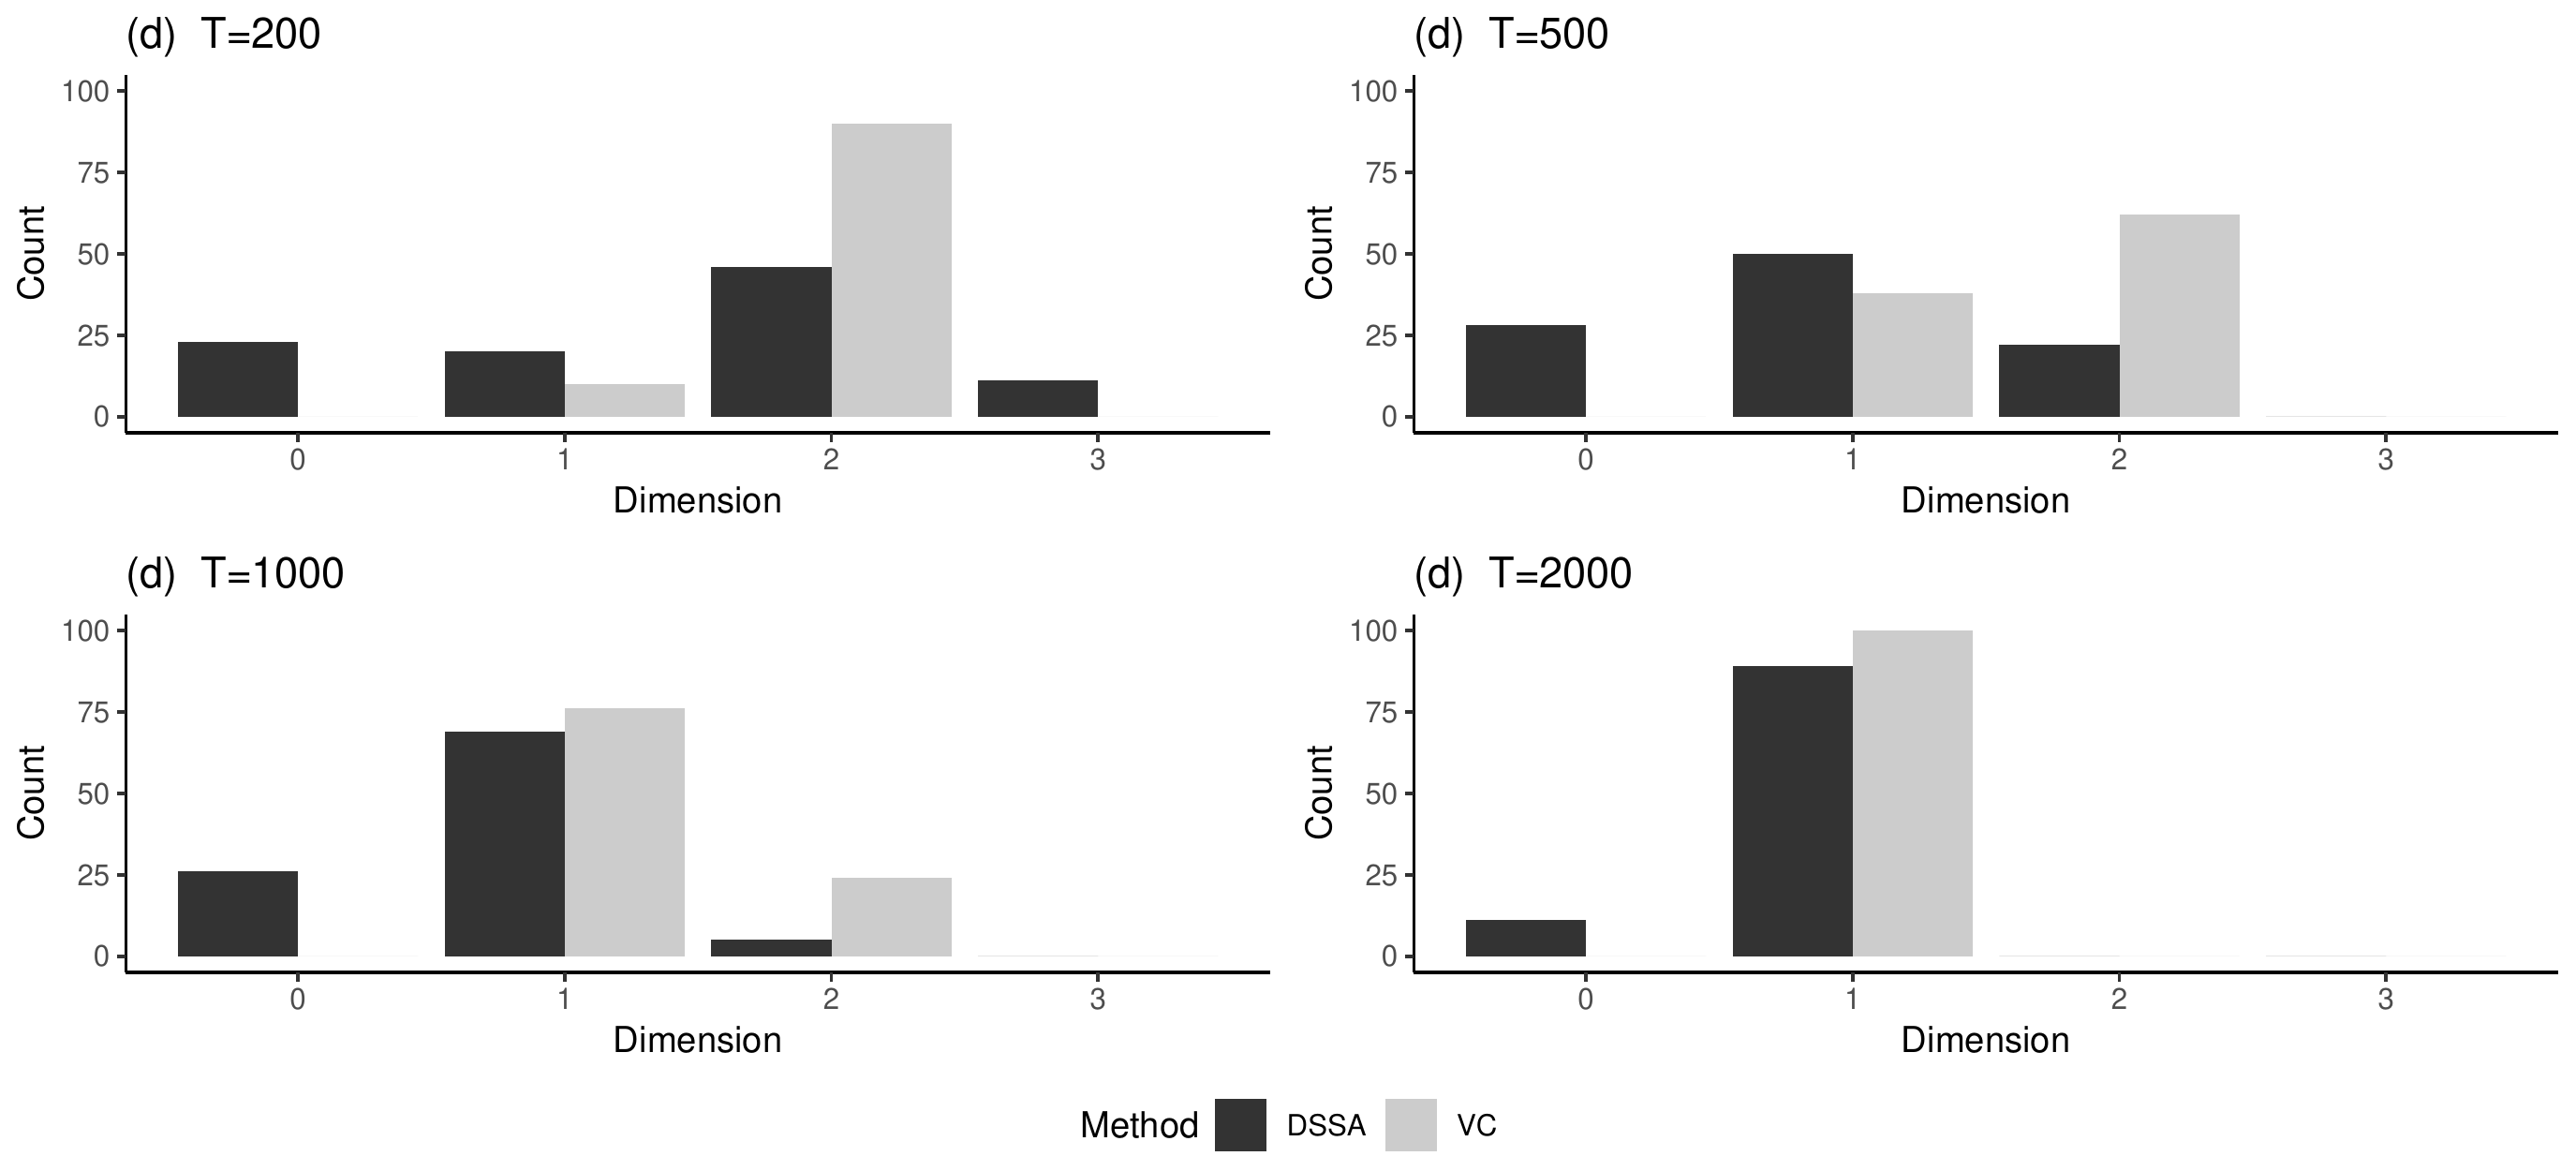}
\end{center}
\vspace{-0.75cm}
\caption{Model 1: Histograms of the estimates of $d$ for the indicated  sample sizes for the two competing methods: DSSA (\citet{sundararajan:2017}) and VC (proposed method). The true value is $d=1$. } \label{fig:model_1}
\end{figure}

%\begin{figure}[H]
%\begin{center}
%\includegraphics[scale=0.45]{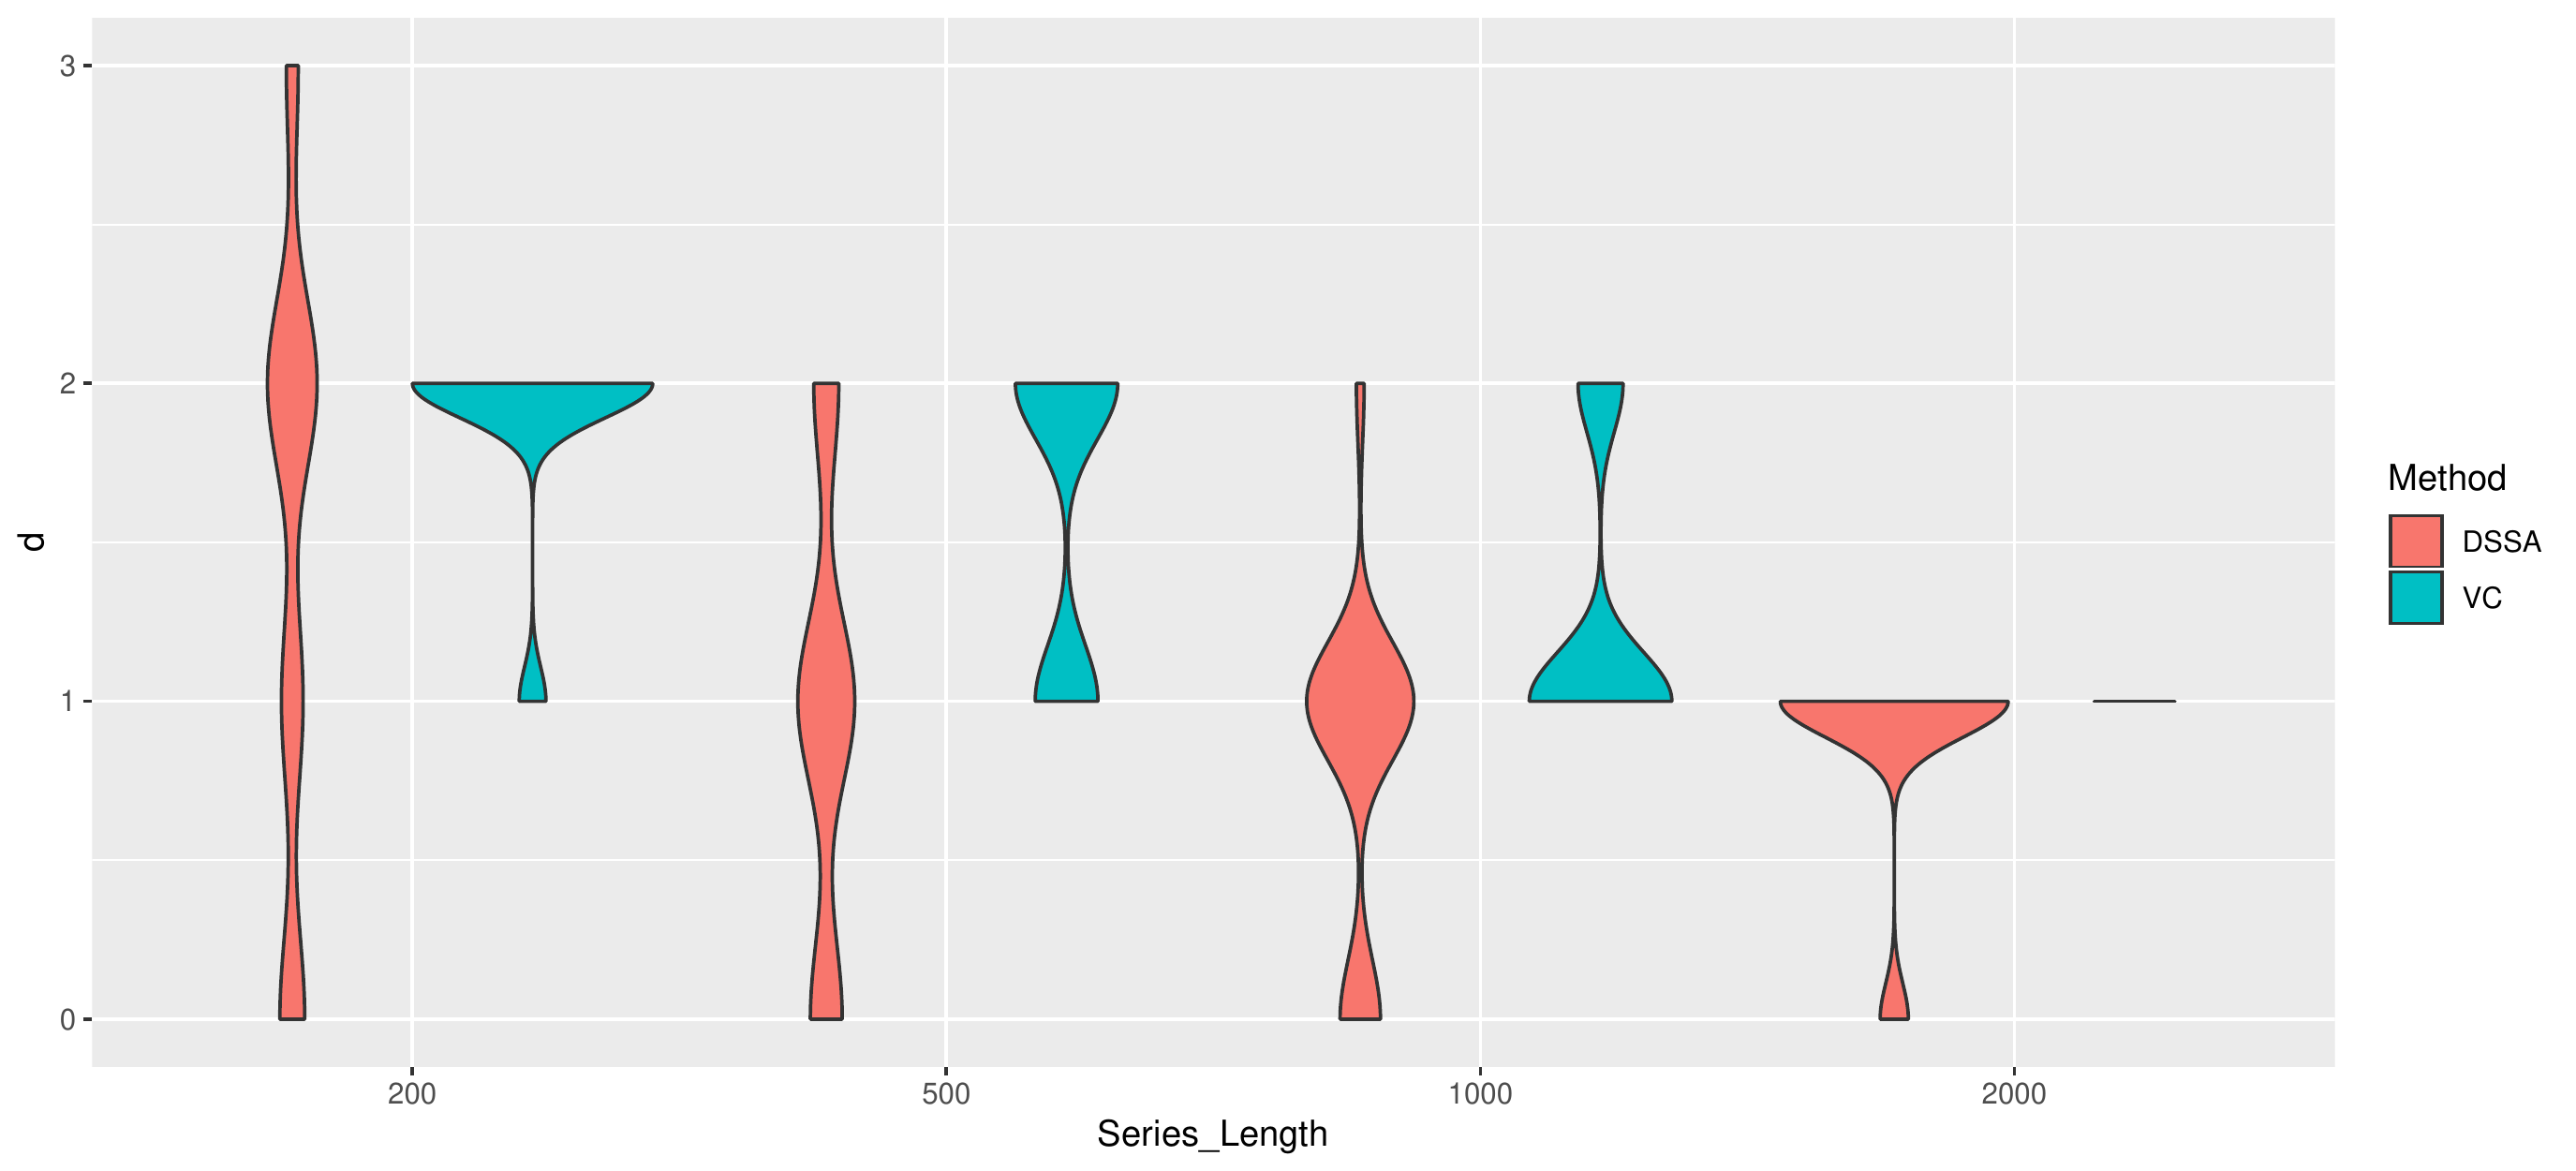}
%\end{center}
%\caption{Model 1: Violin plot of the estimate of $d$ for the indicated  sample sizes for the two %competing methods: DSSA and VC (proposed method). The true value $d=1$. } \label{fig:model_1_violin}
%\end{figure}

\begin{figure}[H]
\begin{center}
\includegraphics[scale=0.34]{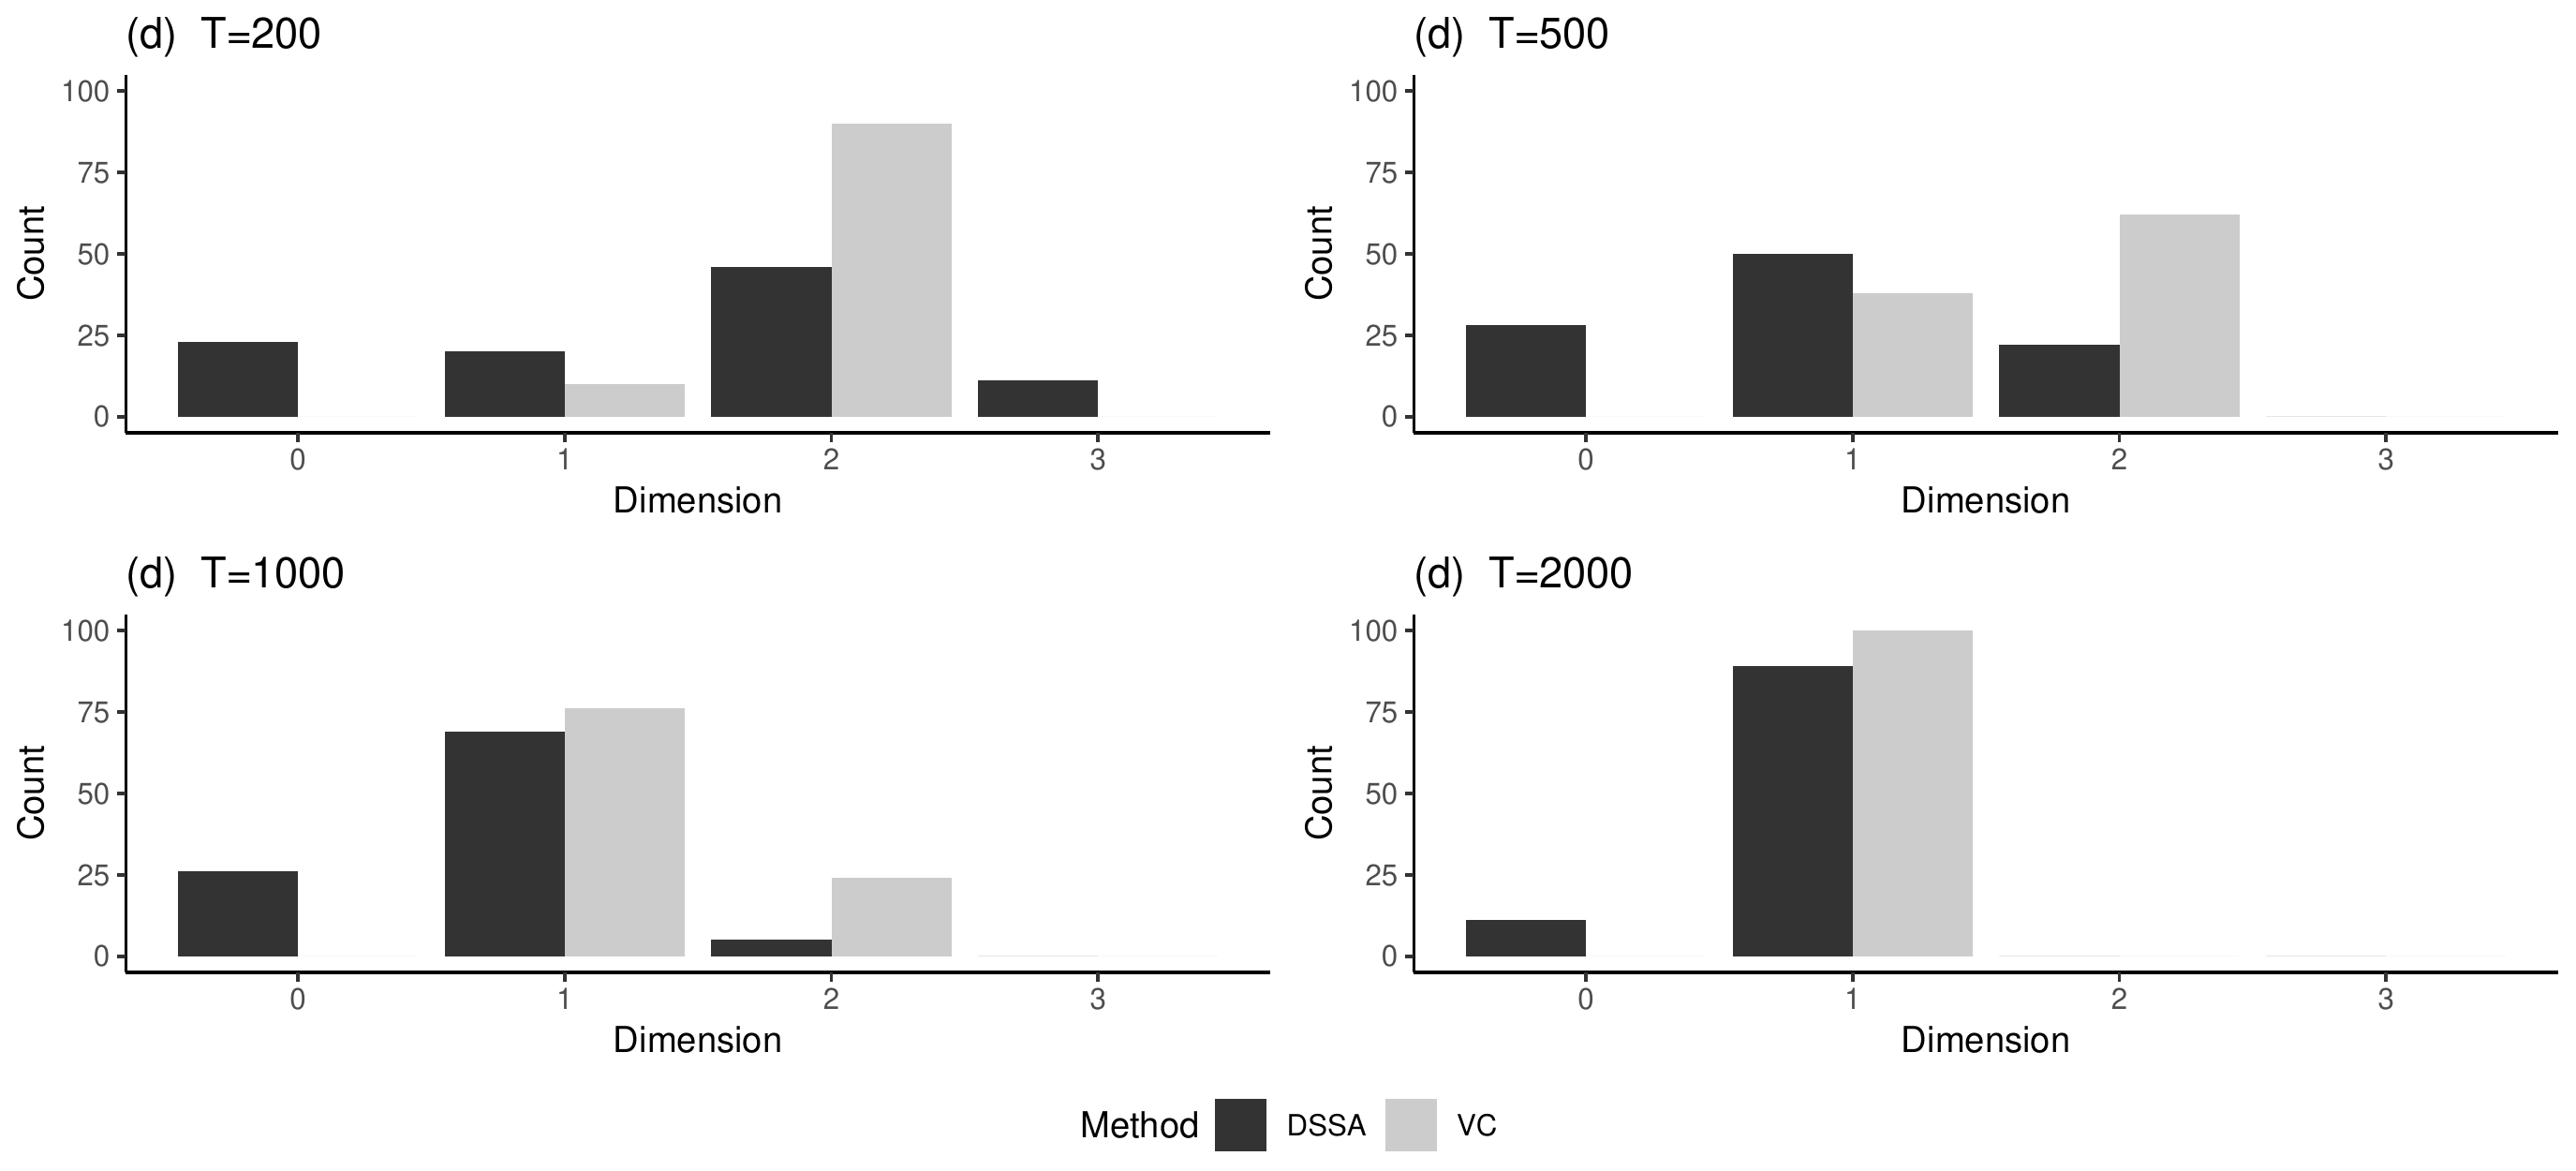}
\end{center}
\vspace{-0.75cm}
\caption{Model 2: Histograms of the estimates of $d$ for the indicated  sample sizes for the two competing methods: DSSA and VC (proposed method). The true value is $d=2$.   } \label{fig:model_2}
\end{figure}

\begin{figure}[H]
\begin{center}
\includegraphics[scale=0.34]{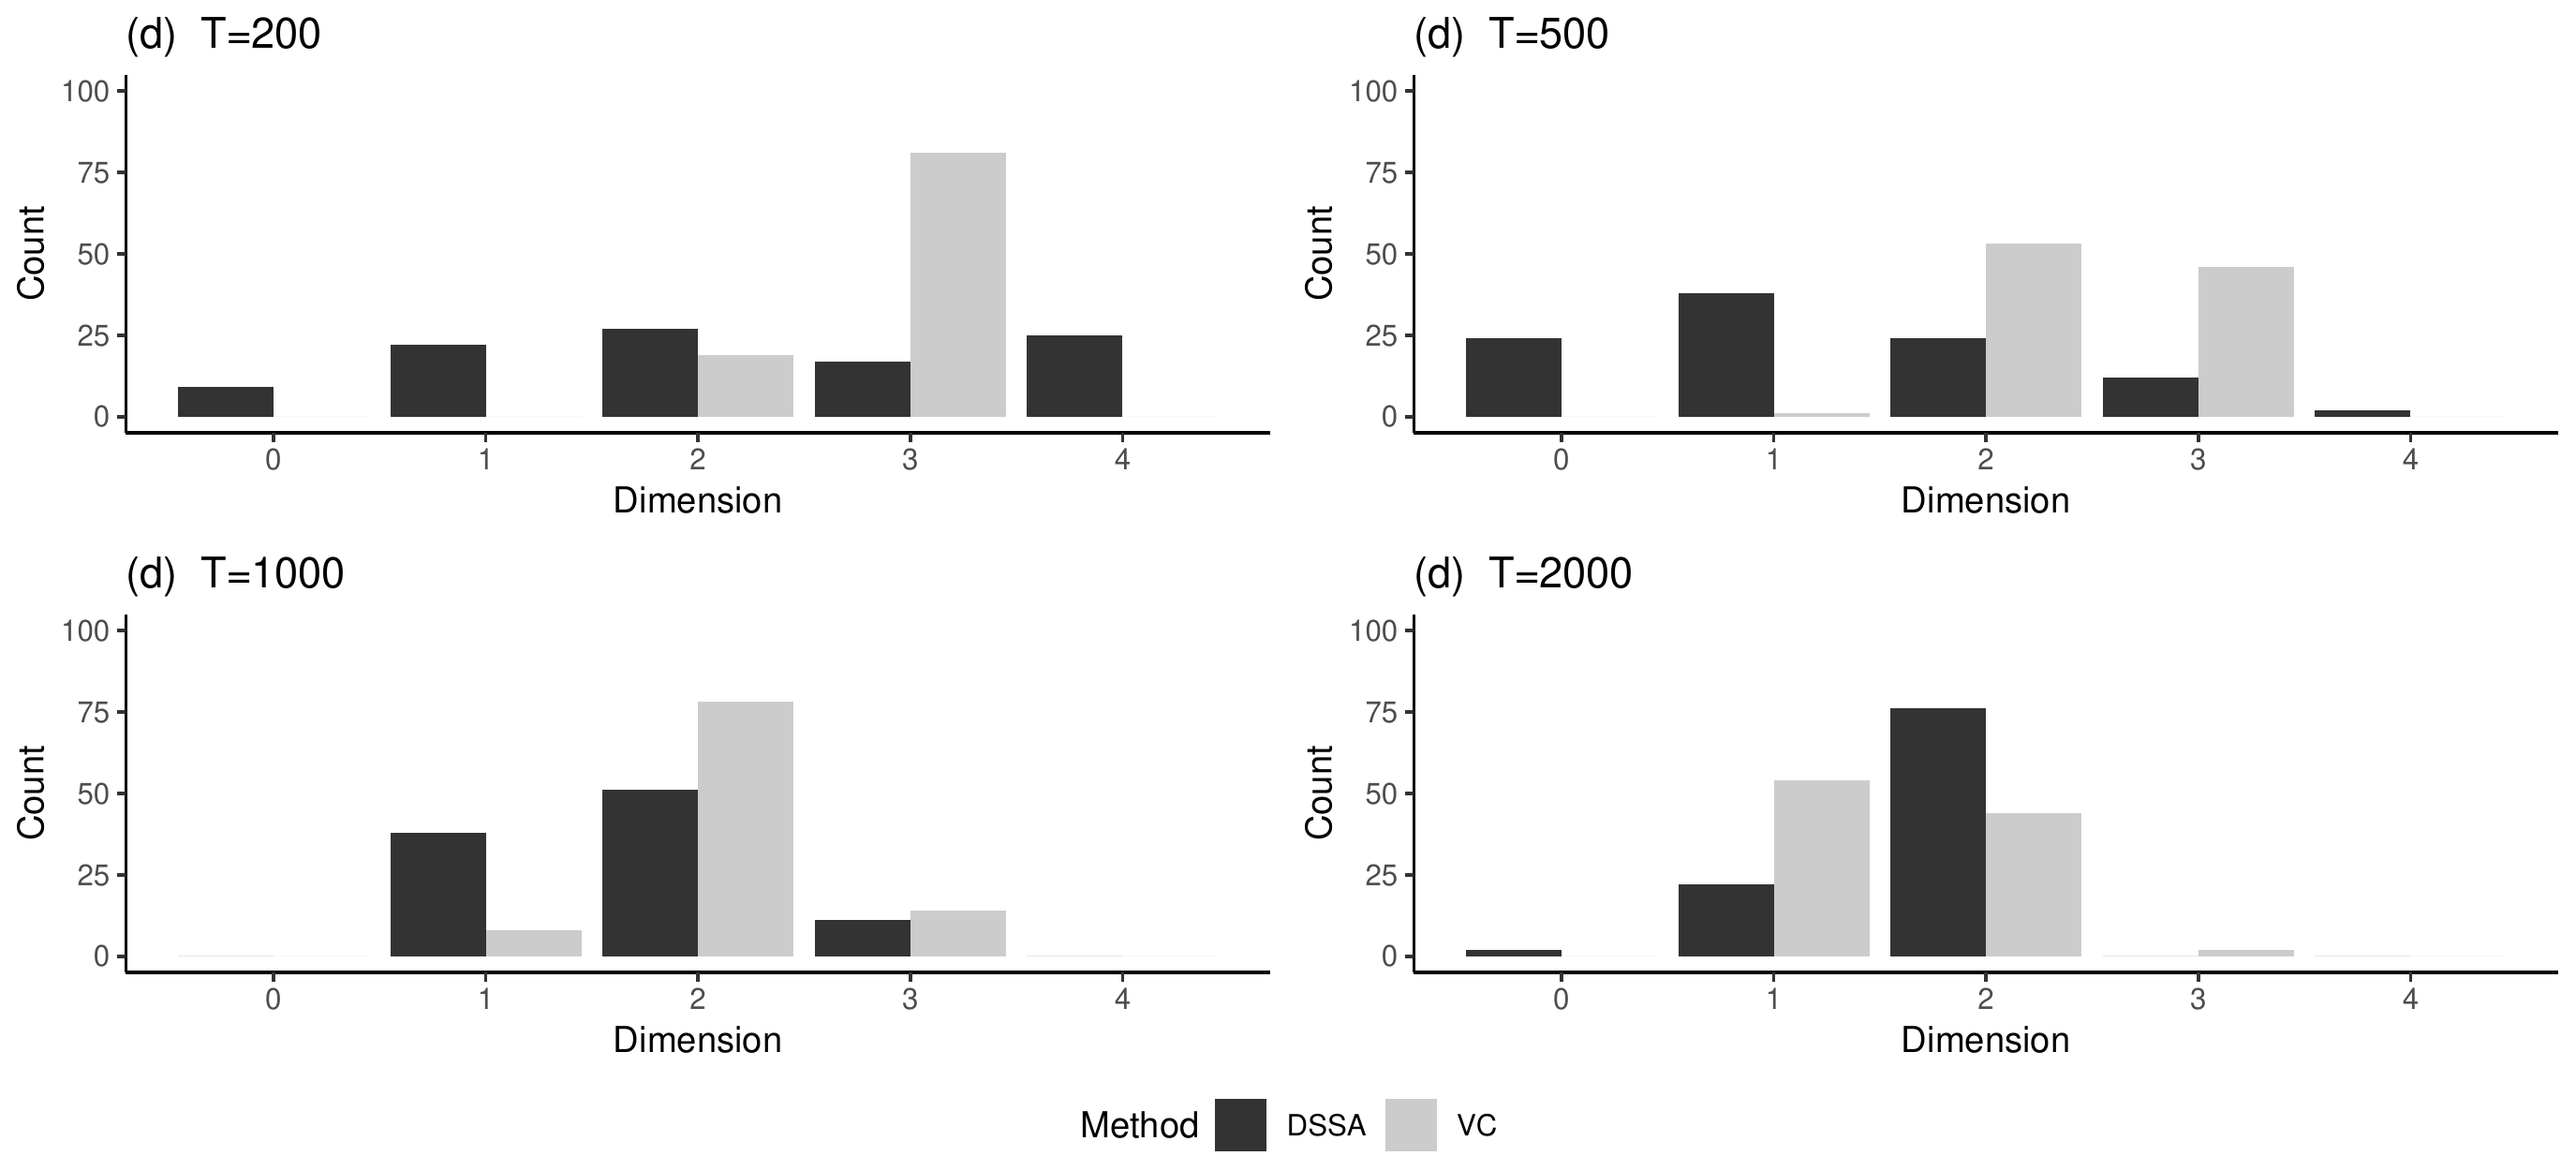}
\end{center}
\vspace{-0.75cm}
\caption{Model 3: Histograms of the estimates of $d$ for the indicated  sample sizes for the two competing methods: DSSA and VC (proposed method). The true value is $d=2$.  } \label{fig:model_3}
\end{figure}

\begin{figure}[H]
\begin{center}
\includegraphics[scale=0.34]{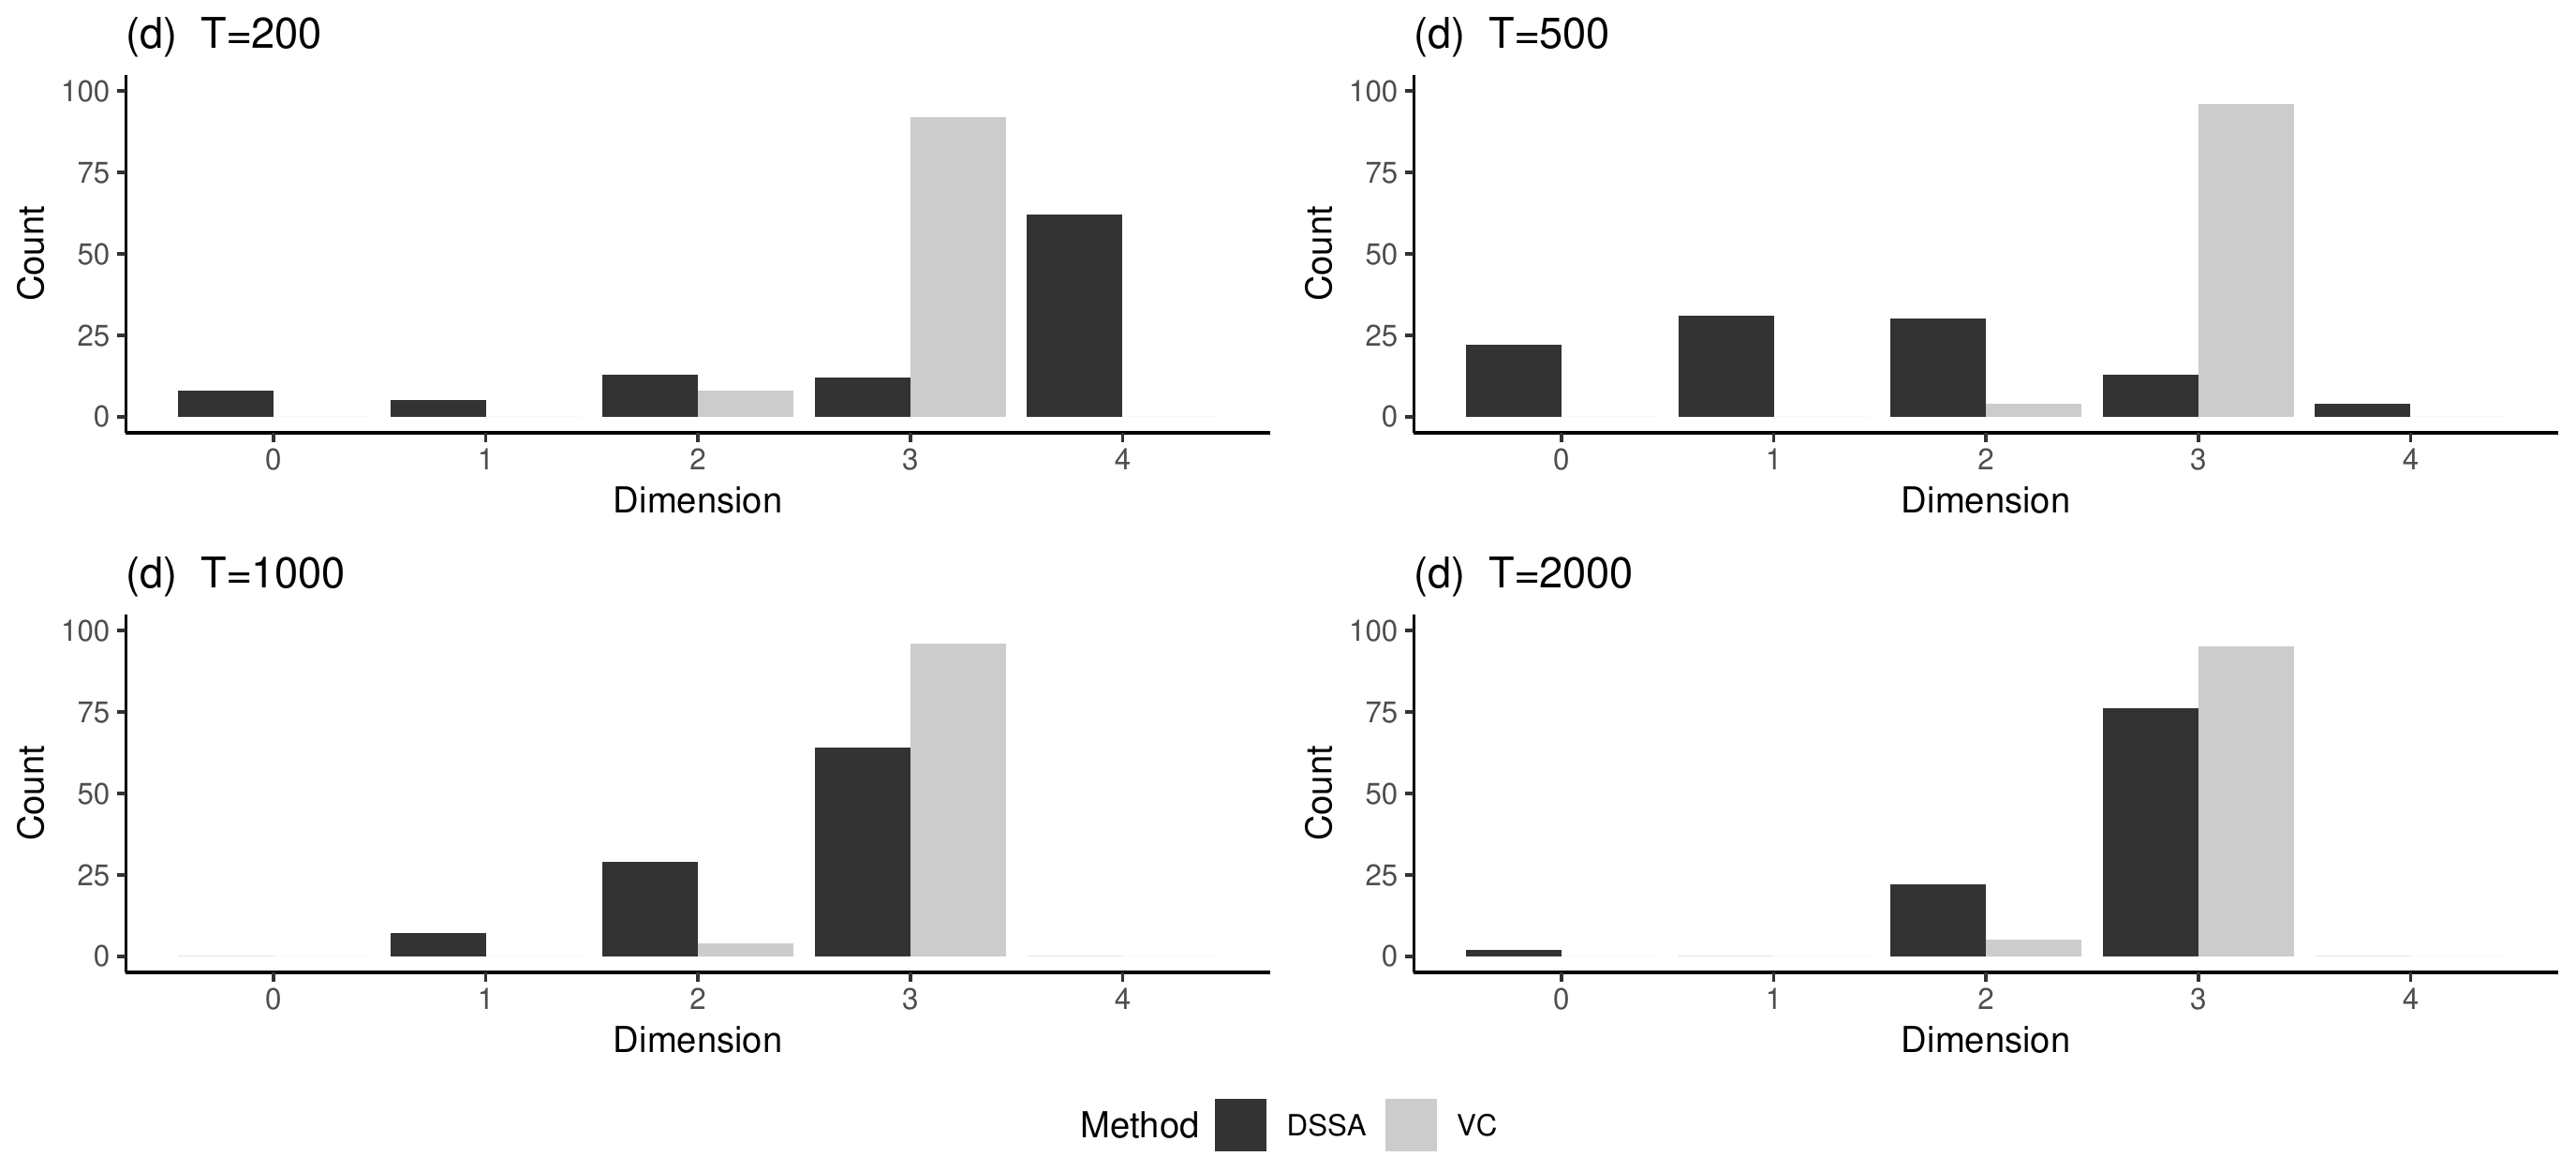}
\end{center}
\vspace{-0.75cm}
\caption{Model 4: Histograms of the estimates of $d$ for the indicated  sample sizes for the two competing methods: DSSA and VC (proposed method). The true value is $d=3$. The value of $\rho$ is set to 0.5. }\label{fig:model_4}
\end{figure}

%%%%%%%%%%%%%%%%%%%%%%%%%%%%%%%%%%%%%%%%%%%%%%%%%%%%%%%%%%%%%%%%%%%%%%%%%%%%%%%%%%%%%%%%%%
%%%%%%%%%%%%%%%%%%%%%%%%%%%%%%%%%%%%%%%%%%%%%%%%%%%%%%%%%%%%%%%%%%%%%%%%%%%%%%%%%%%%%%%%%%%

%% SPlitting Figures

%\begin{figure}[H]
%\begin{center}
%\includegraphics[scale=0.45]{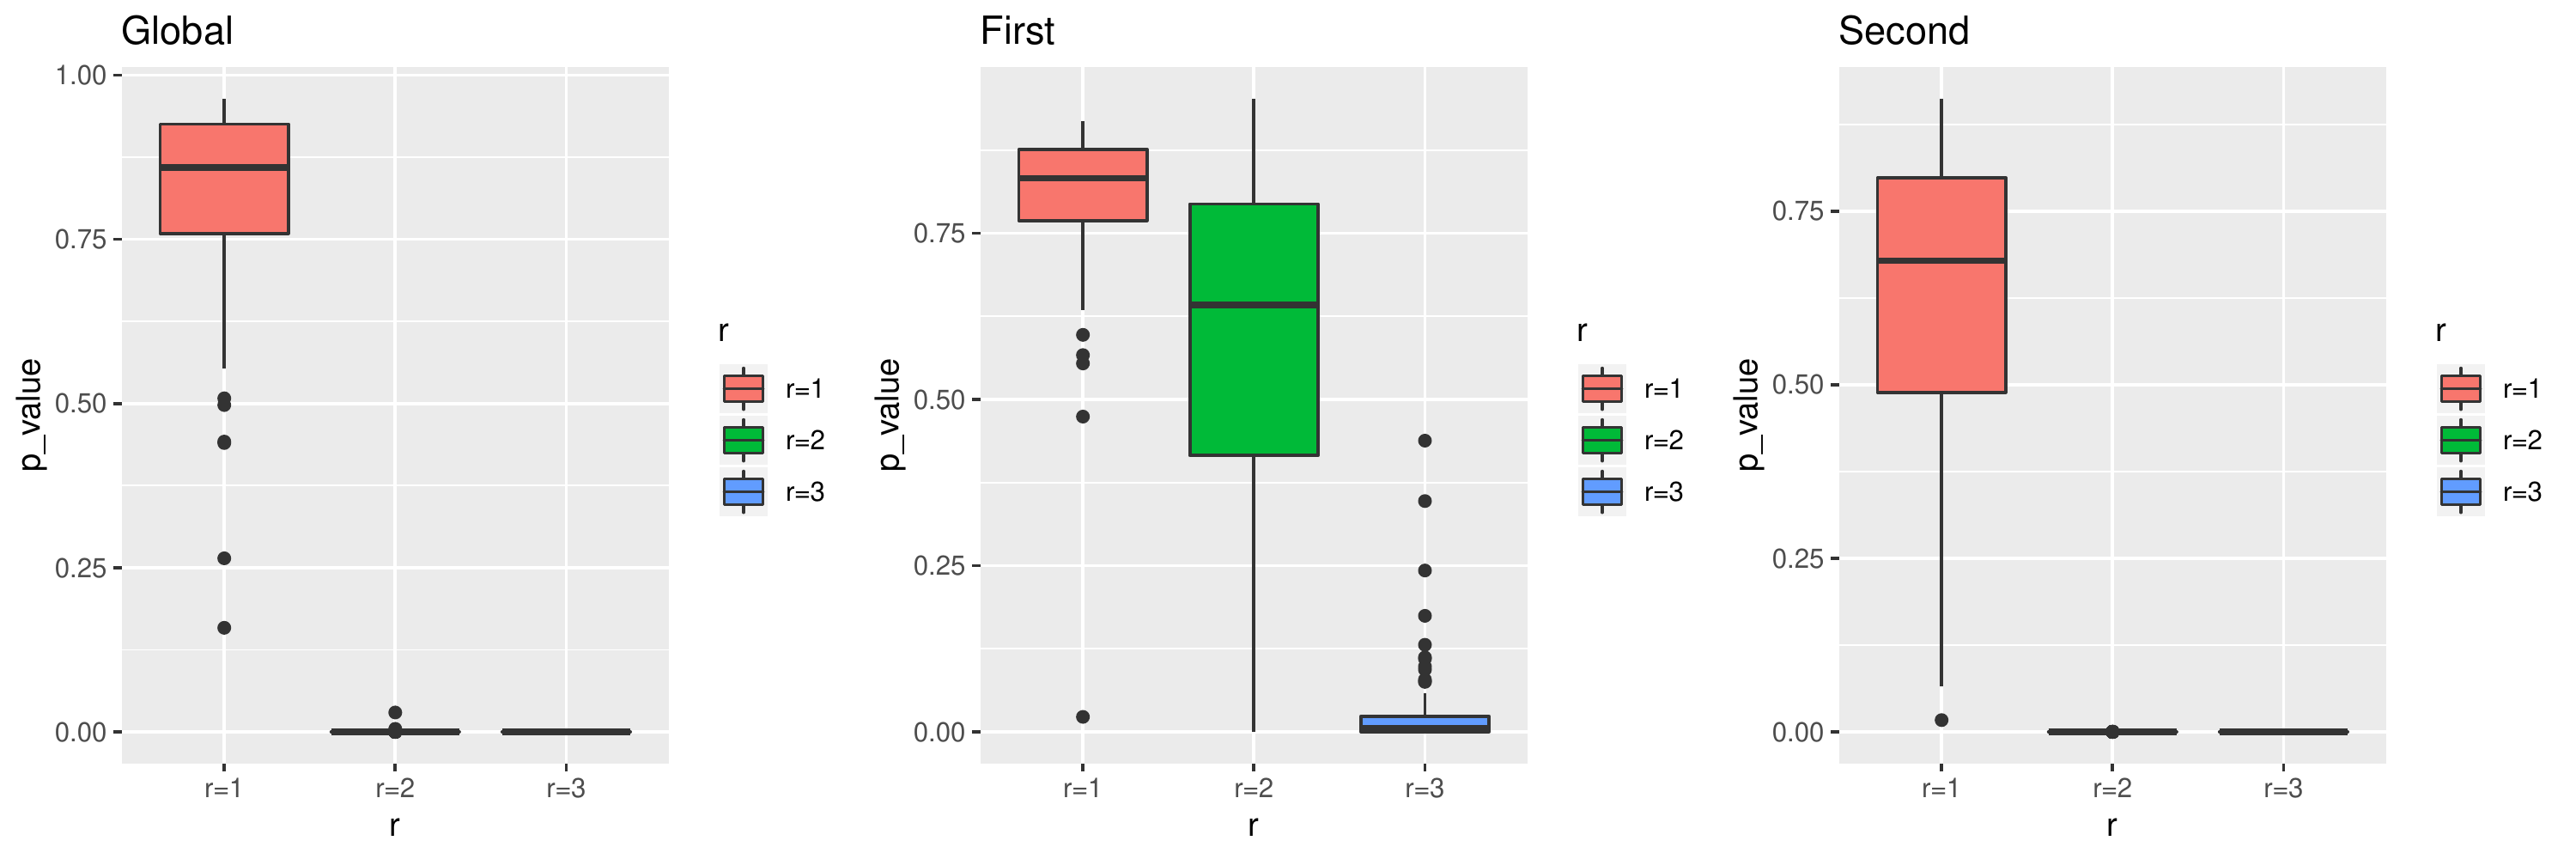}
%\end{center}
%\caption{Model 5: Histograms of the estimate of $d_0$ obtained over the intervals $(0,1)$ - global, %$(0,0.5)$ - first and $(0.5,1)$ - second. The true $d_{0,u}=2$ for $0<u<0.5$ and $d_{0,u} = 1$ for %$0.5<u<1$. }\label{fig:pvals_splitting_model_5}
%\end{figure}

%\begin{figure}[H]
%\begin{center}
%\includegraphics[scale=0.45]{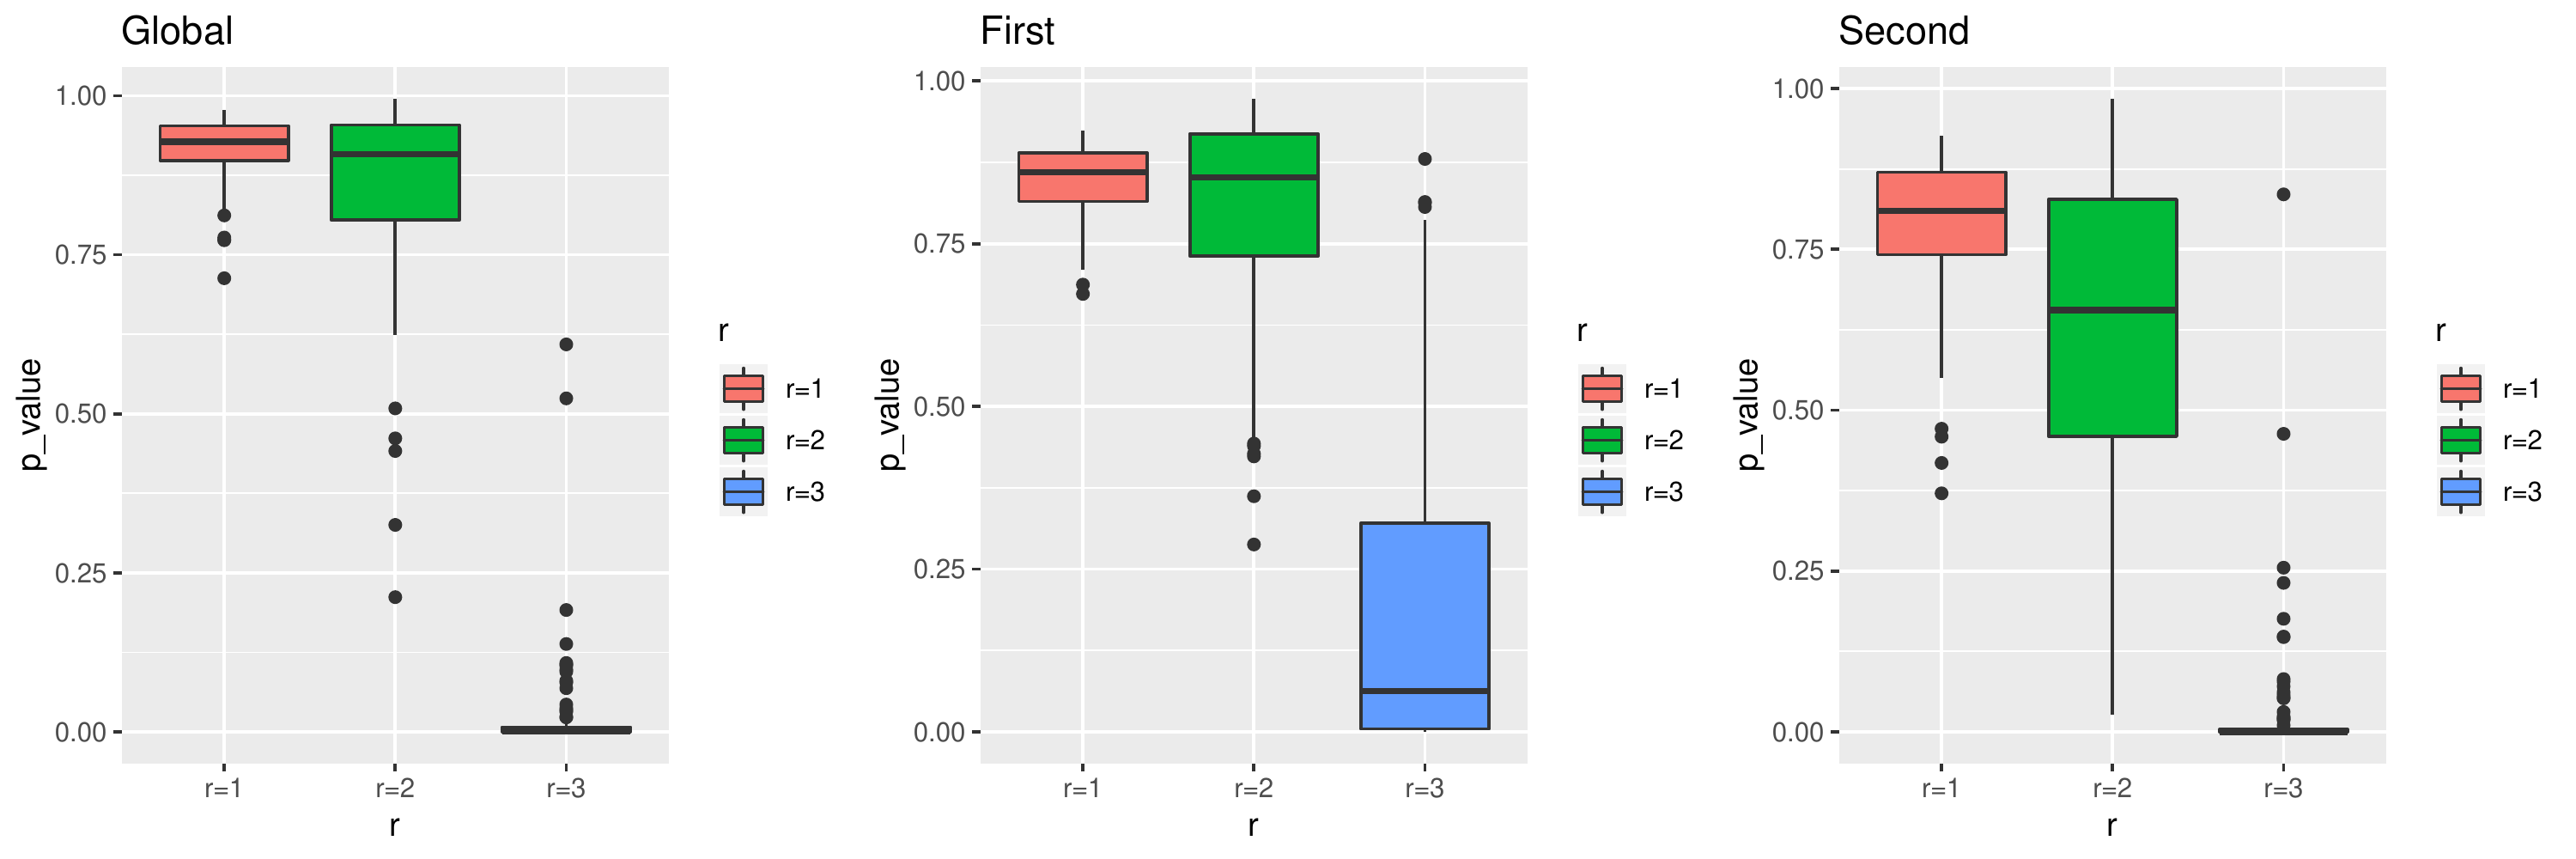}
%\end{center}
%\caption{Model 6: Histograms of the estimate of $d_0$ obtained over the intervals $(0,1)$ - global, %$(0,0.5)$ - first and $(0.5,1)$ - second. The true $d_{0,u}=3$ for $0<u<0.5$ and $d_{0,u} = 2$ for %$0.5<u<1$. }\label{fig:model_6}
%\end{figure}

%%%%%%%%%%%%%%%%%%%%%%%%%%%%%%%%%%%%%%%%%%%%%%%%%%%%%%%%%%%%%%%%%%%%%%%%%%%%%%%%%%%%%%%%%
%%%%%%%%%%%%%%%%%%%%%%%%%%%%%%%%%%%%%%%%%%%%%%%%%%%%%%%%%%%%%%%%%%%%%%%%%%%%%%%%%%%%%%%%%%
% Section 6.2
\subsection{Figures for Section \ref{s:simulation_subspace}}

% % Model 2
%
\begin{figure}[H]
\minipage{0.24\textwidth}
  \includegraphics[width=\linewidth]{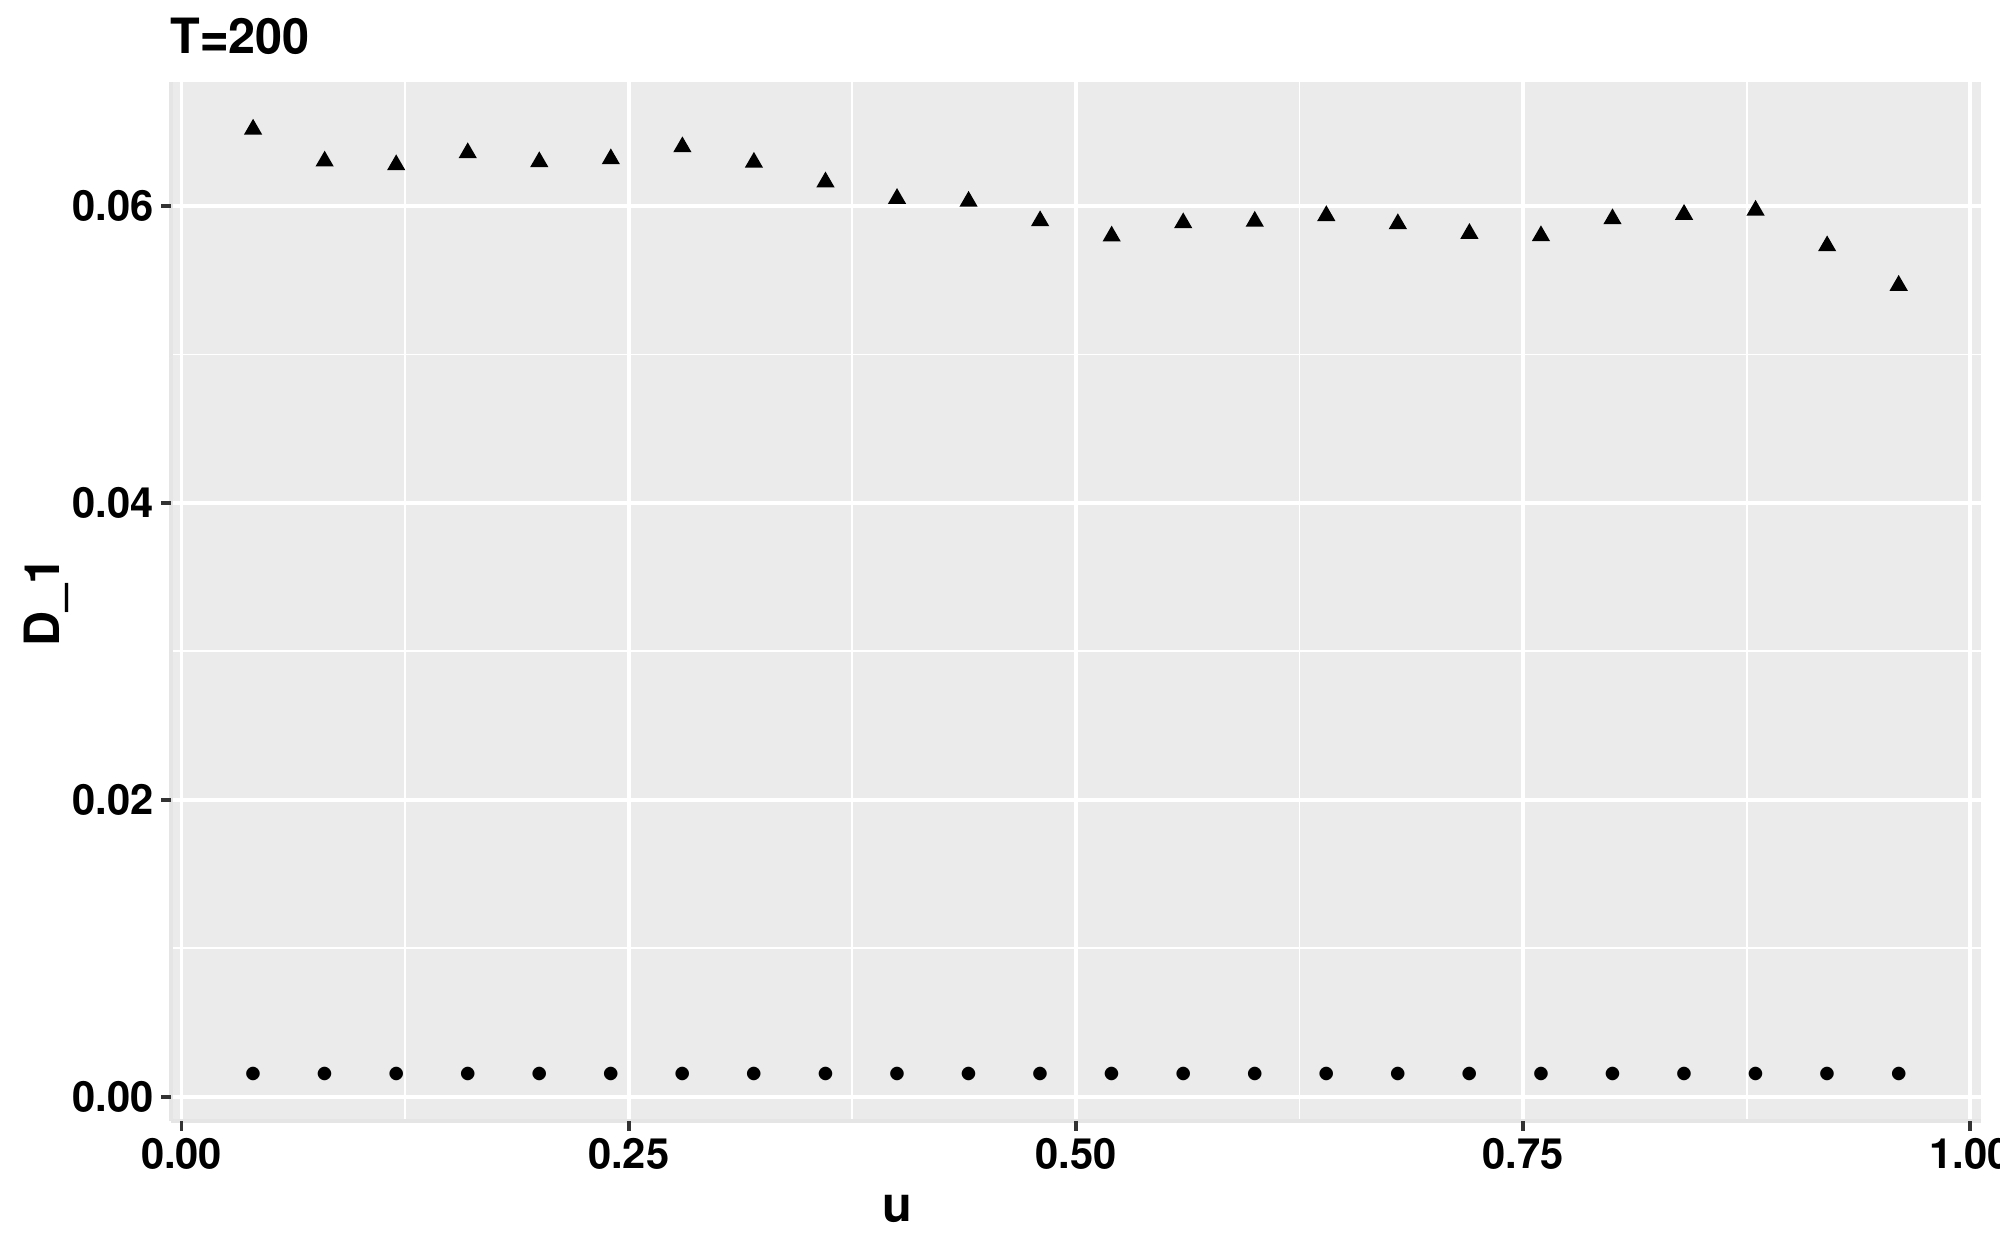}
\endminipage\hfill
\minipage{0.24\textwidth}
  \includegraphics[width=\linewidth]{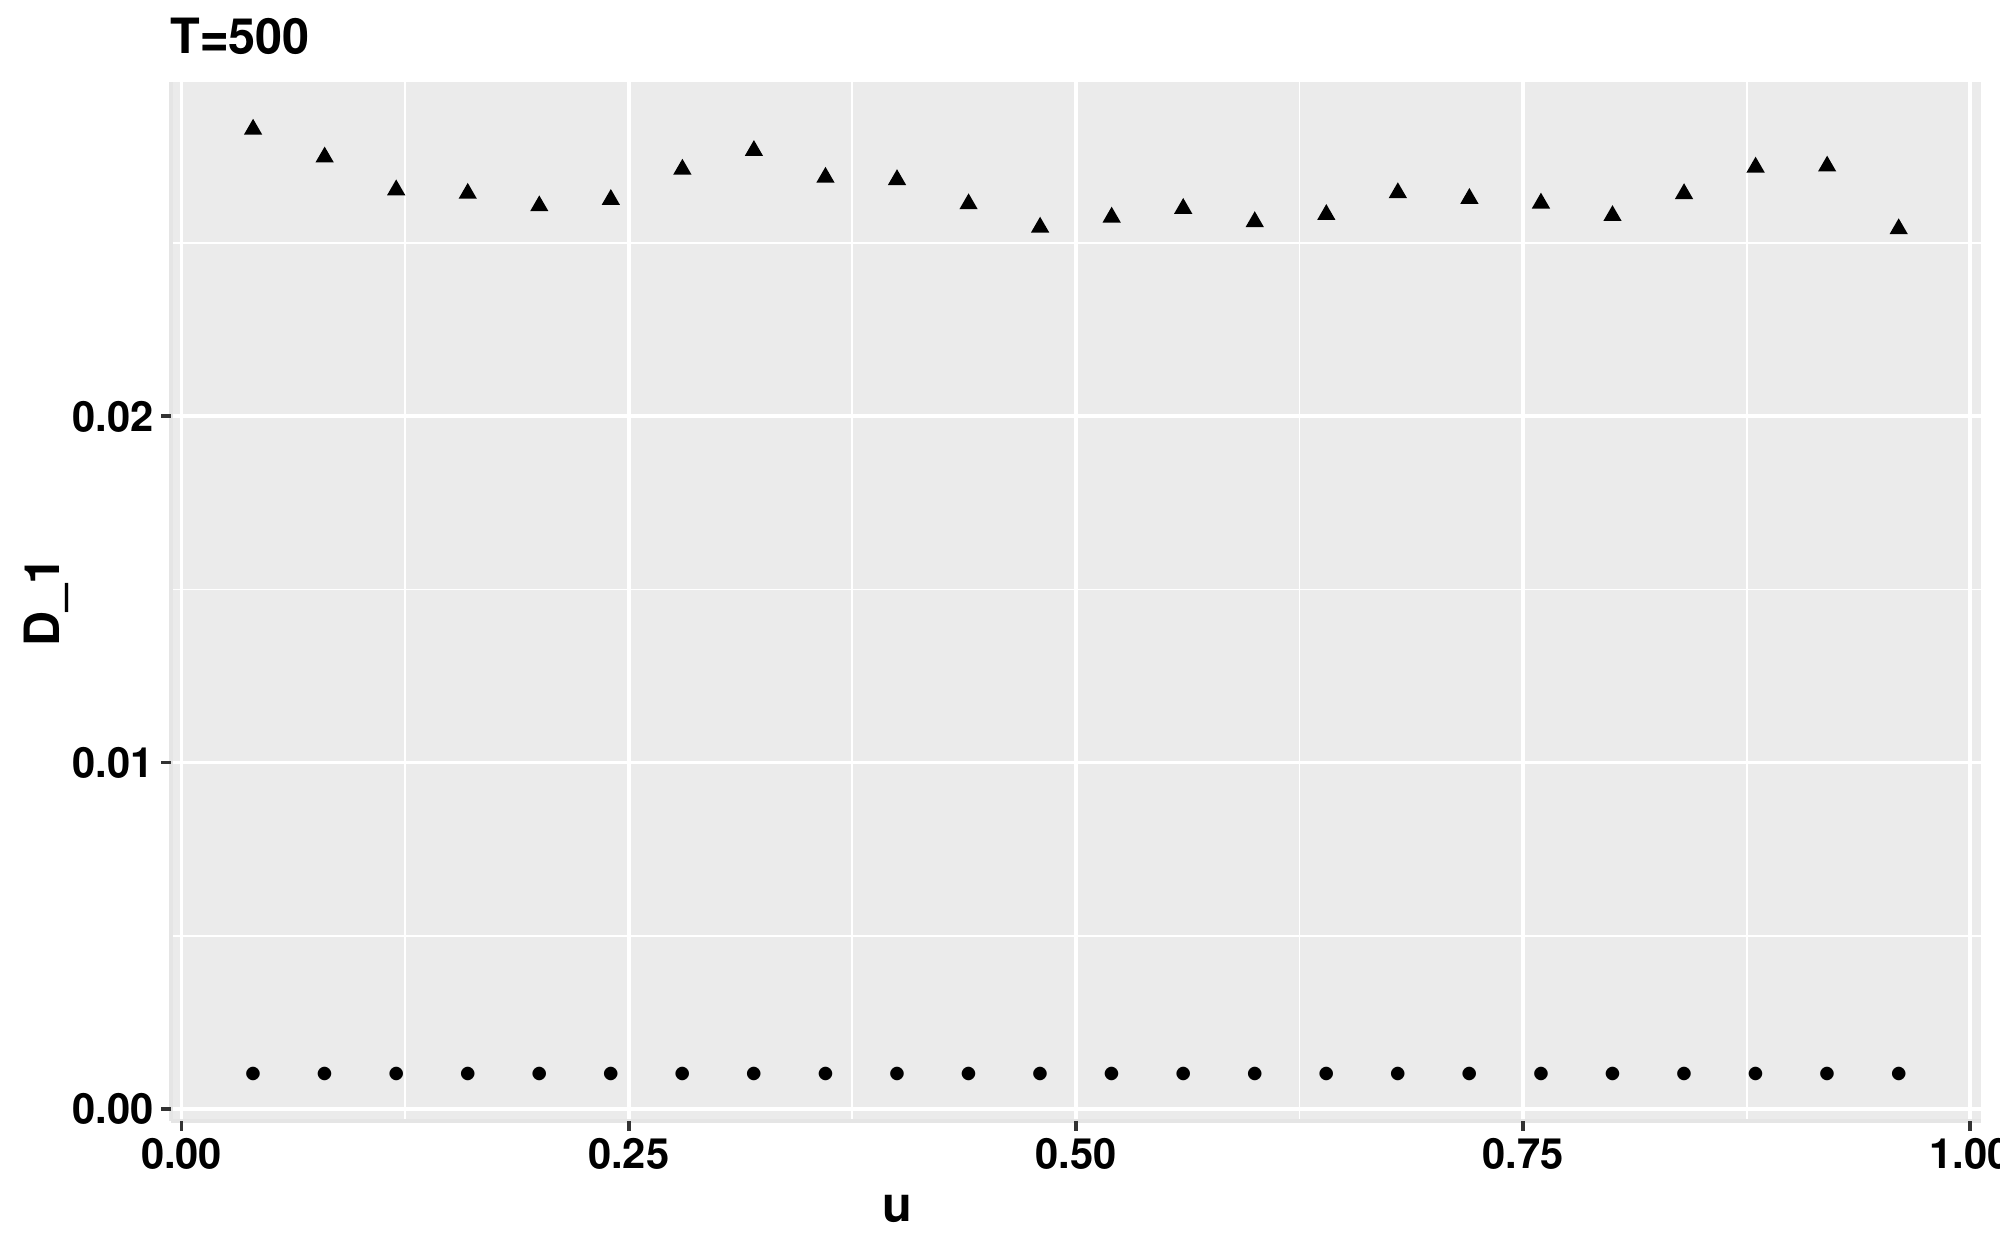}
\endminipage\hfill
\minipage{0.24\textwidth}%
  \includegraphics[width=\linewidth]{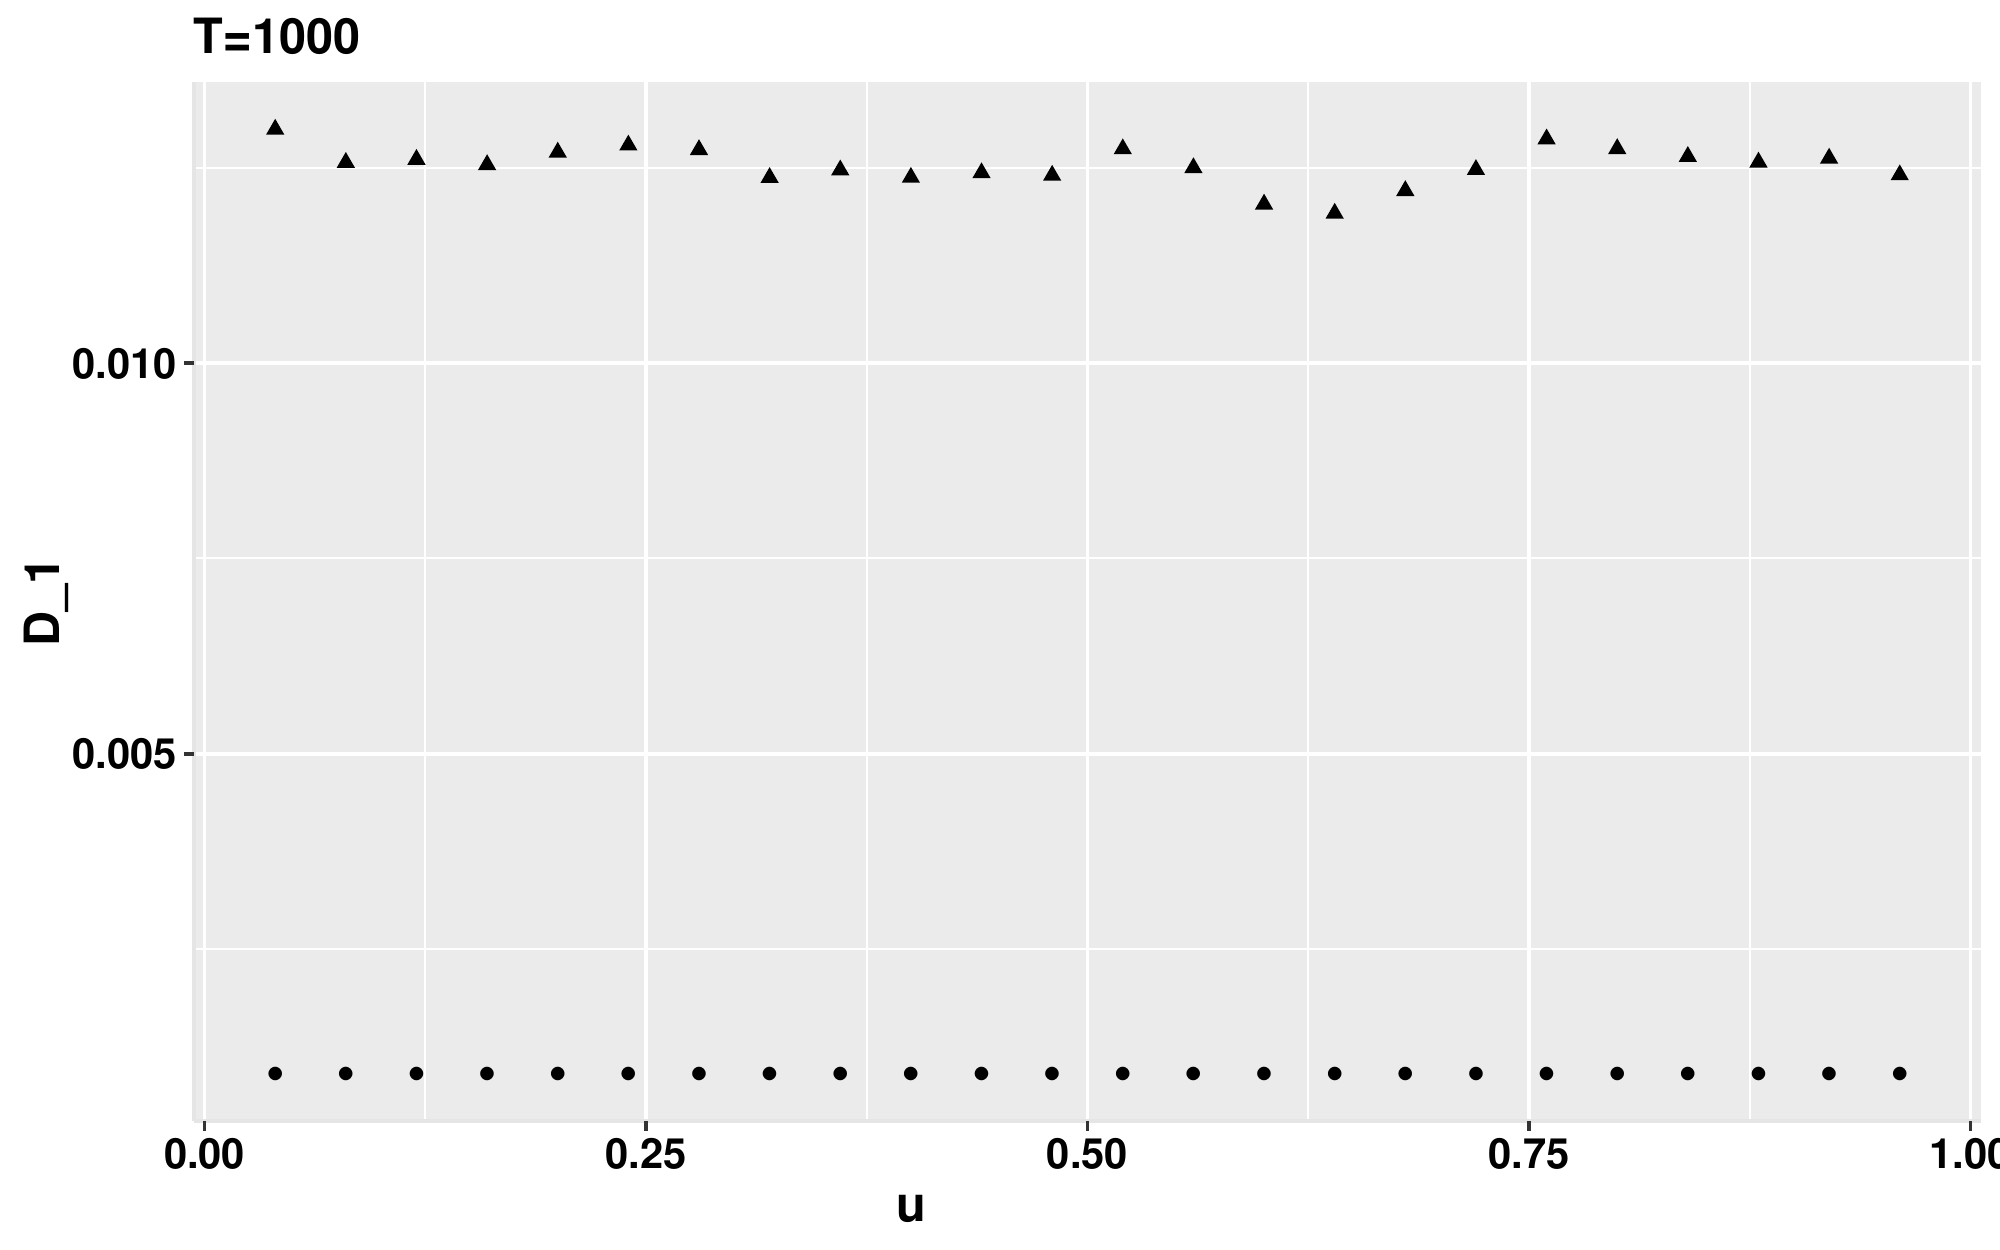}
\endminipage
\minipage{0.24\textwidth}%
  \includegraphics[width=\linewidth]{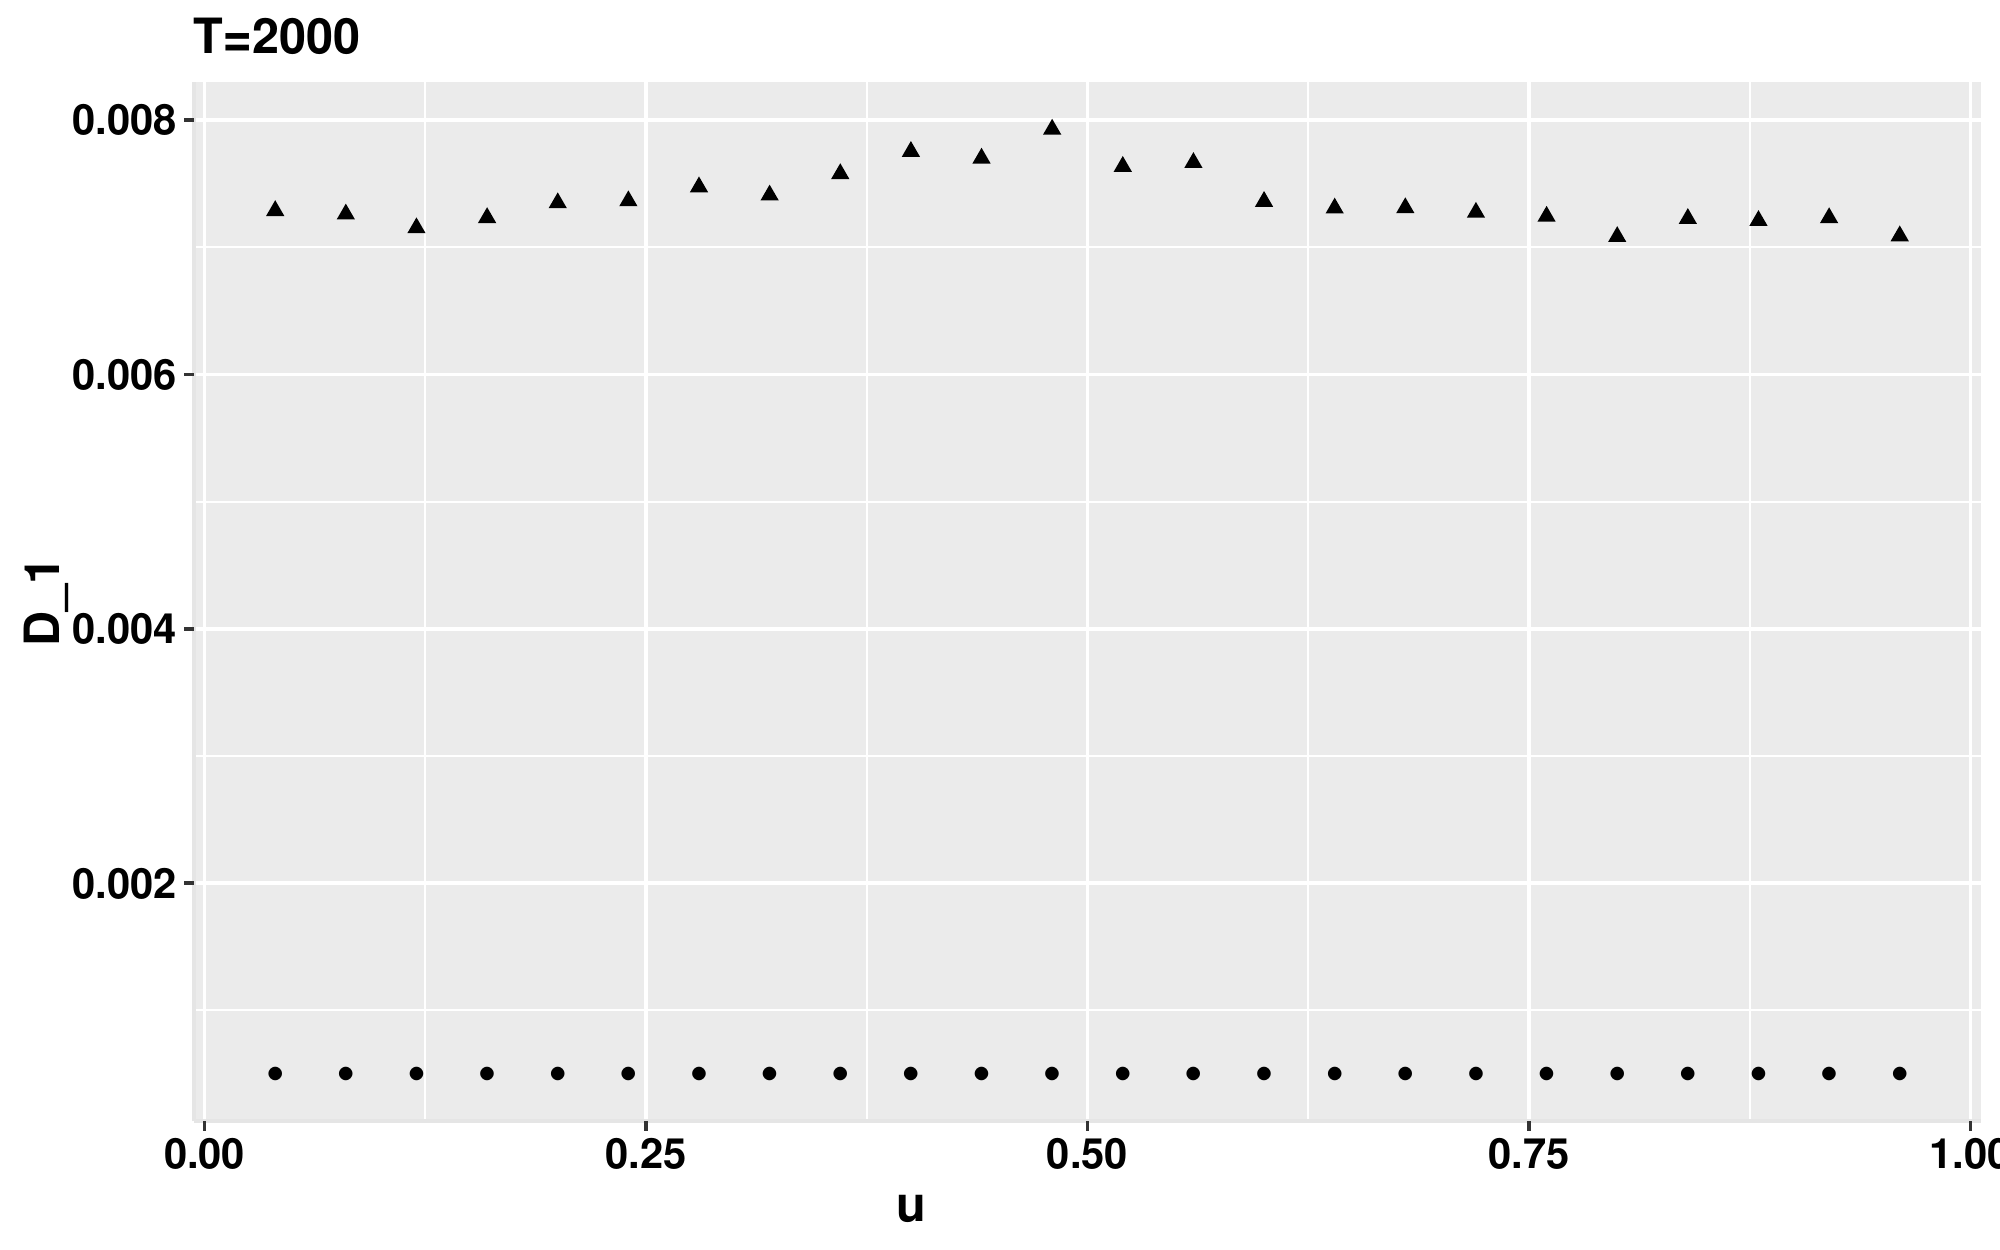}
\endminipage
% \caption{Model 1: Plot of $D_1(\widehat{B}_{1} (u) )$ against $u$ for the competing methods DSSA %and VC and several sample sizes.  } \label{fig:m1_compare_d1}
\end{figure}
\vspace{-0.5cm}
\begin{figure}[H]
\minipage{0.24\textwidth}
  \includegraphics[width=\linewidth]{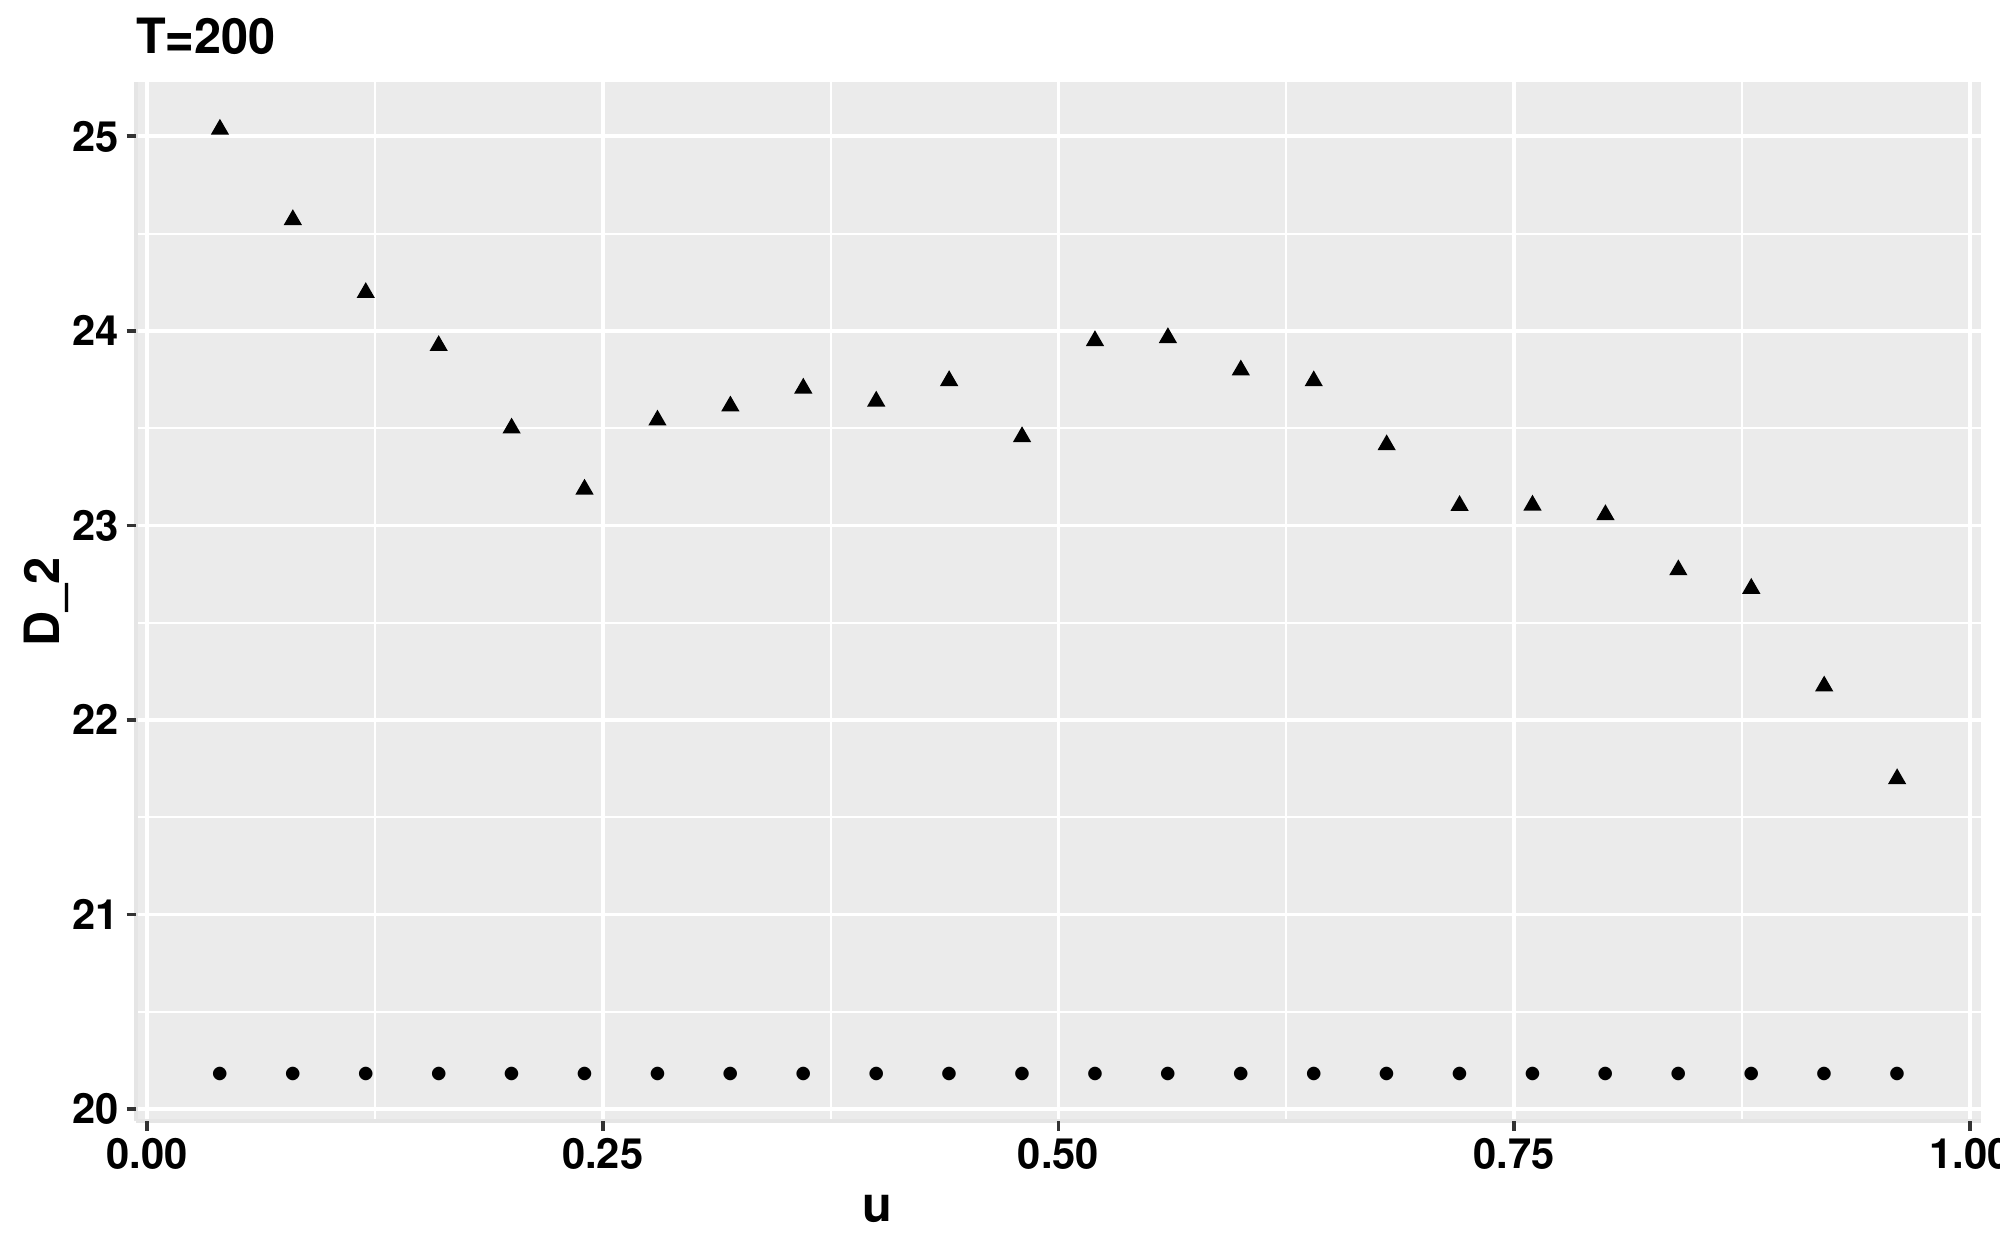}
\endminipage\hfill
\minipage{0.24\textwidth}
  \includegraphics[width=\linewidth]{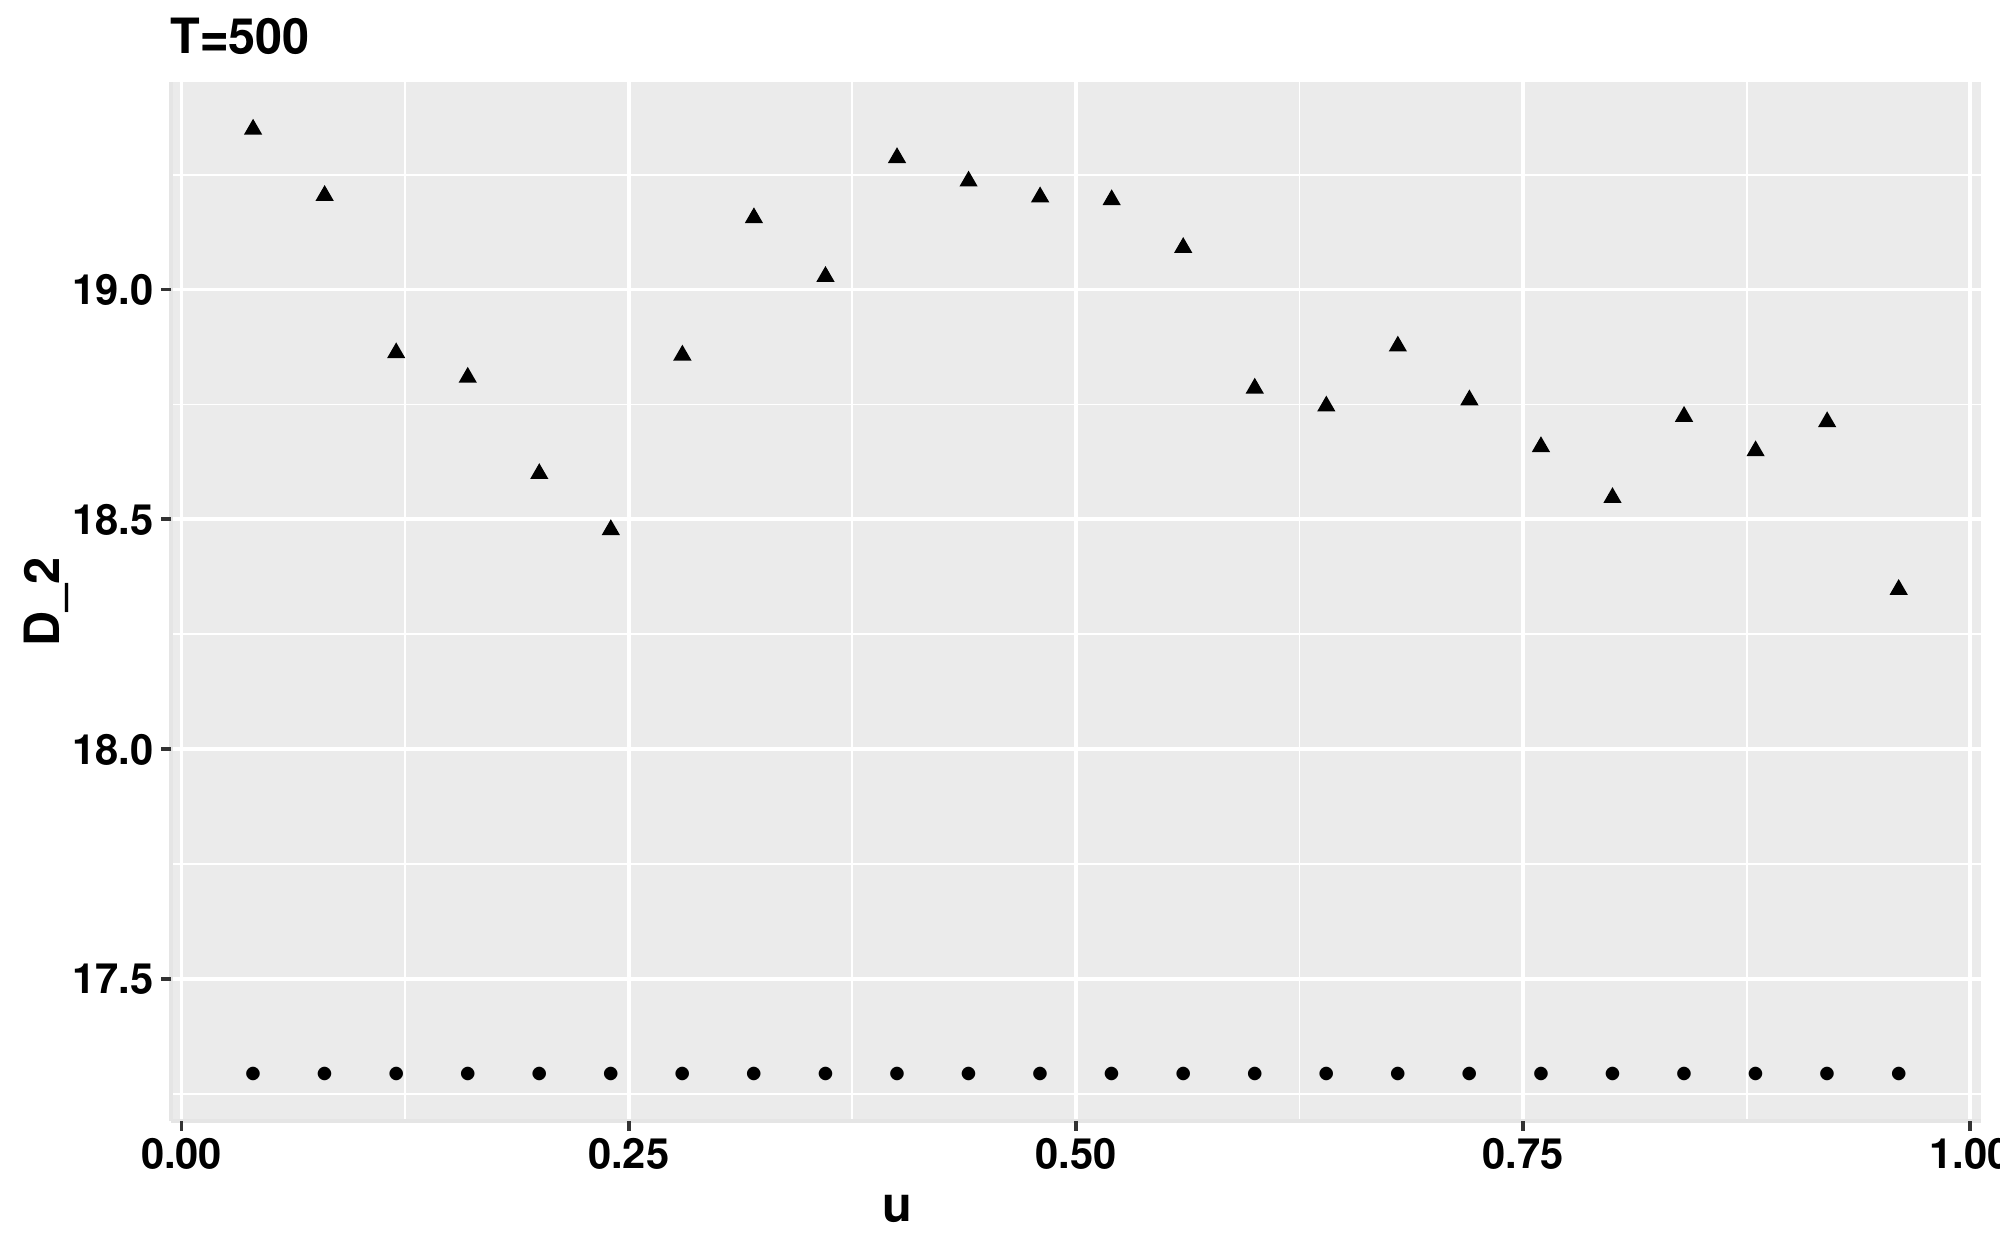}
\endminipage\hfill
\minipage{0.24\textwidth}%
  \includegraphics[width=\linewidth]{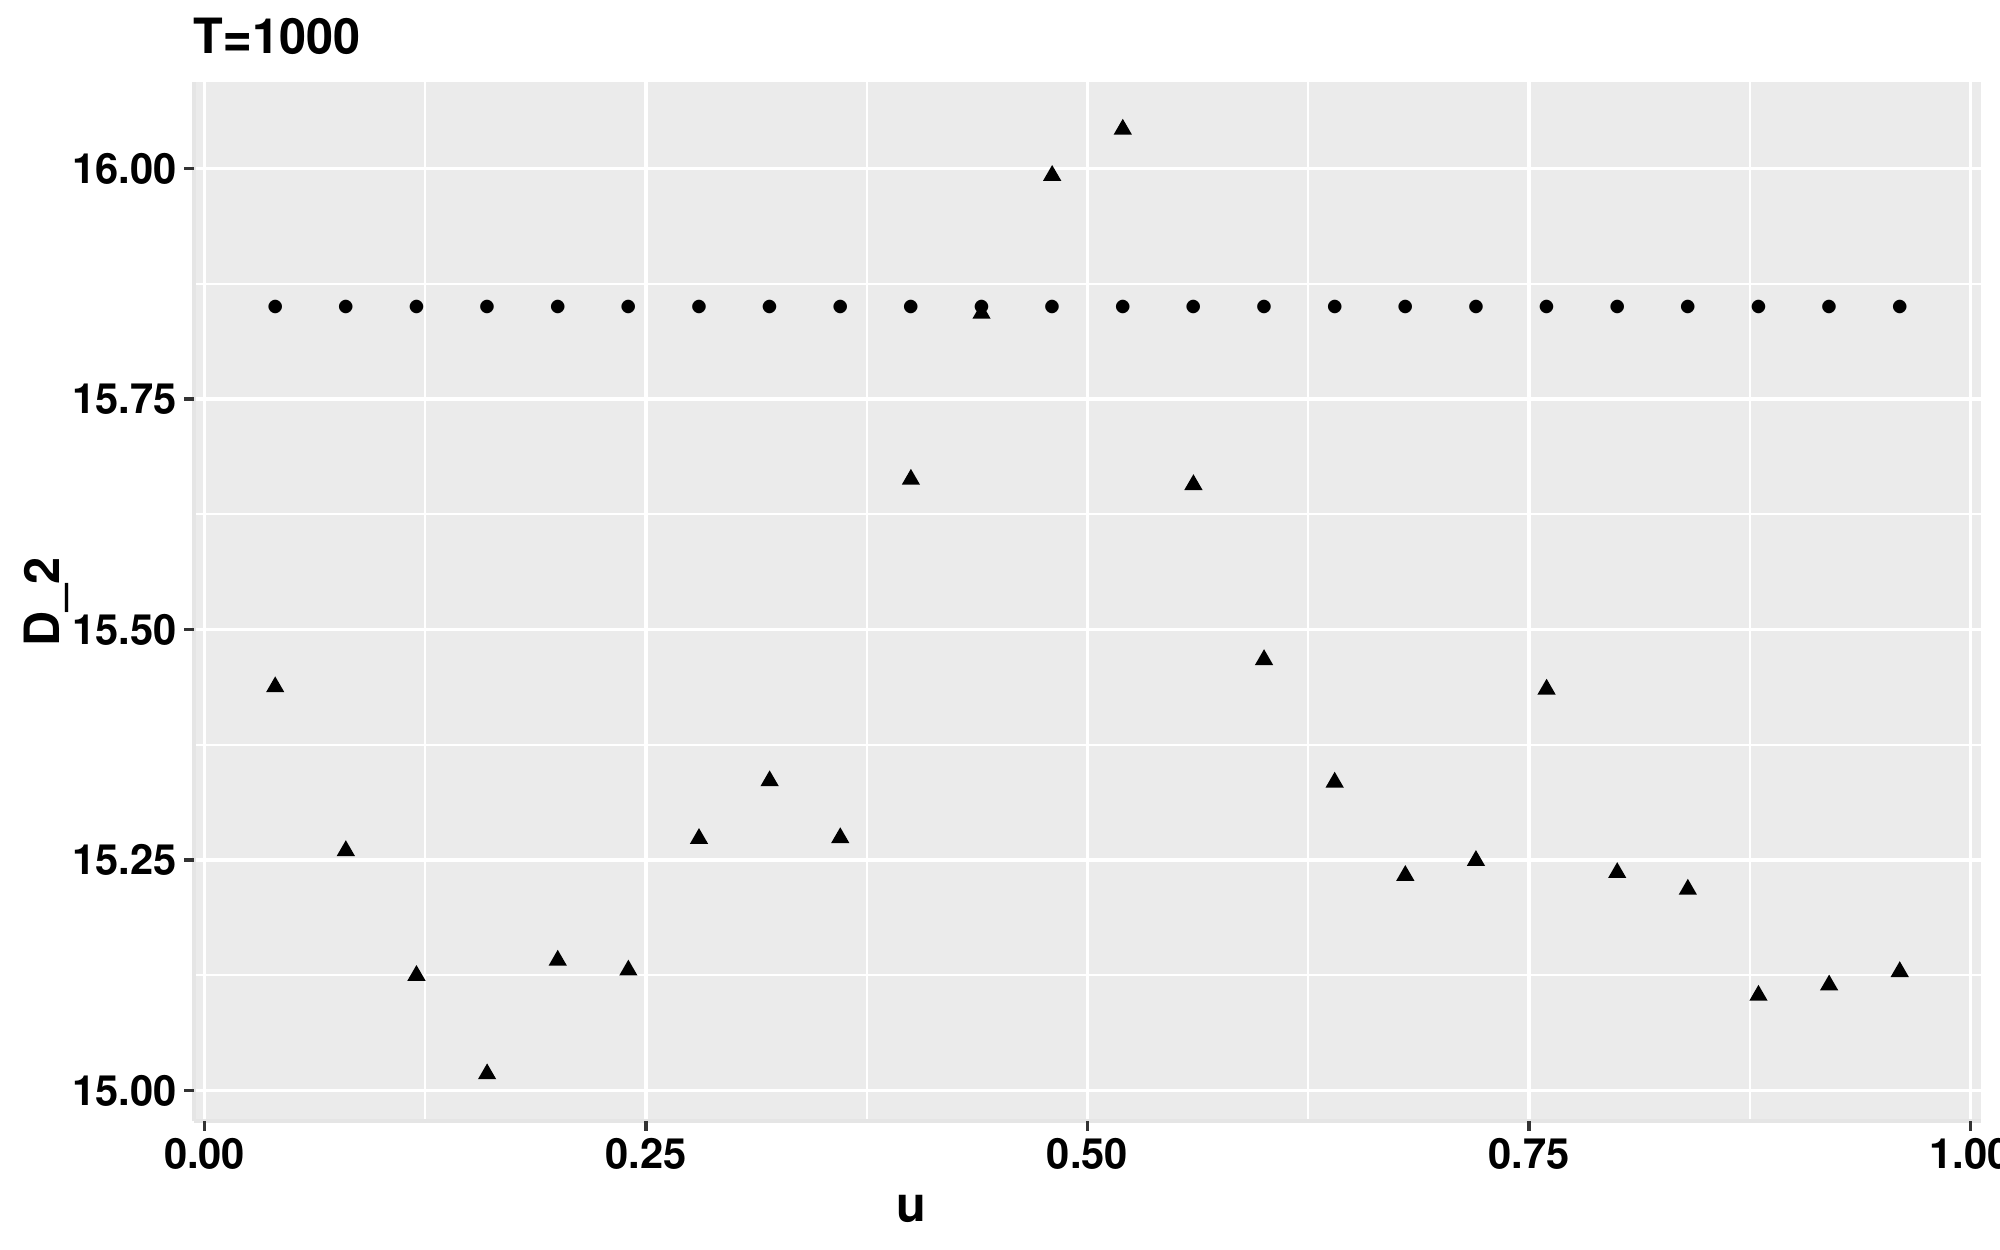}
\endminipage
\minipage{0.24\textwidth}%
  \includegraphics[width=\linewidth]{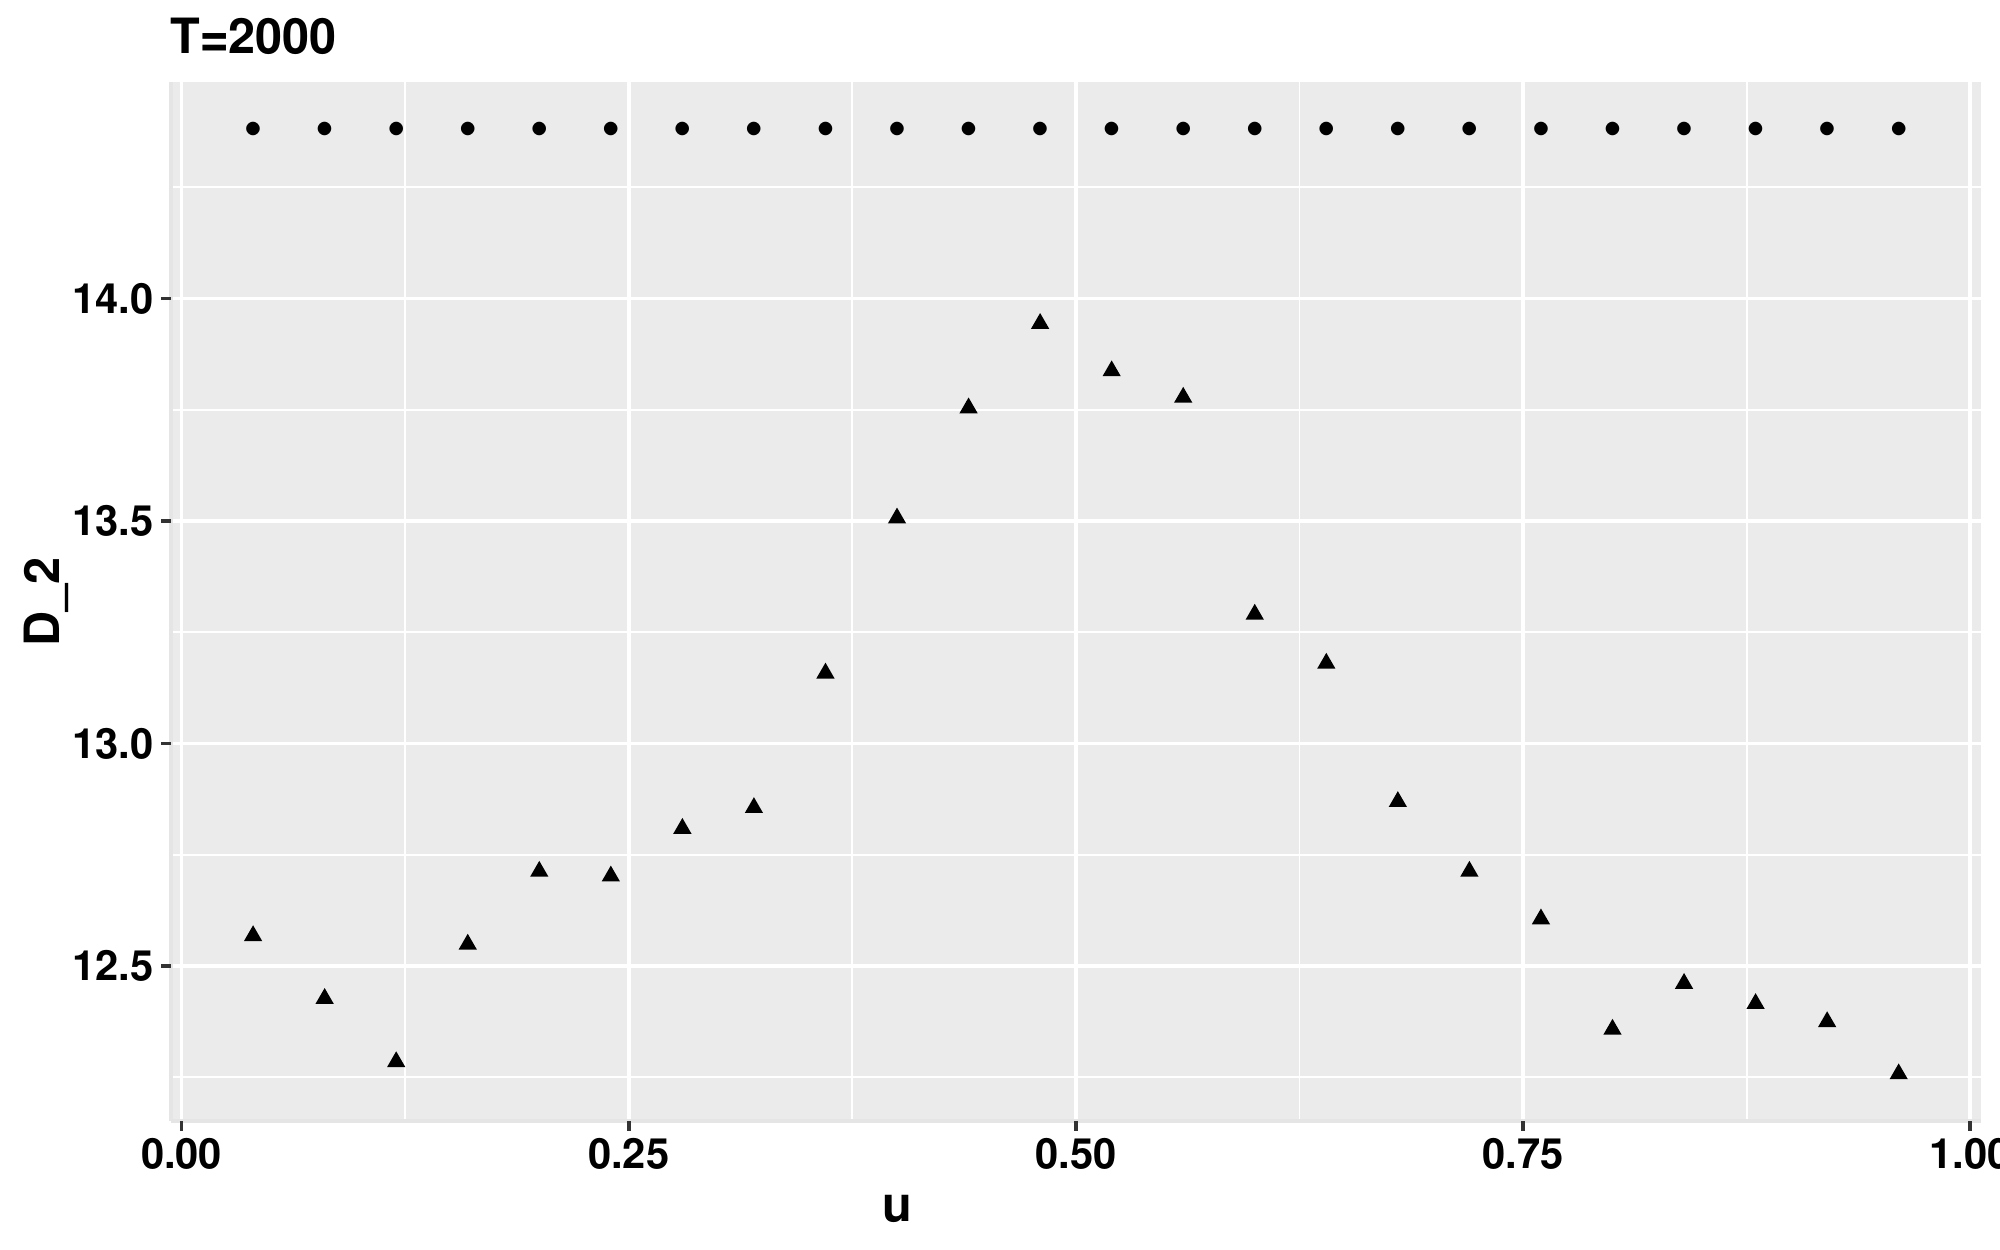}
\endminipage
\caption{Model 2 - Top:  Plot of $D_1(\widehat{B}_{1} (u) )$ against $u$ for the competing methods DSSA and VC and several sample sizes. VC (avg.) in triangles in squares and DSSA in solid circles. Bottom: Analogous plot but with measure $D_2(\widehat{B}_{1} (u) )$ against $u$.  } \label{fig:m2_compare_d1d2}
\end{figure}

\begin{figure}[H]
\minipage{0.24\textwidth}
  \includegraphics[width=\linewidth]{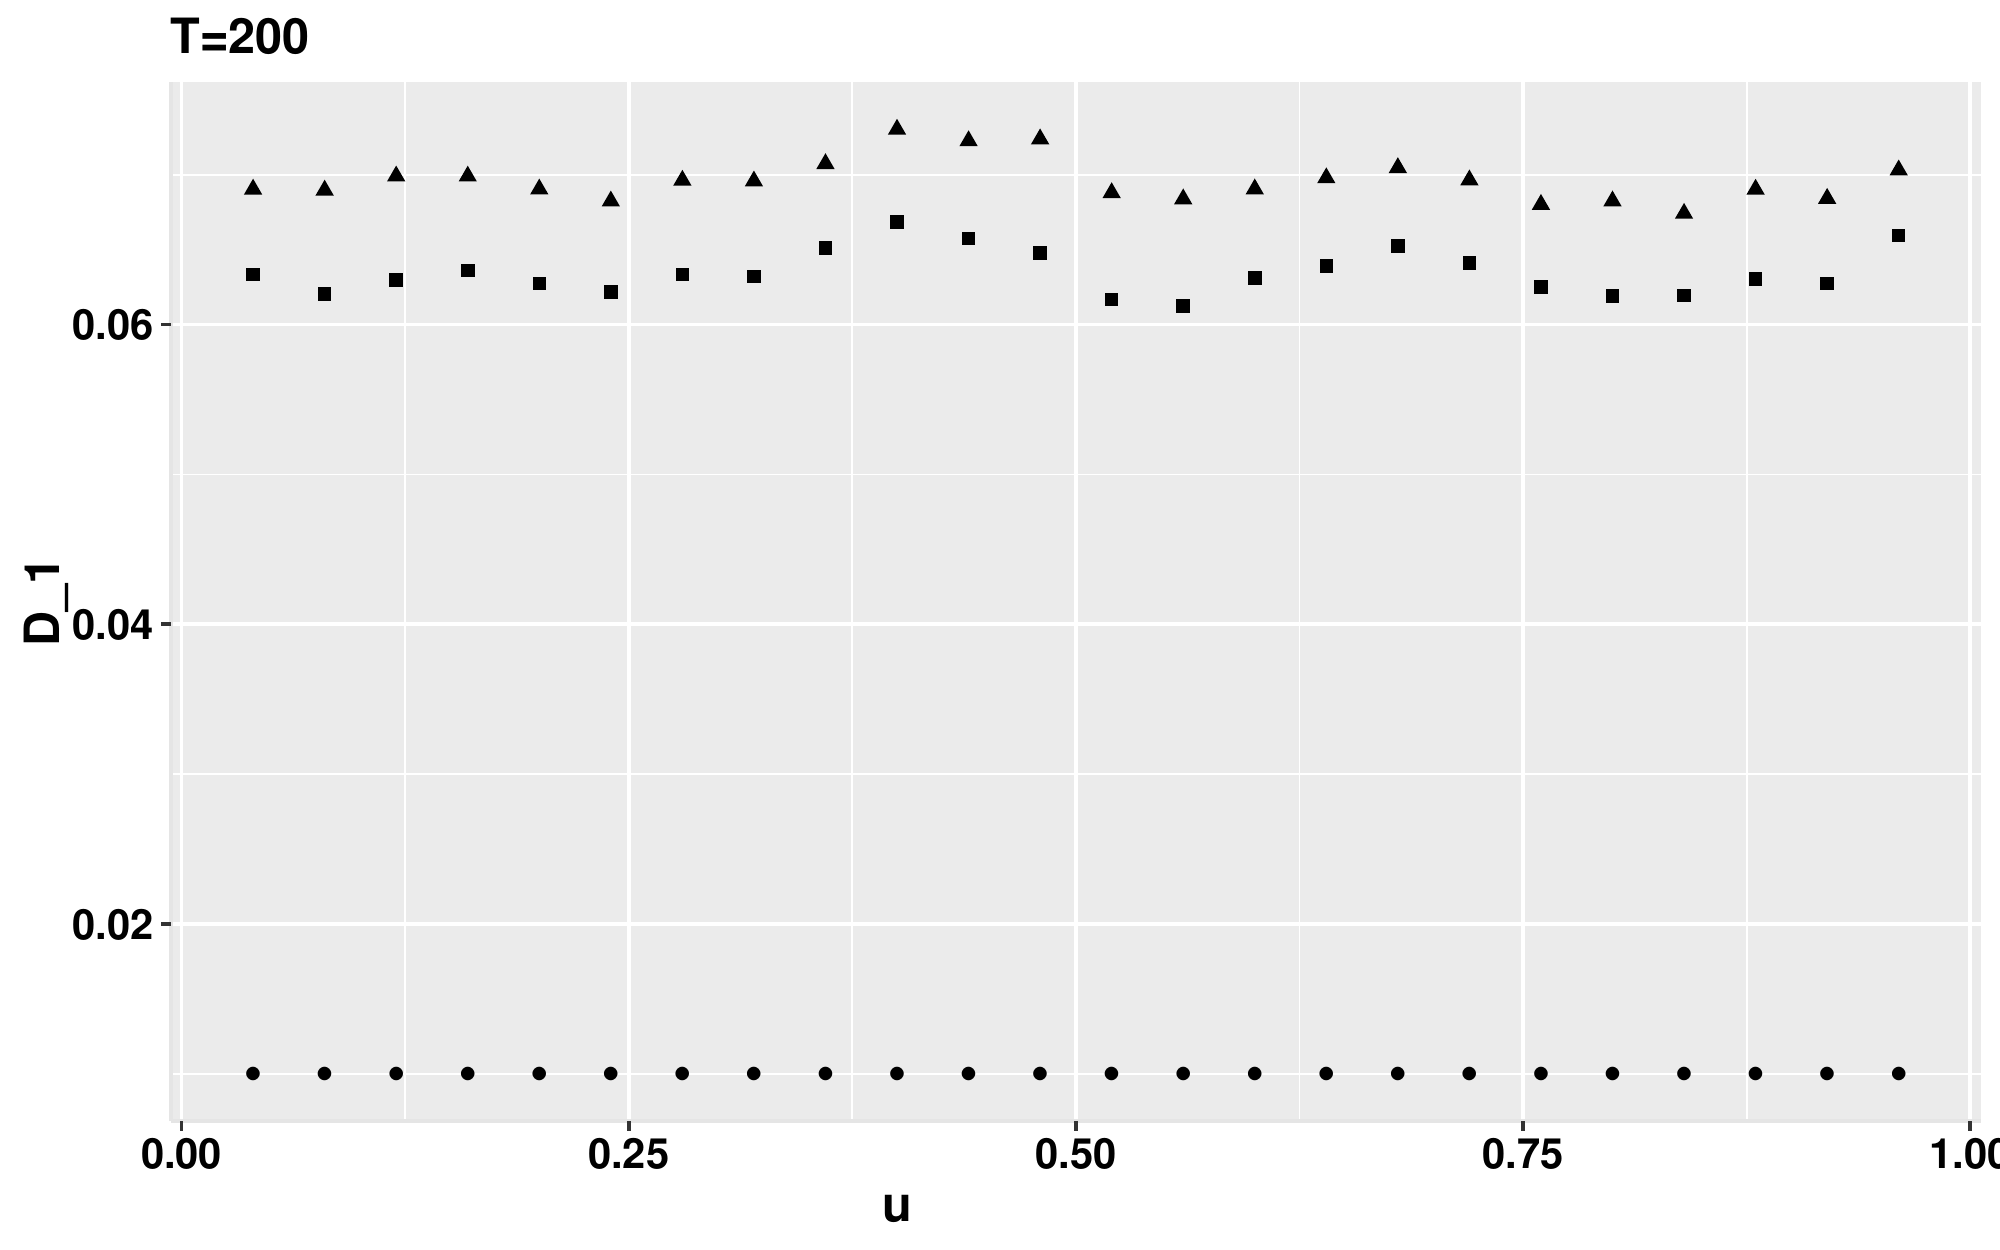}
\endminipage\hfill
\minipage{0.24\textwidth}
  \includegraphics[width=\linewidth]{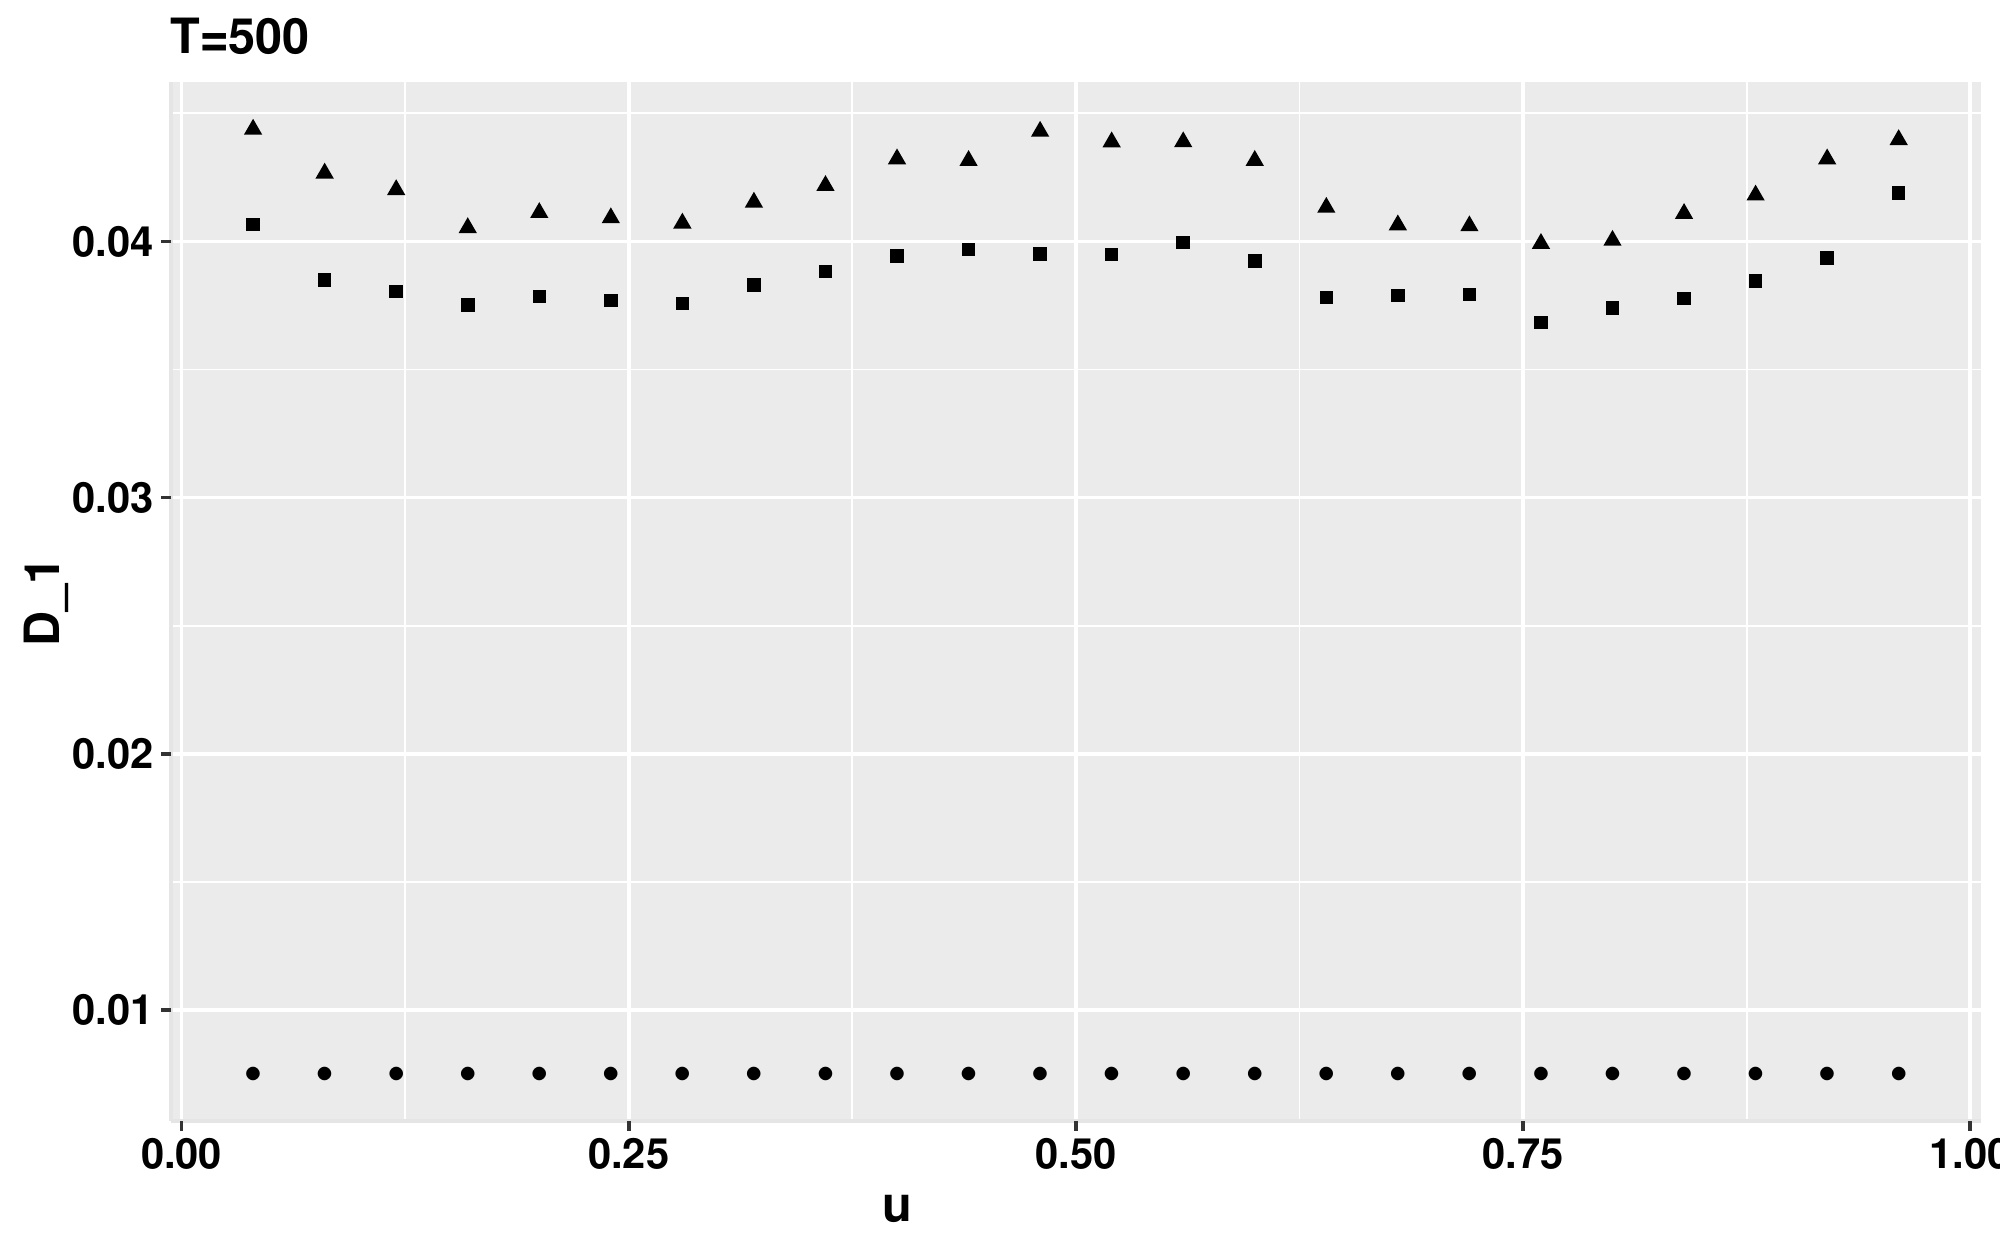}
\endminipage\hfill
\minipage{0.24\textwidth}%
  \includegraphics[width=\linewidth]{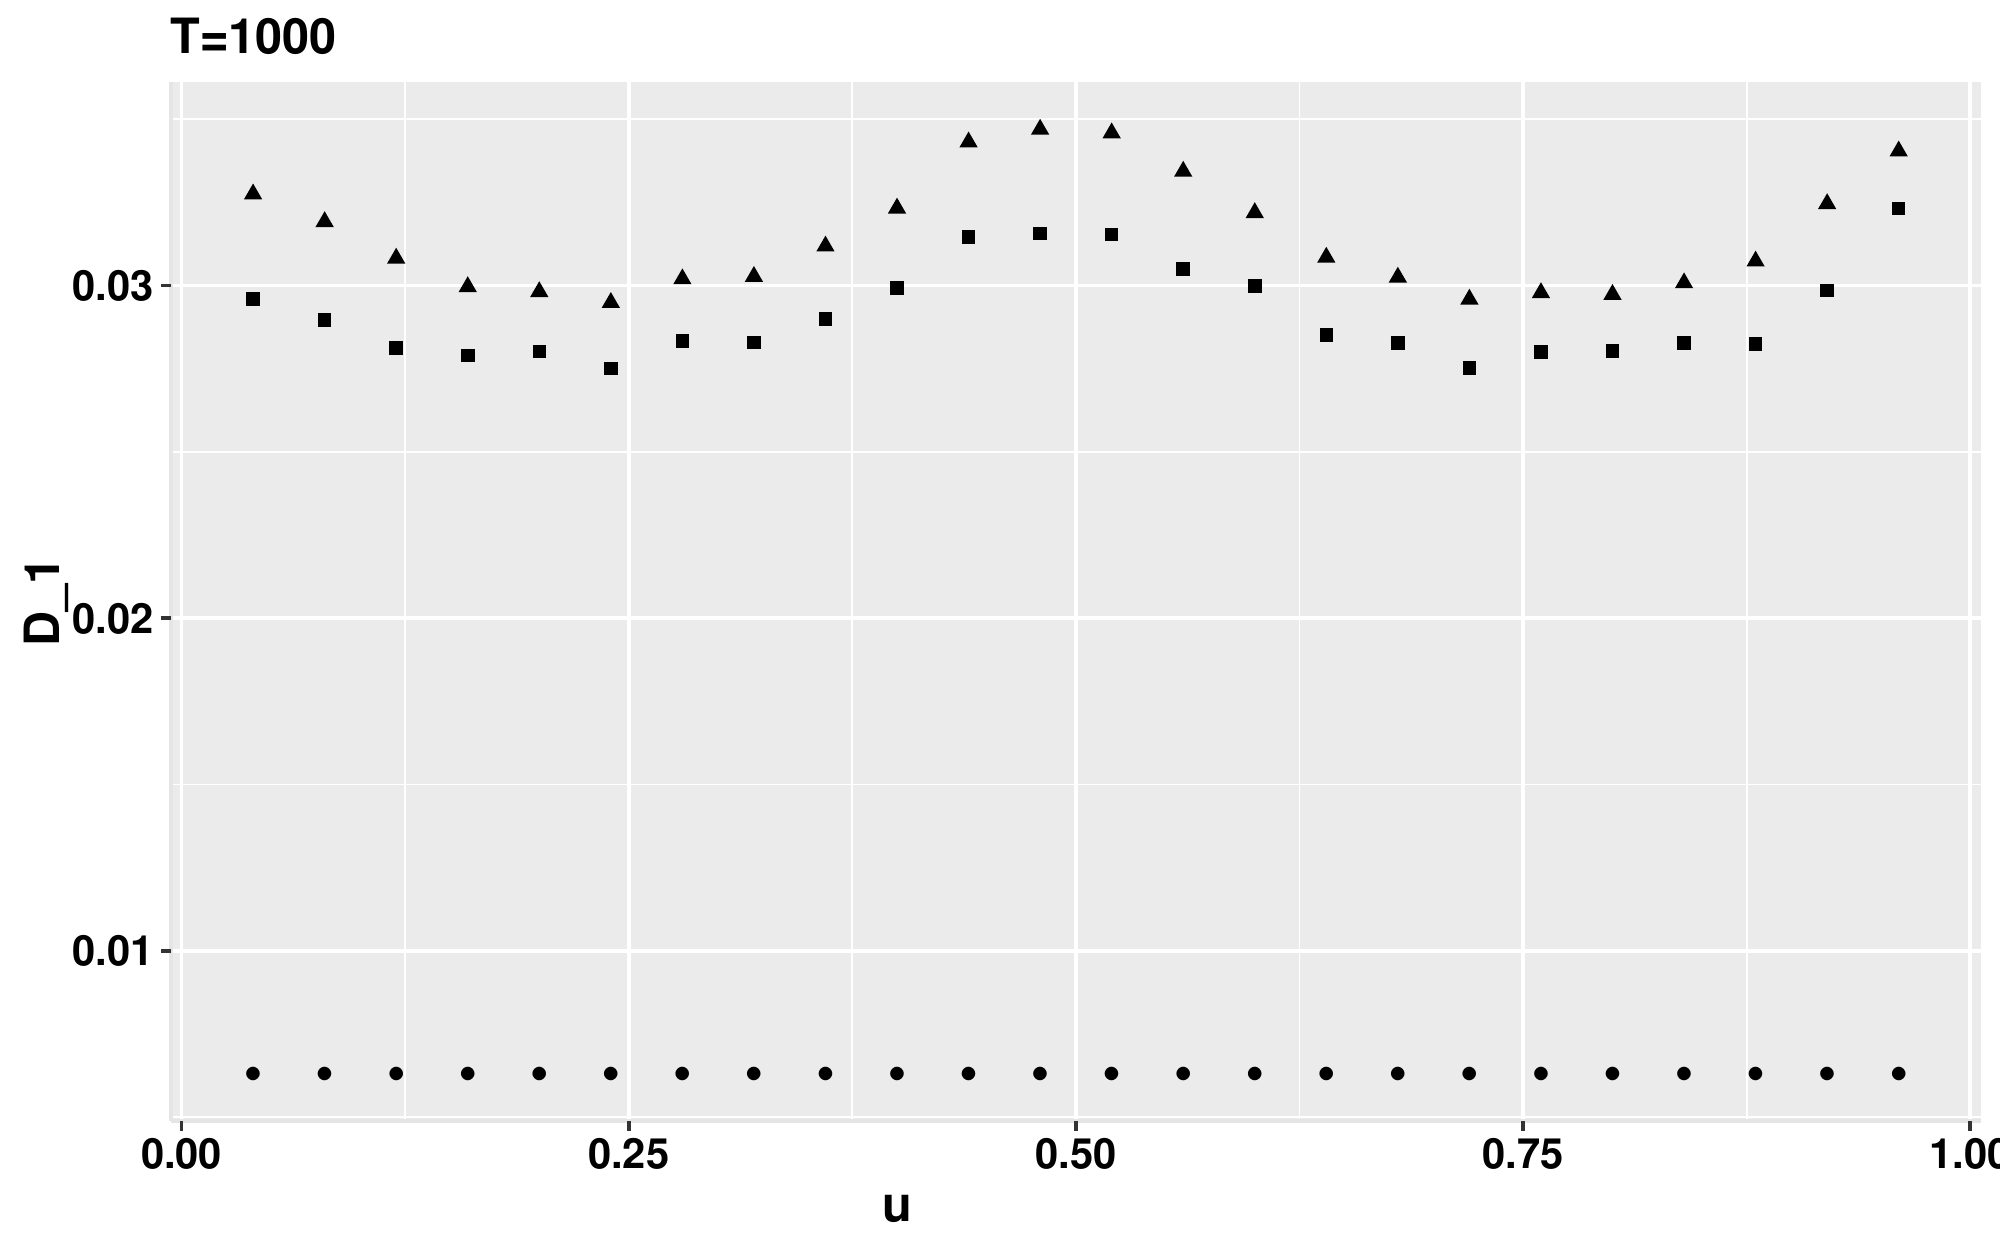}
\endminipage
\minipage{0.24\textwidth}%
  \includegraphics[width=\linewidth]{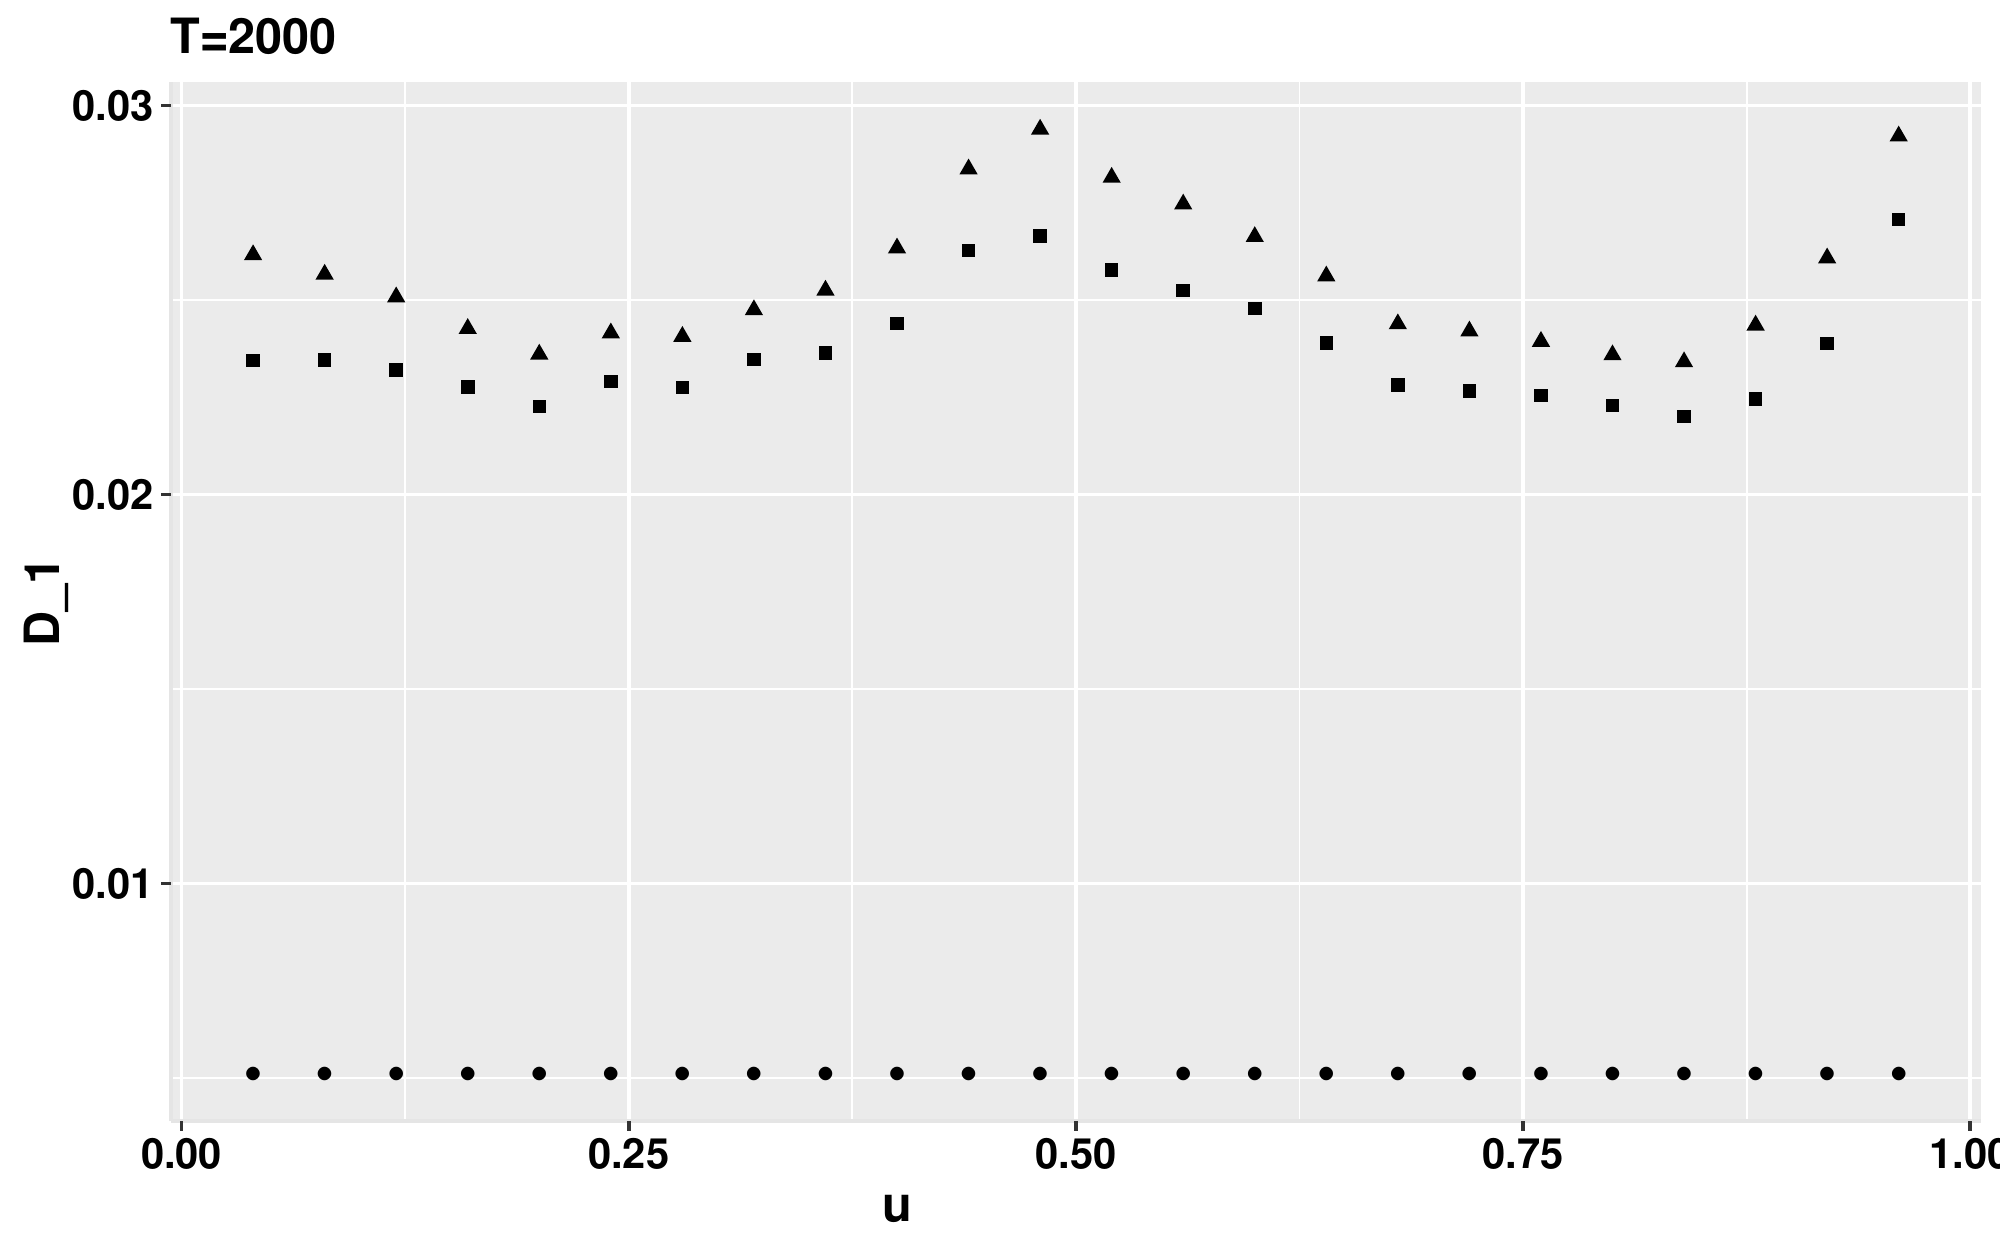}
\endminipage
% \caption{Model 1: Plot of $D_1(\widehat{B}_{1} (u) )$ against $u$ for the competing methods DSSA %and VC and several sample sizes.  } \label{fig:m1_compare_d1}
\end{figure}
\vspace{-0.5cm}
\begin{figure}[H]
\minipage{0.24\textwidth}
  \includegraphics[width=\linewidth]{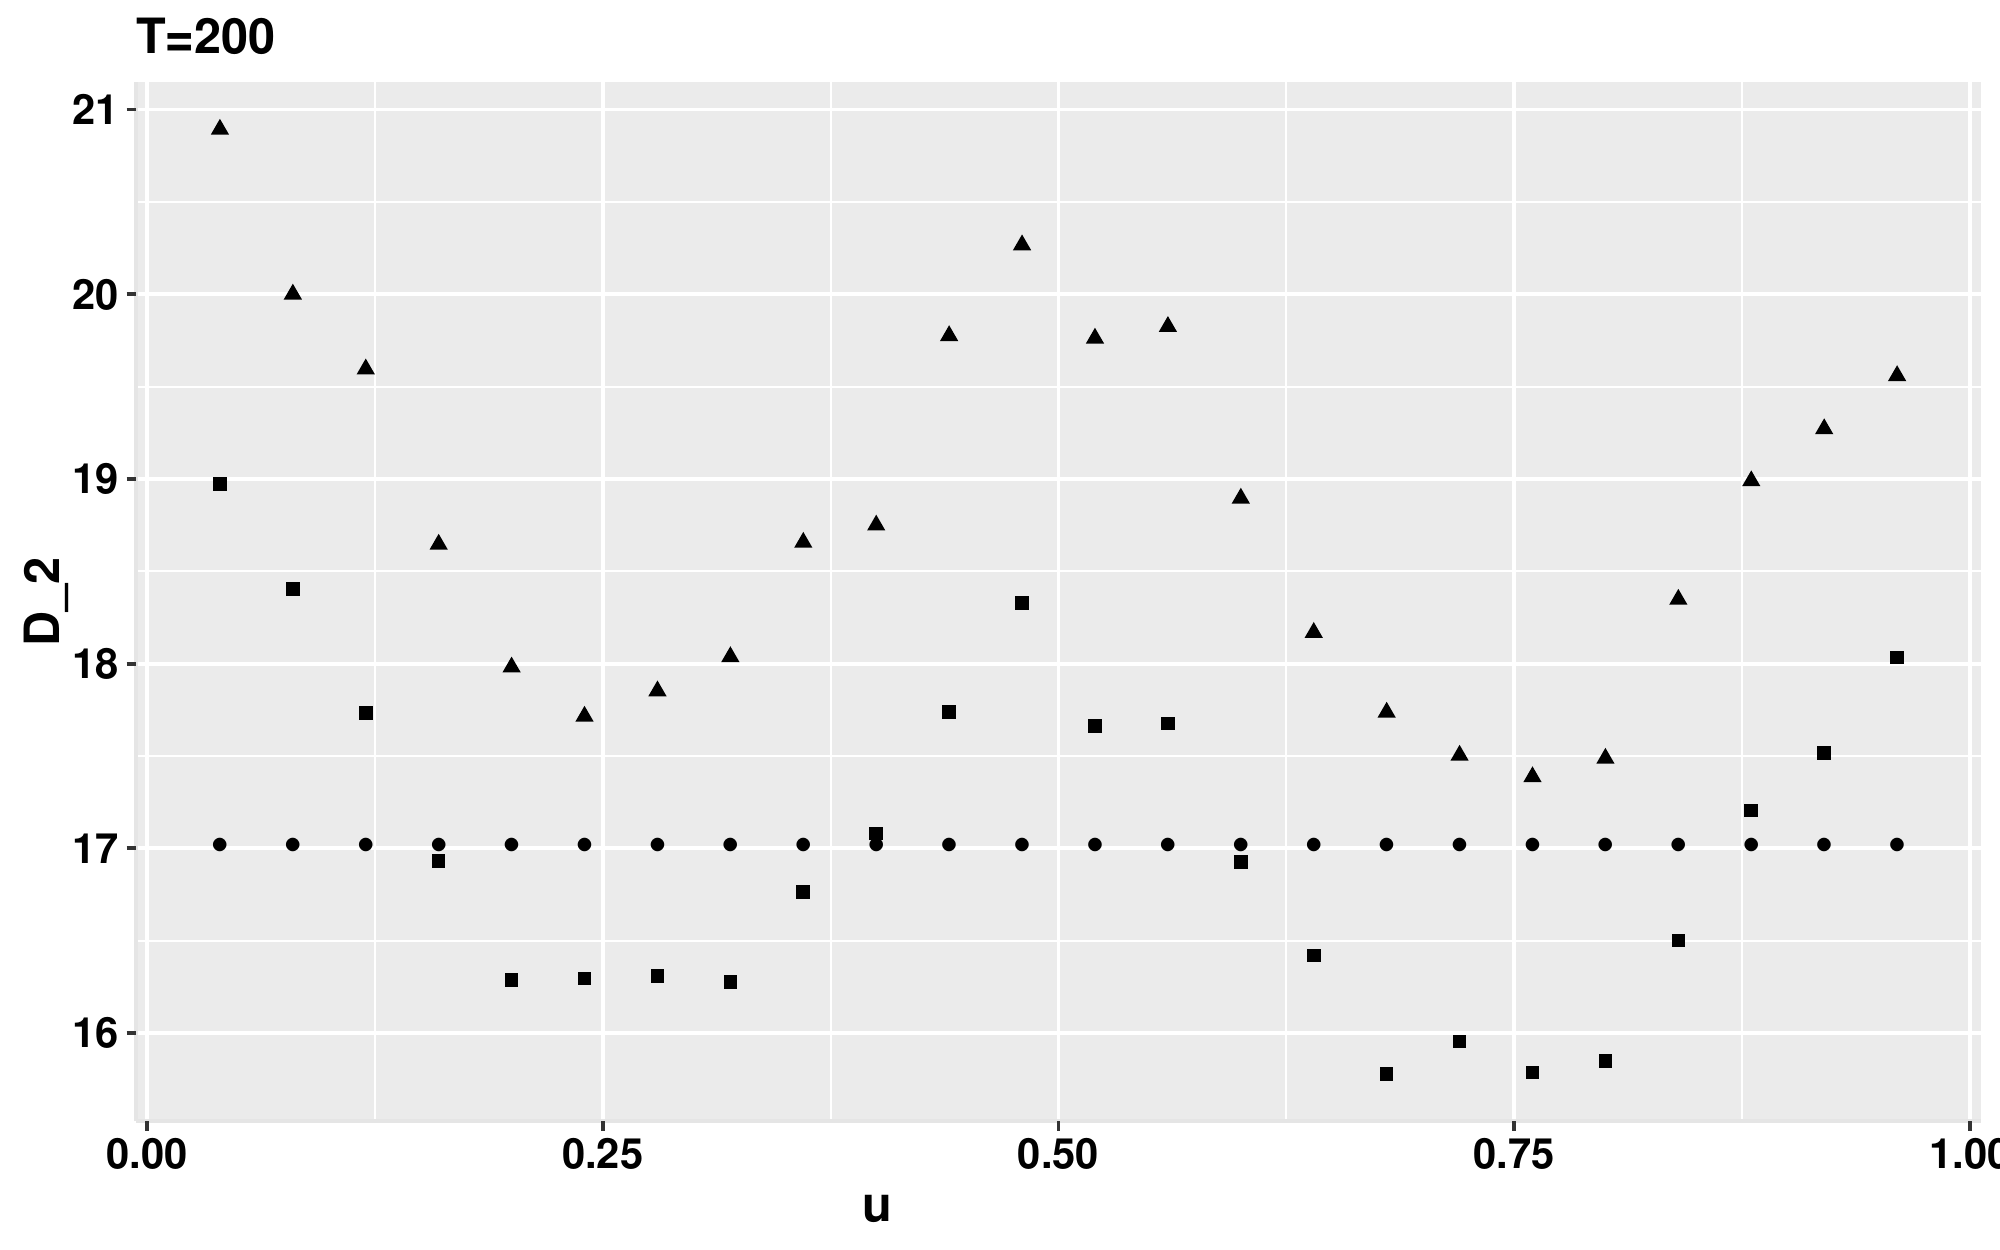}
\endminipage\hfill
\minipage{0.24\textwidth}
  \includegraphics[width=\linewidth]{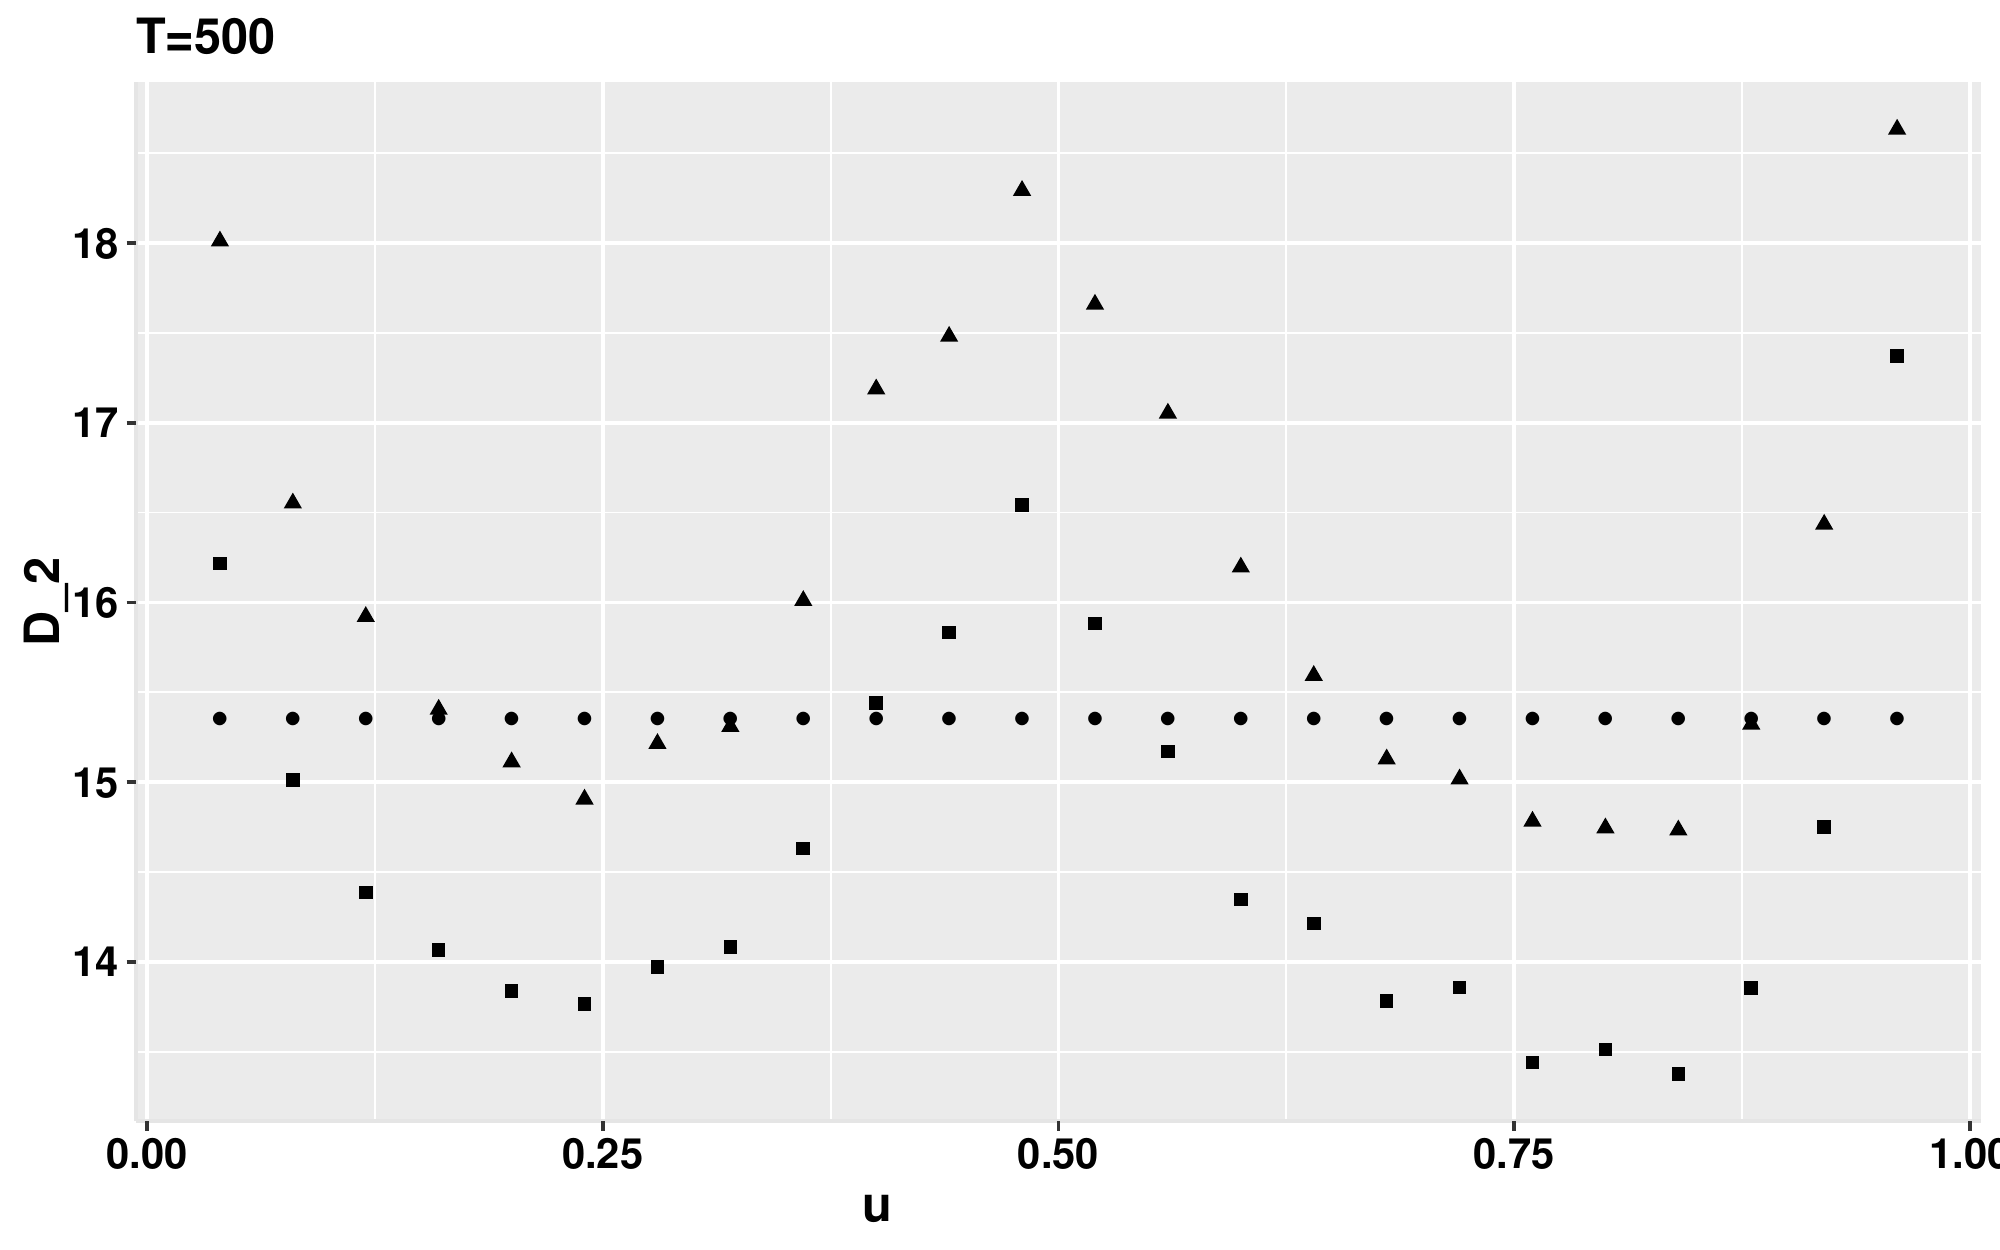}
\endminipage\hfill
\minipage{0.24\textwidth}%
  \includegraphics[width=\linewidth]{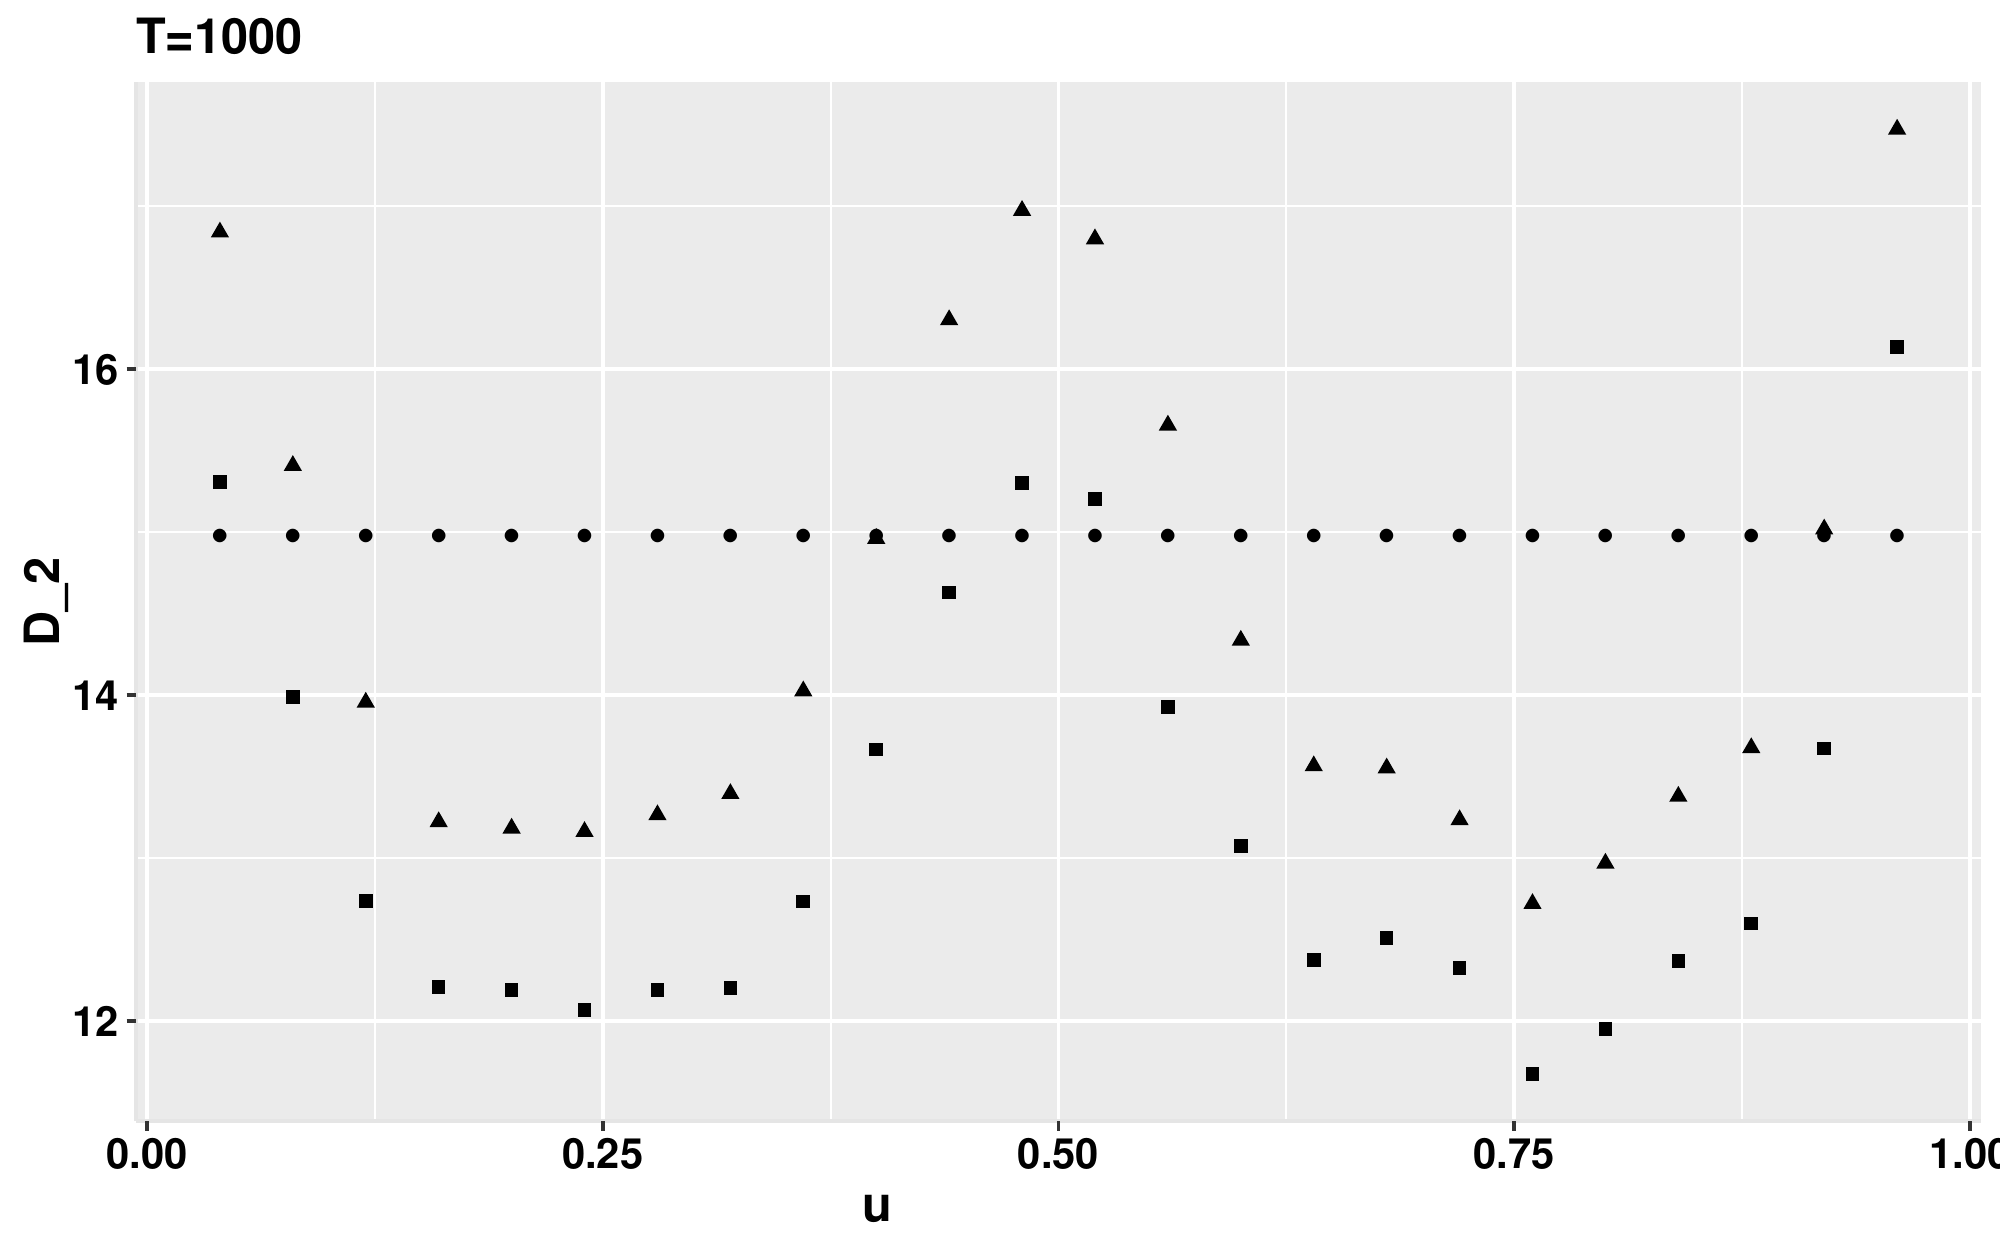}
\endminipage
\minipage{0.24\textwidth}%
  \includegraphics[width=\linewidth]{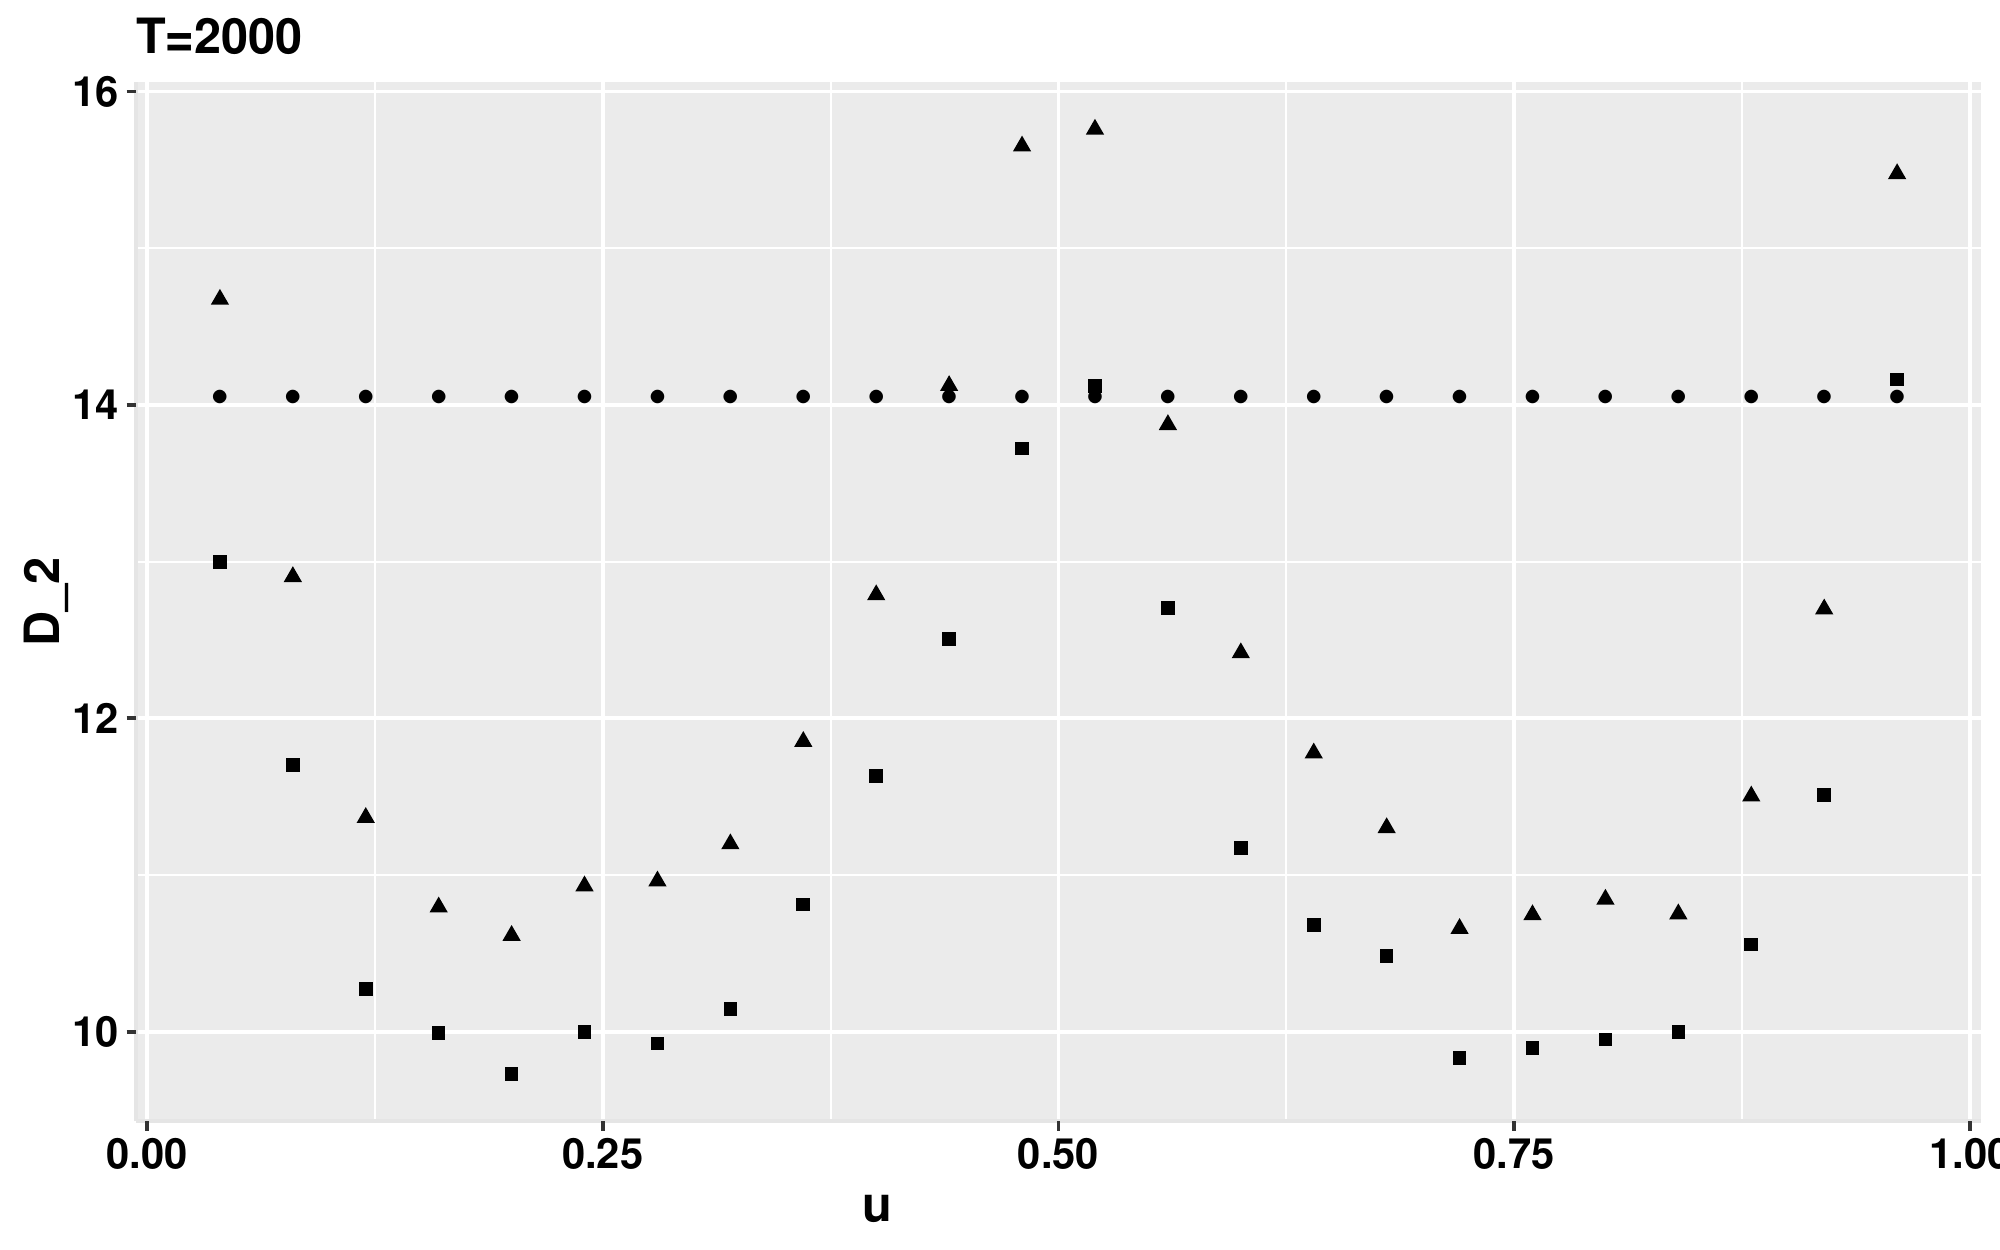}
\endminipage
\caption{Model 3 - Top:  Plot of $D_1(\widehat{B}_{1} (u) )$ against $u$ for the competing methods DSSA and VC and several sample sizes. VC (avg.) in triangles, VC (min.) in squares and DSSA in solid circles. Bottom: Analogous plot but with measure $D_2(\widehat{B}_{1} (u) )$ against $u$.  } \label{fig:m3_compare_d1d2}
\end{figure}

\begin{figure}[H]
\minipage{0.24\textwidth}
  \includegraphics[width=\linewidth]{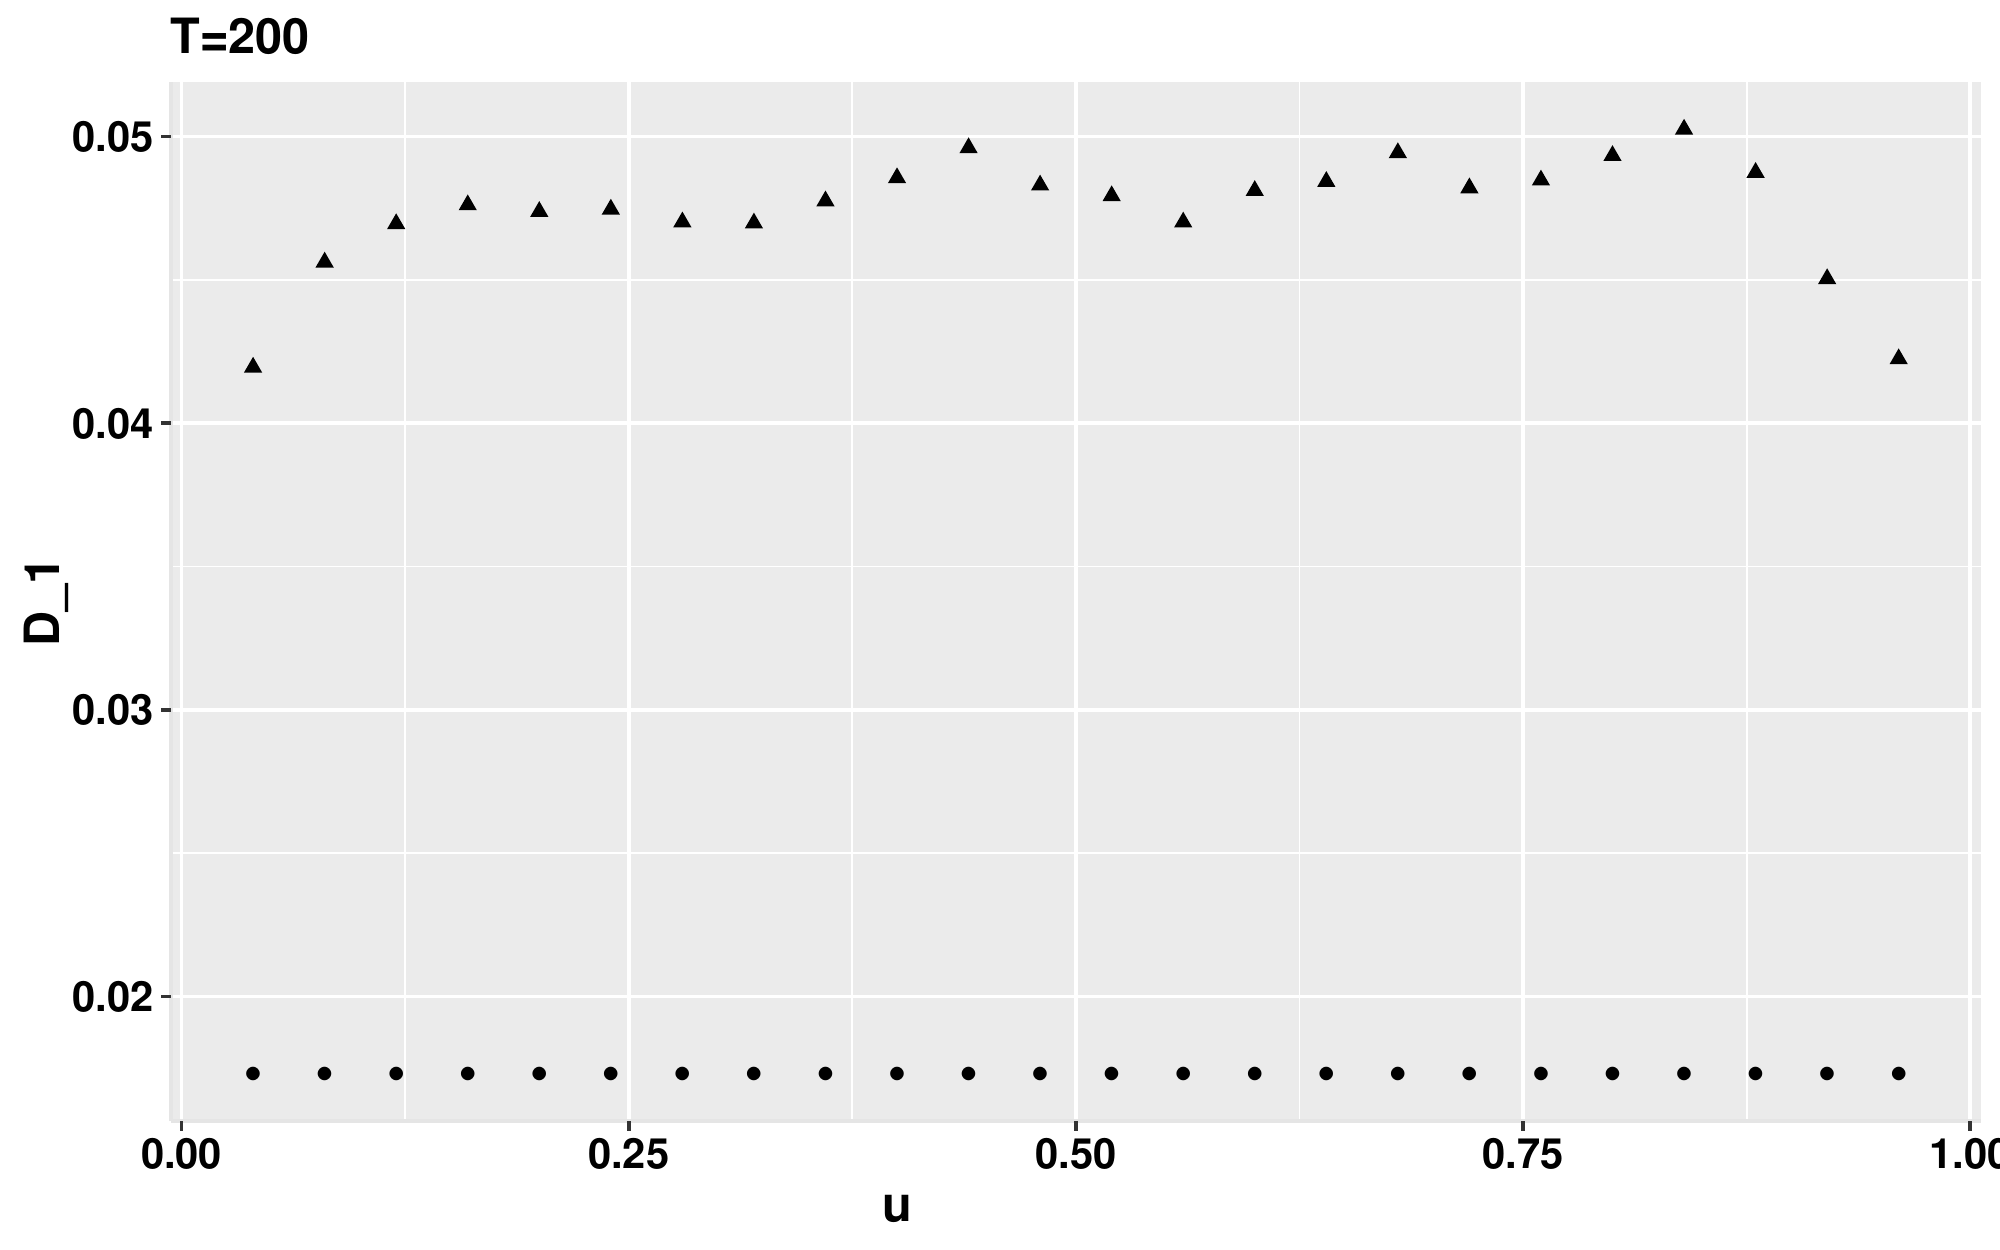}
\endminipage\hfill
\minipage{0.24\textwidth}
  \includegraphics[width=\linewidth]{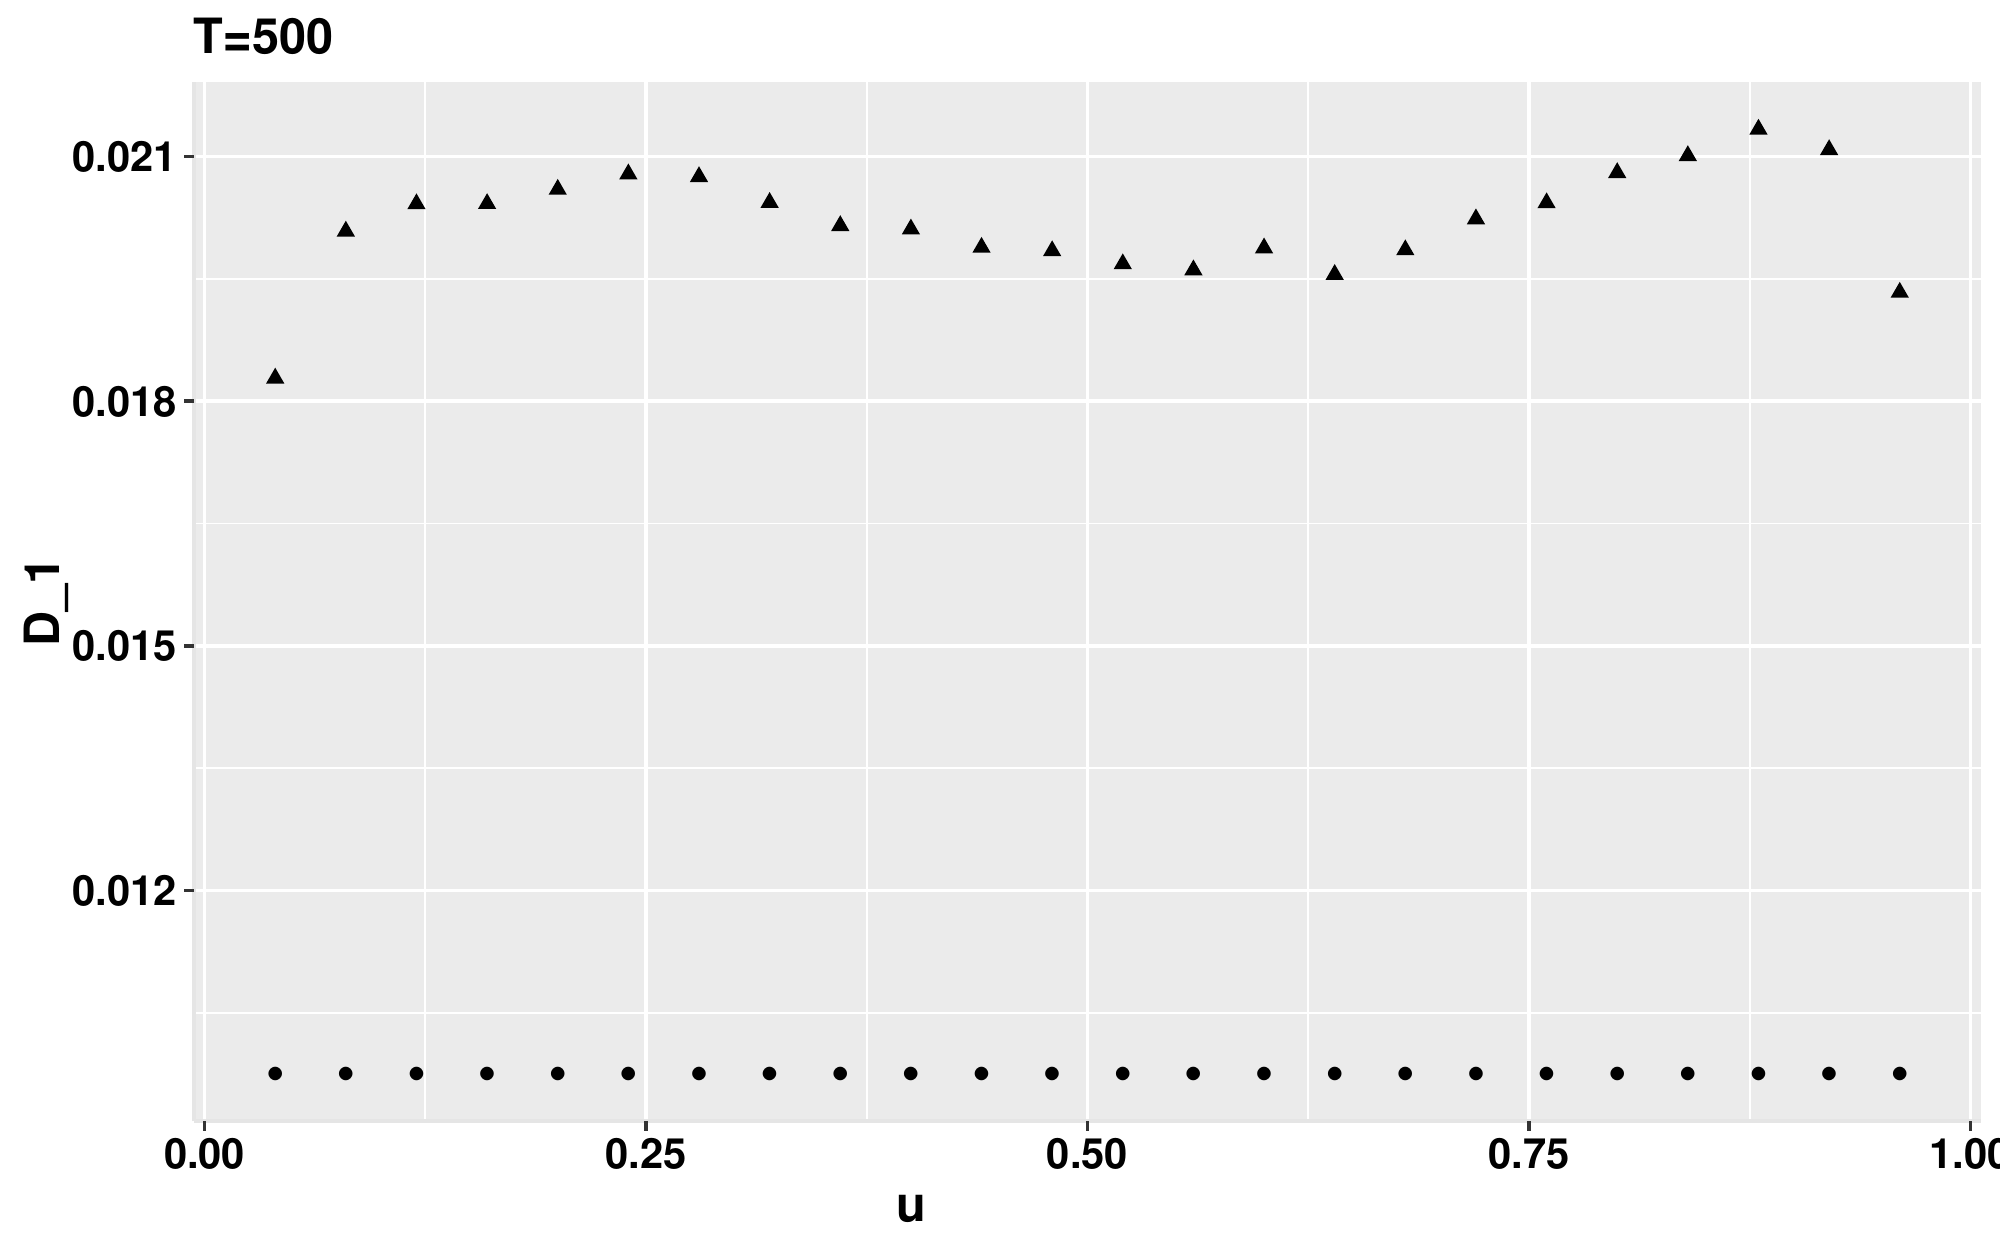}
\endminipage\hfill
\minipage{0.24\textwidth}%
  \includegraphics[width=\linewidth]{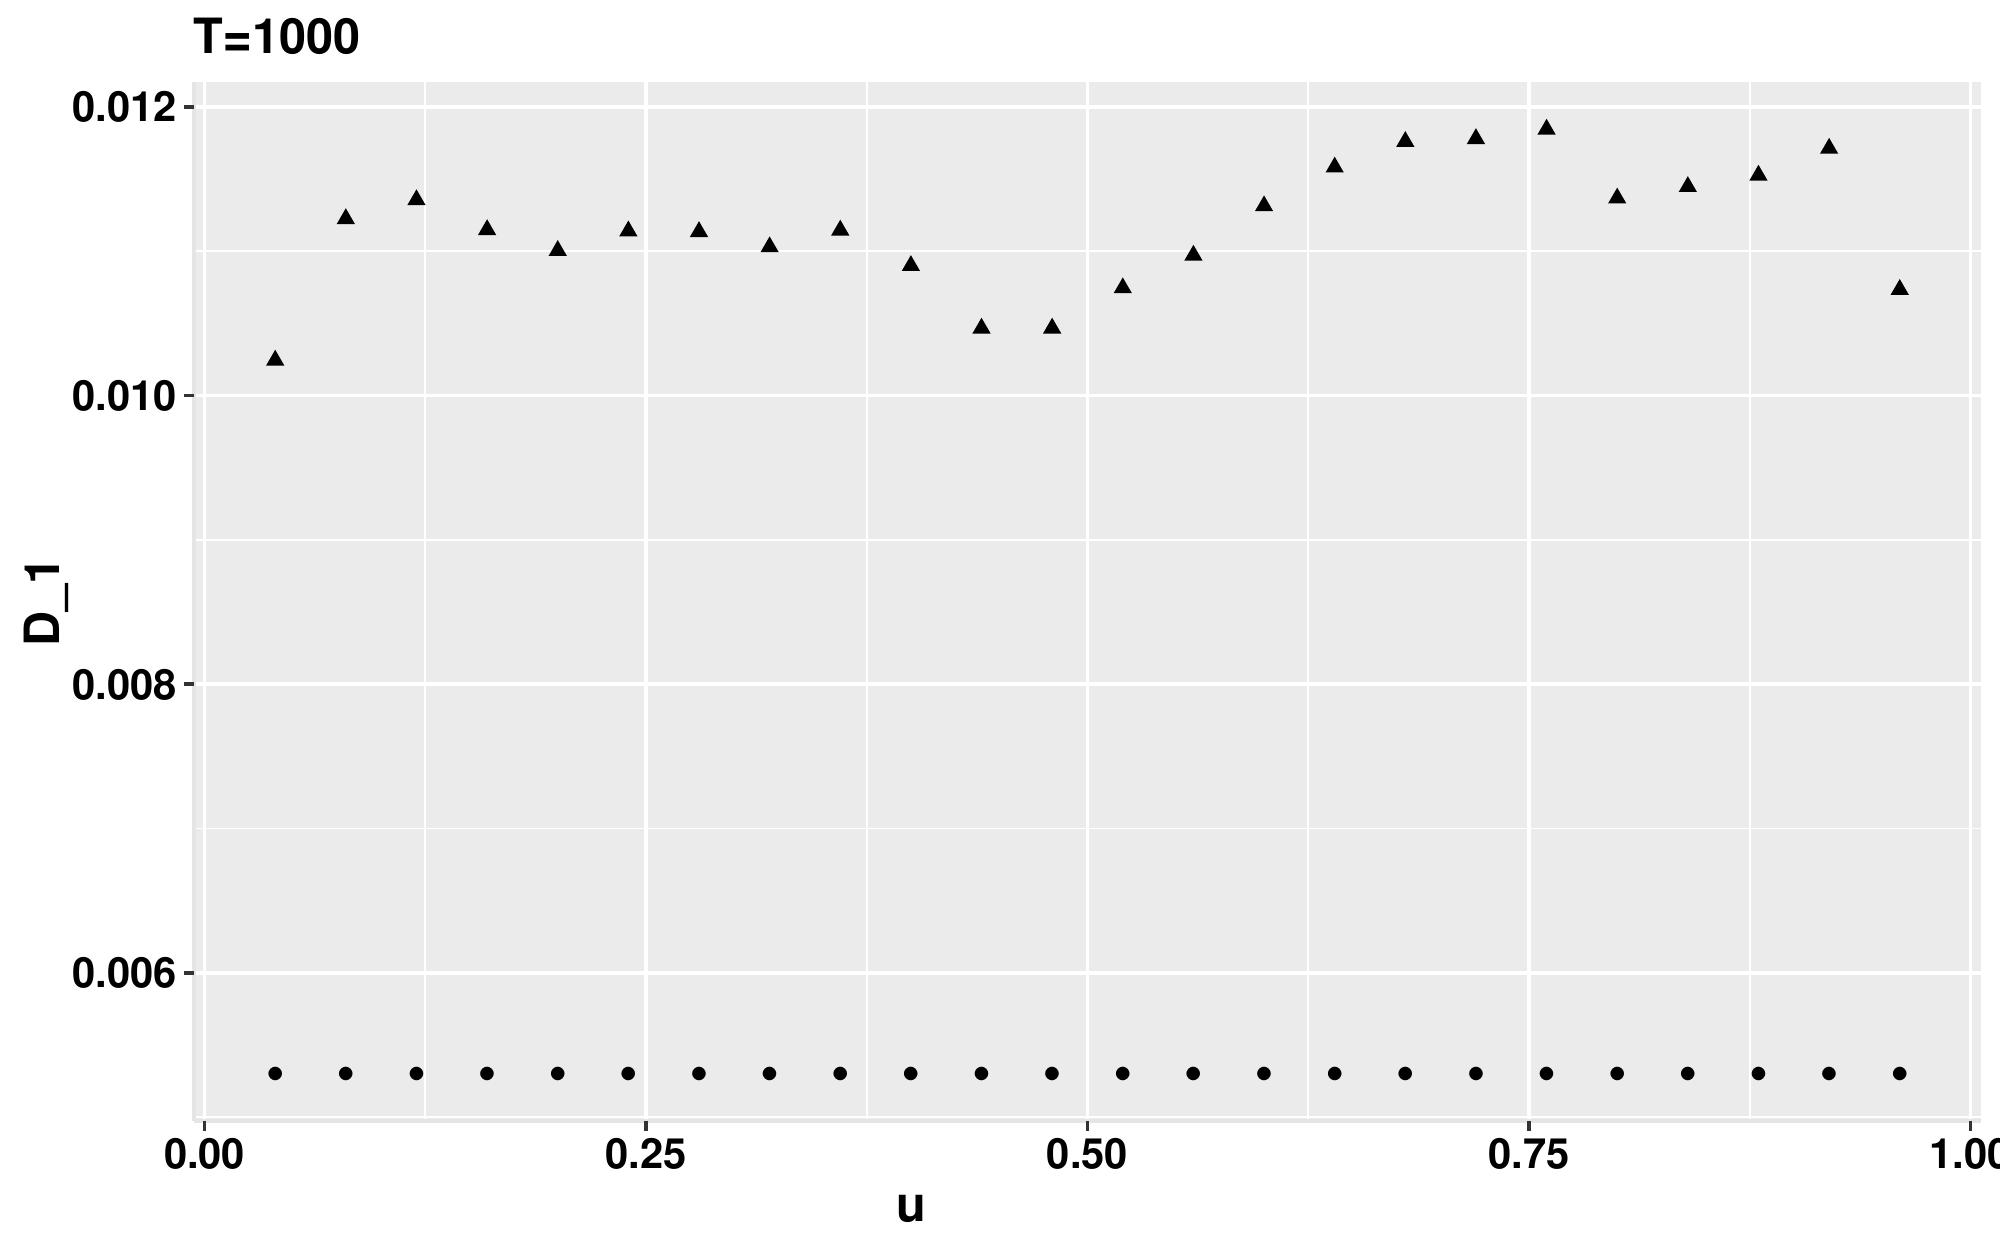}
\endminipage
\minipage{0.24\textwidth}%
  \includegraphics[width=\linewidth]{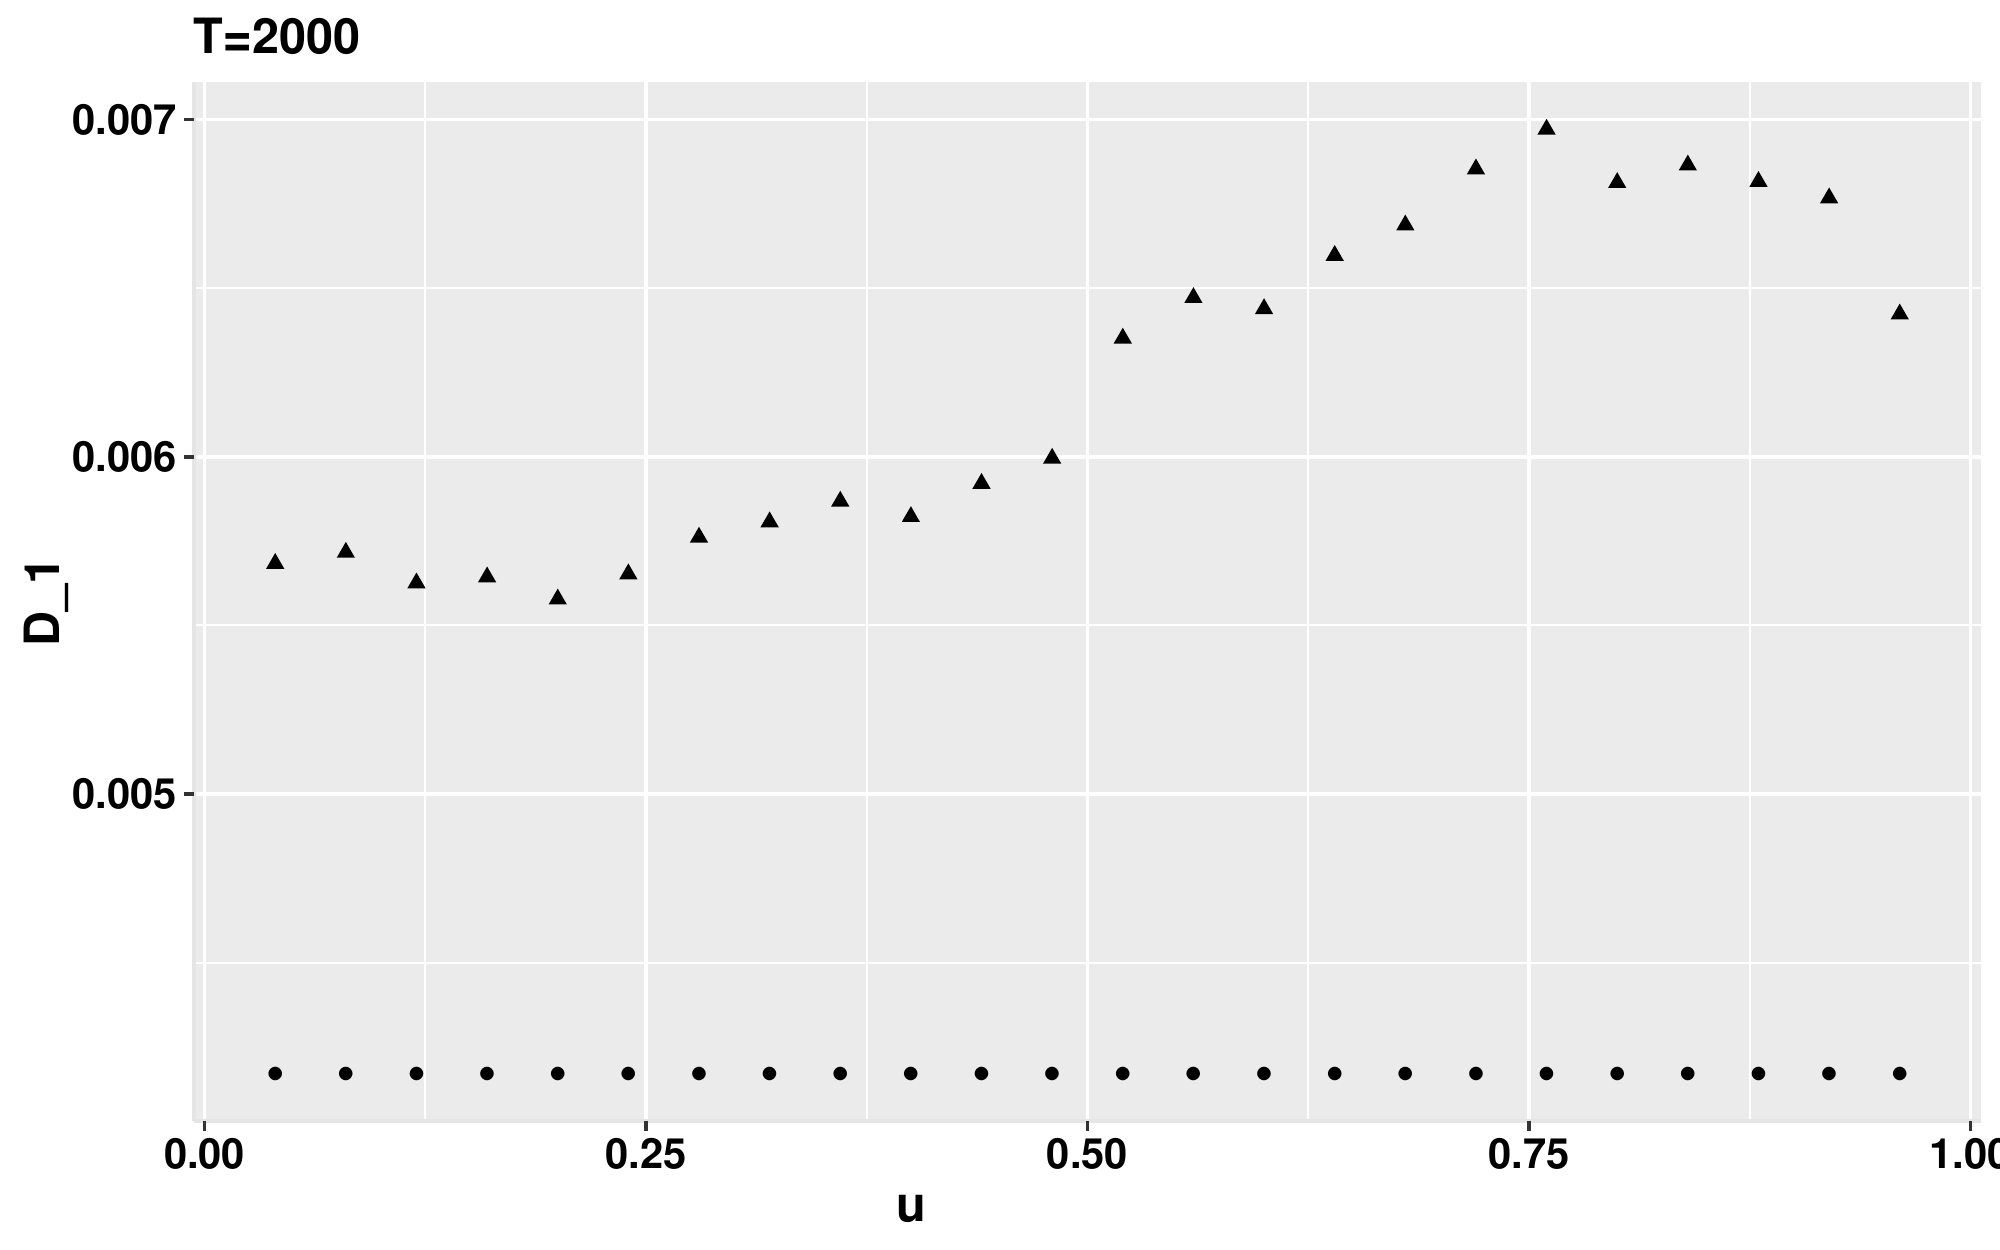}
\endminipage
% \caption{Model 1: Plot of $D_1(\widehat{B}_{1} (u) )$ against $u$ for the competing methods DSSA %and VC and several sample sizes.  } \label{fig:m1_compare_d1}
\end{figure}
\vspace{-0.5cm}
\begin{figure}[H]
\minipage{0.24\textwidth}
  \includegraphics[width=\linewidth]{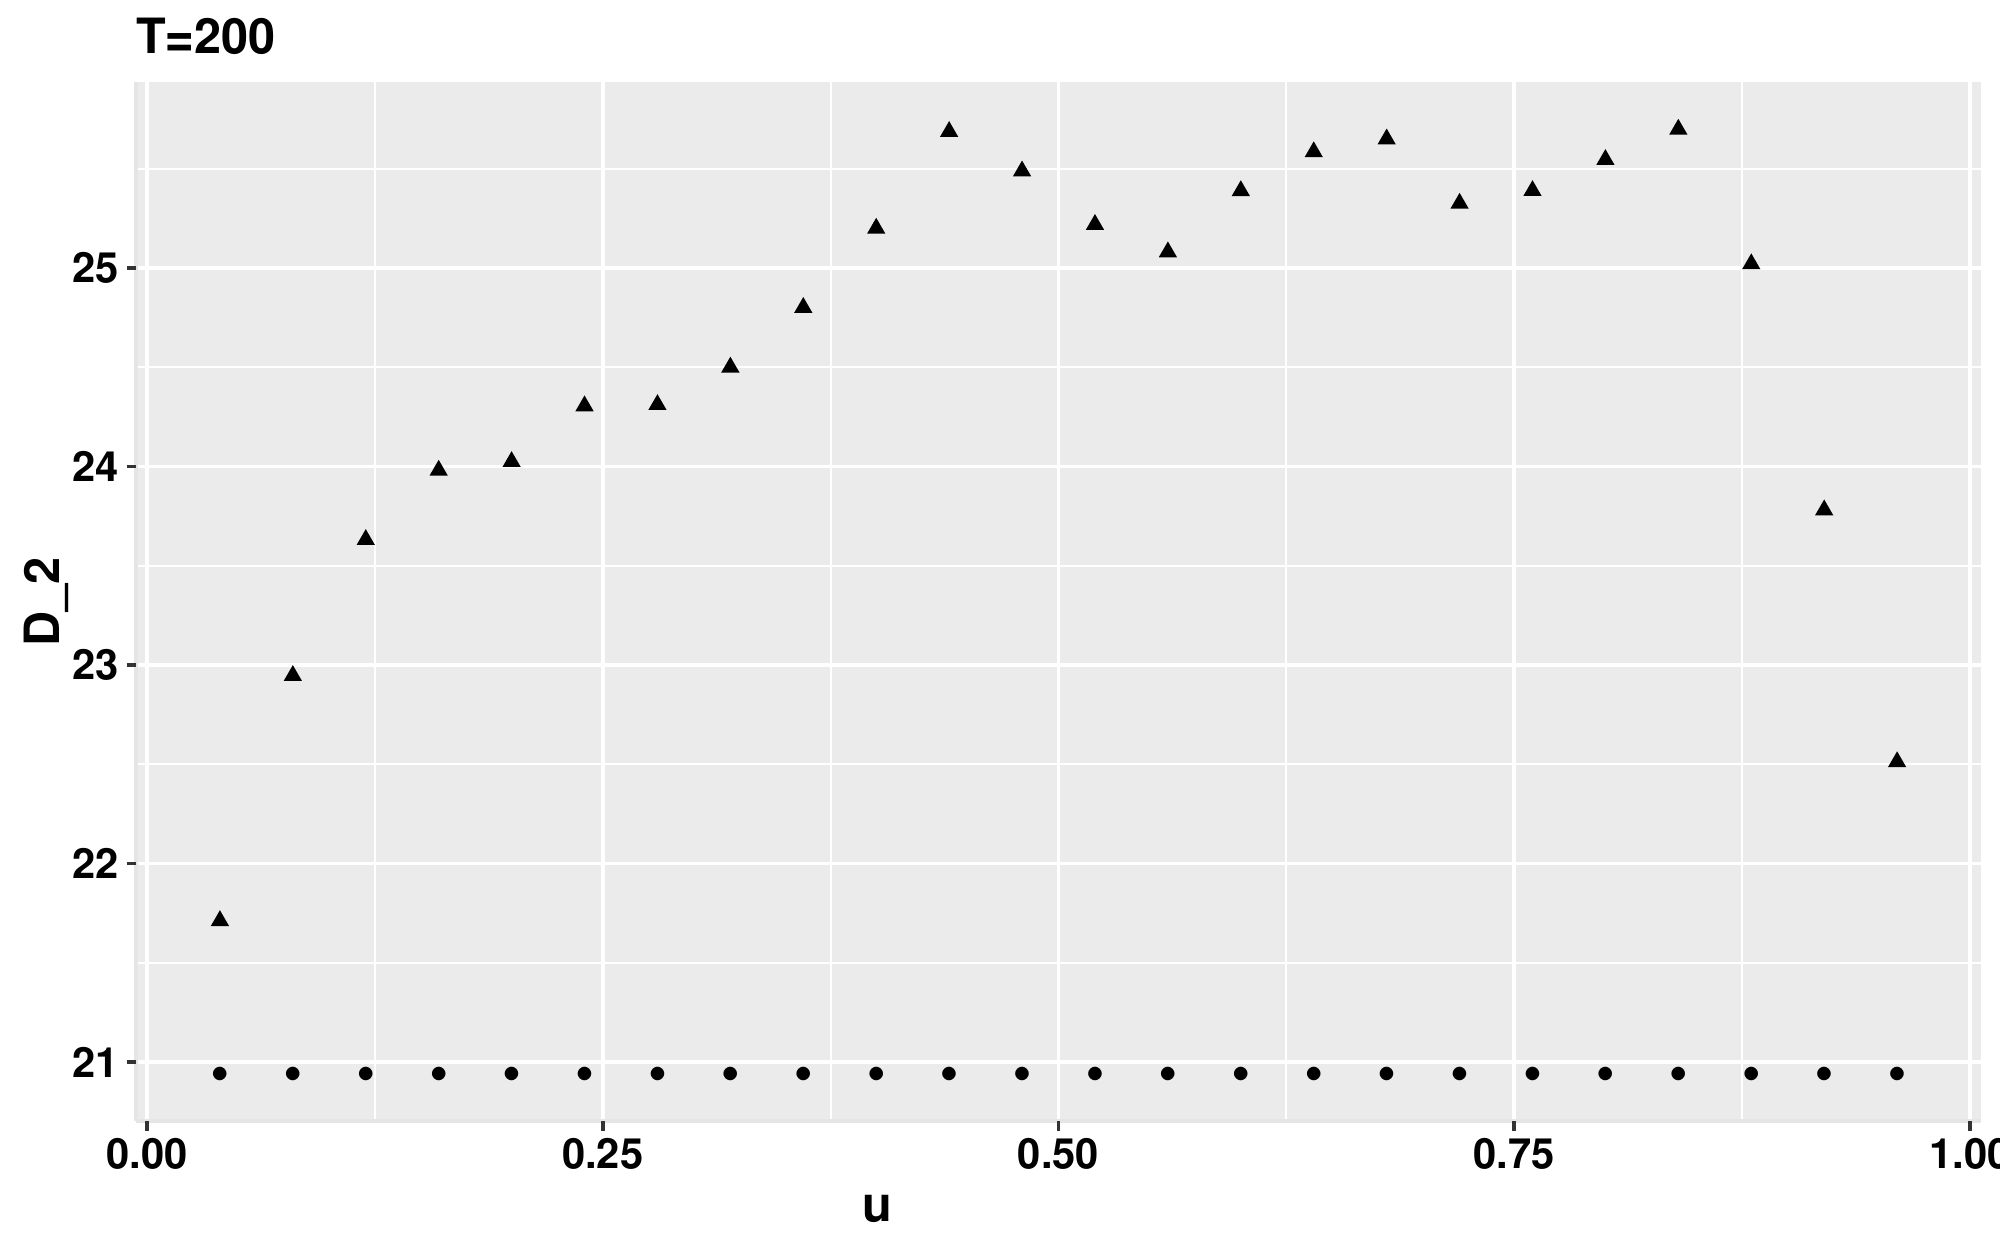}
\endminipage\hfill
\minipage{0.24\textwidth}
  \includegraphics[width=\linewidth]{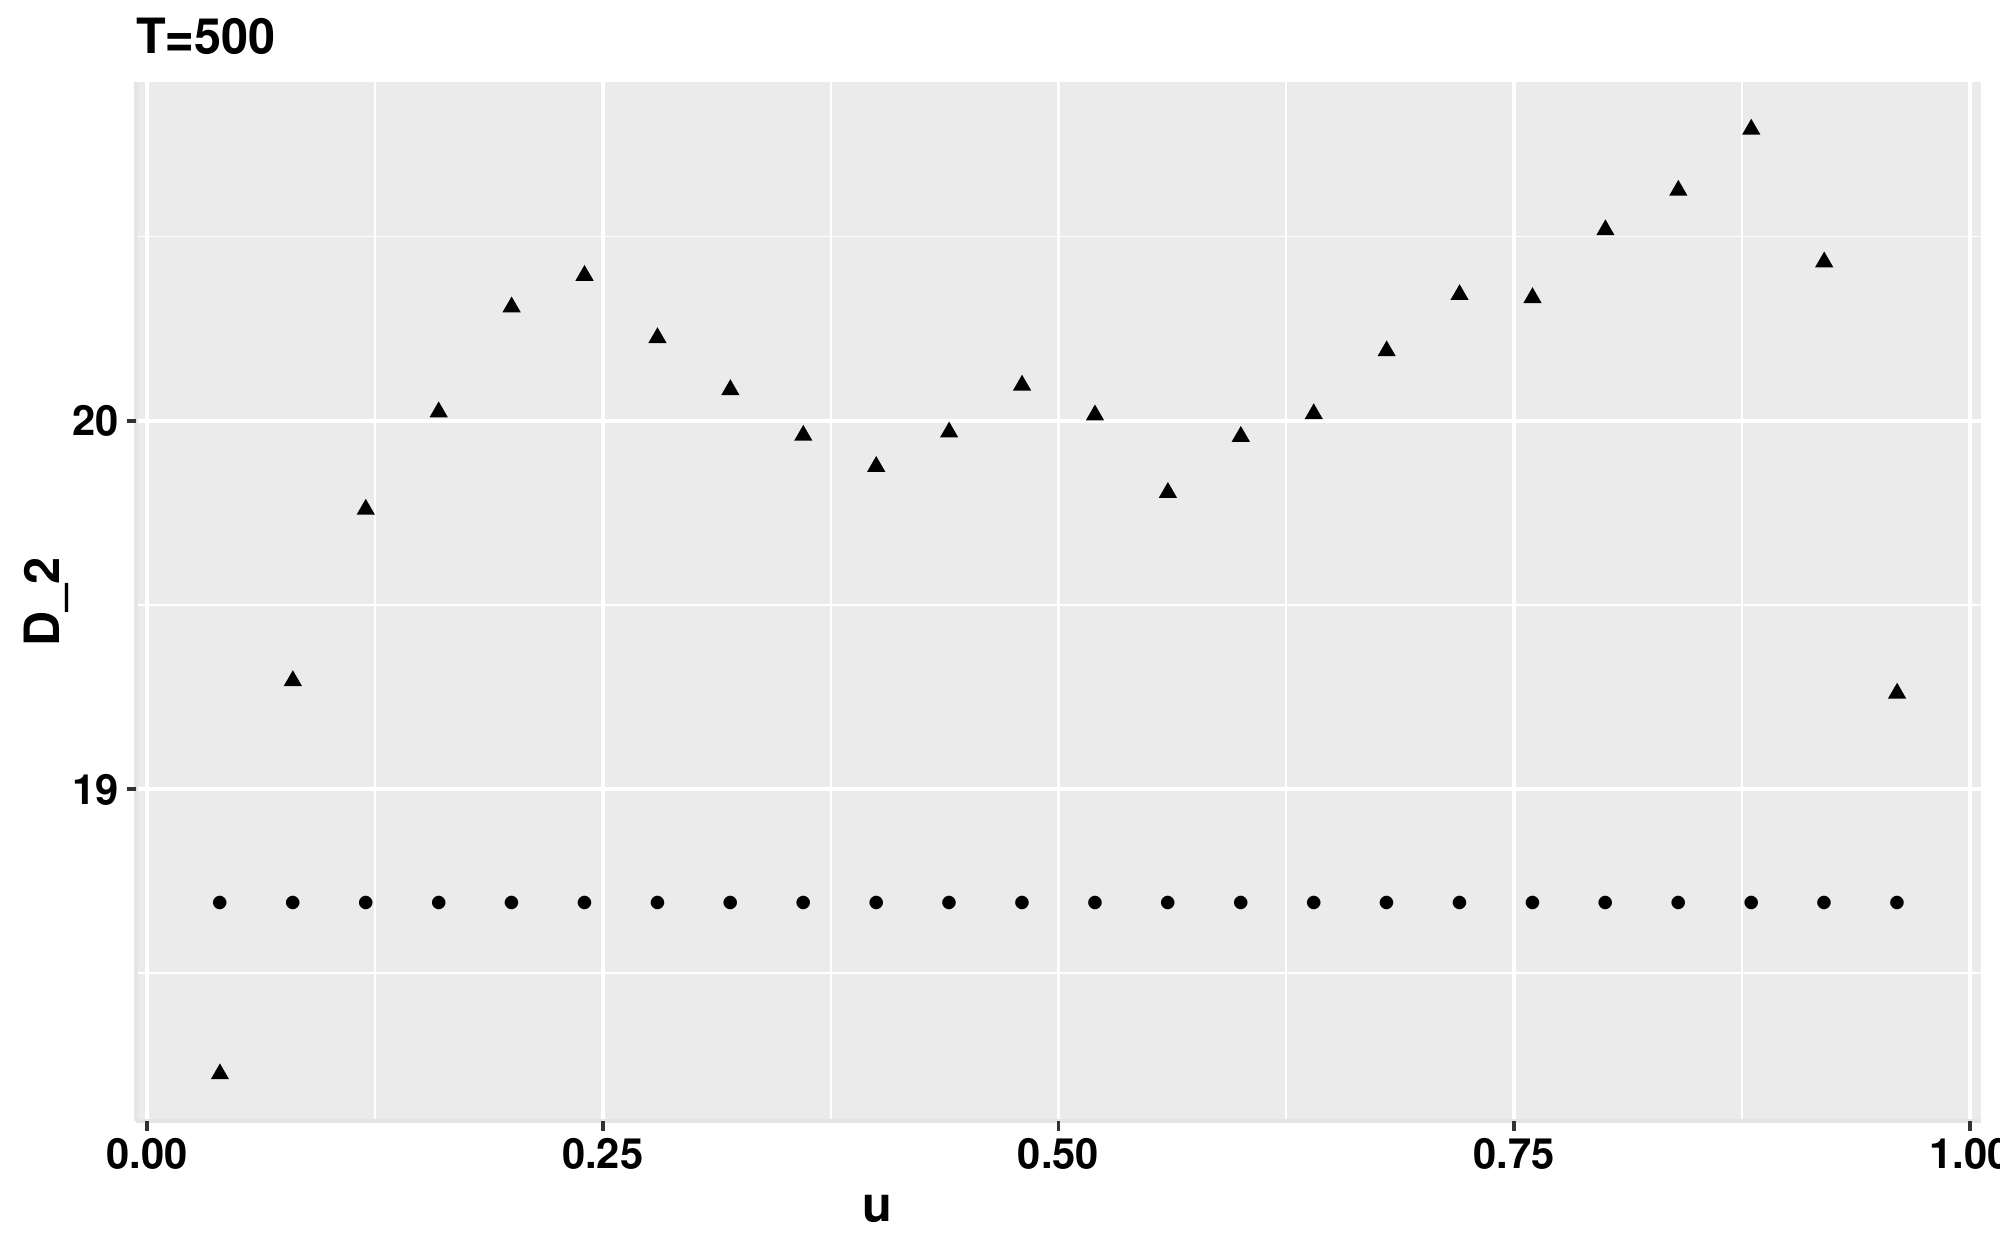}
\endminipage\hfill
\minipage{0.24\textwidth}%
  \includegraphics[width=\linewidth]{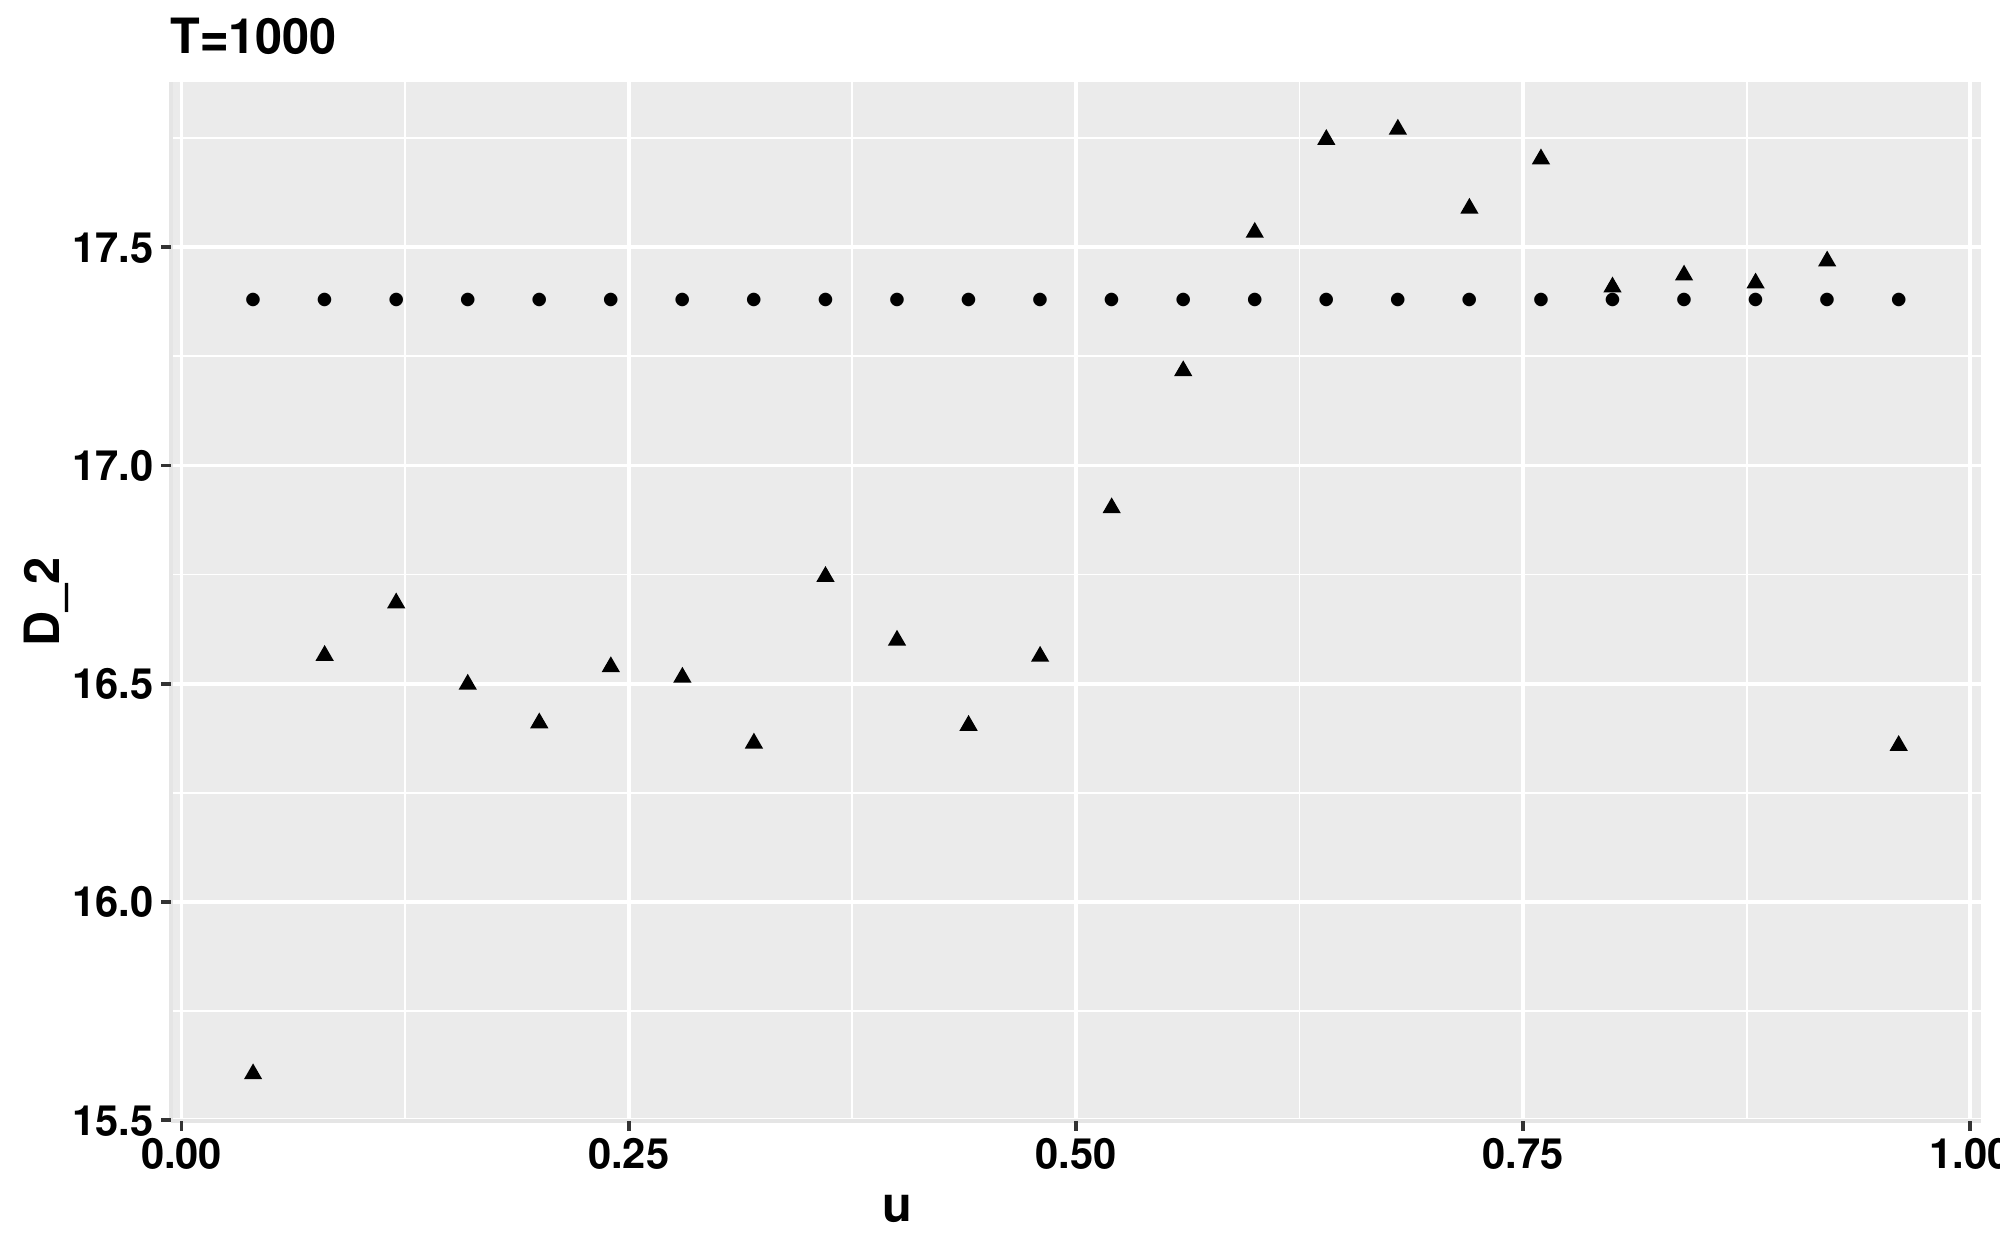}
\endminipage
\minipage{0.24\textwidth}%
  \includegraphics[width=\linewidth]{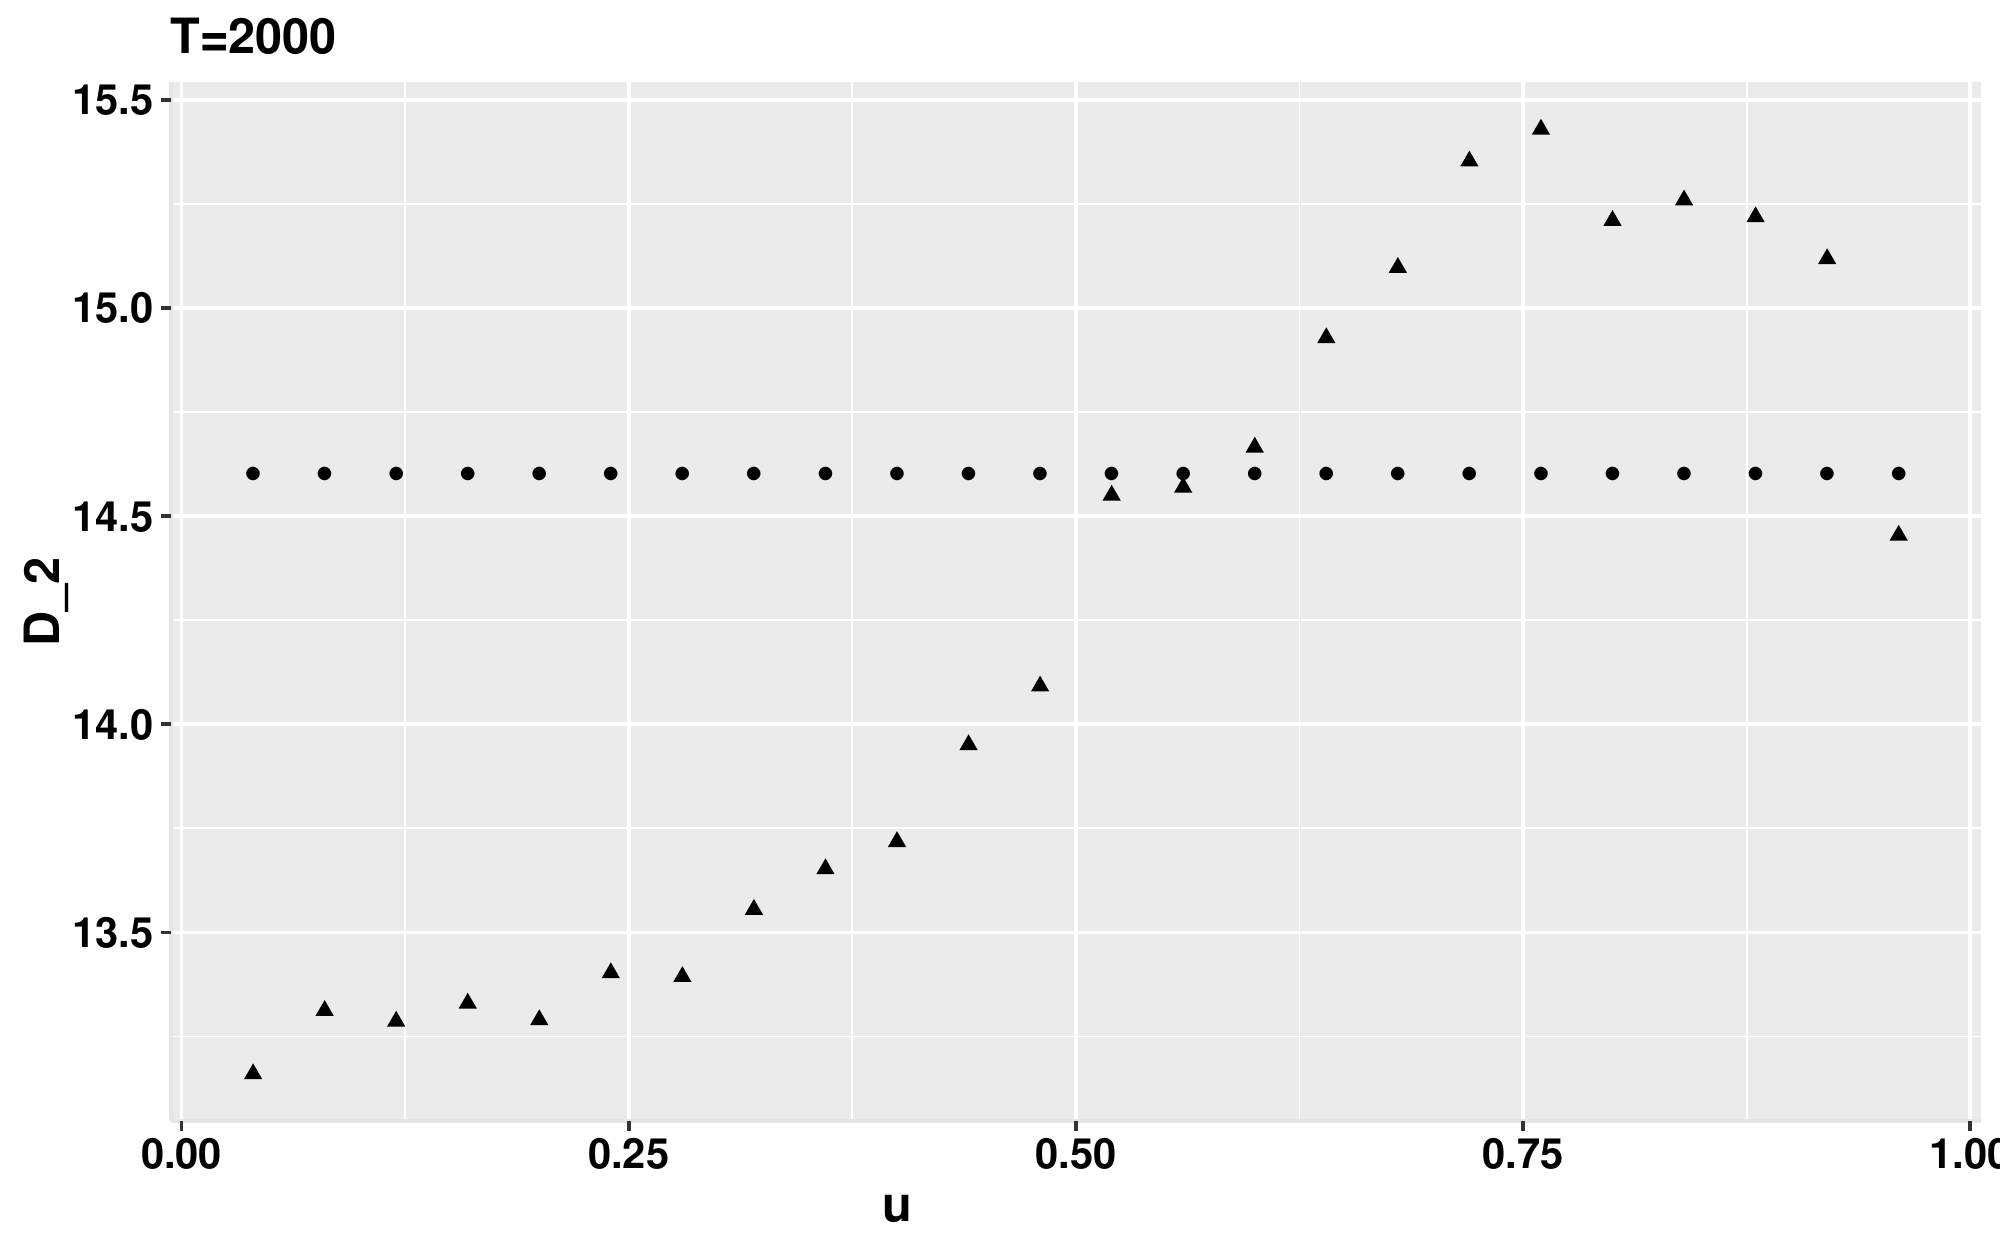}
\endminipage
\caption{Model 4 - Top:  Plot of $D_1(\widehat{B}_{1} (u) )$ against $u$ for the competing methods DSSA and VC and several sample sizes. VC (avg.) in triangles, VC (min.) in squares and DSSA in solid circles. Bottom: Analogous plot but with measure $D_2(\widehat{B}_{1} (u) )$ against $u$.  } \label{fig:m4_compare_d1d2}
\end{figure}

\section{Additional figures and tables for Section \ref{s:application}}

\begin{figure}[H]
\begin{center}
\includegraphics[scale=0.4]{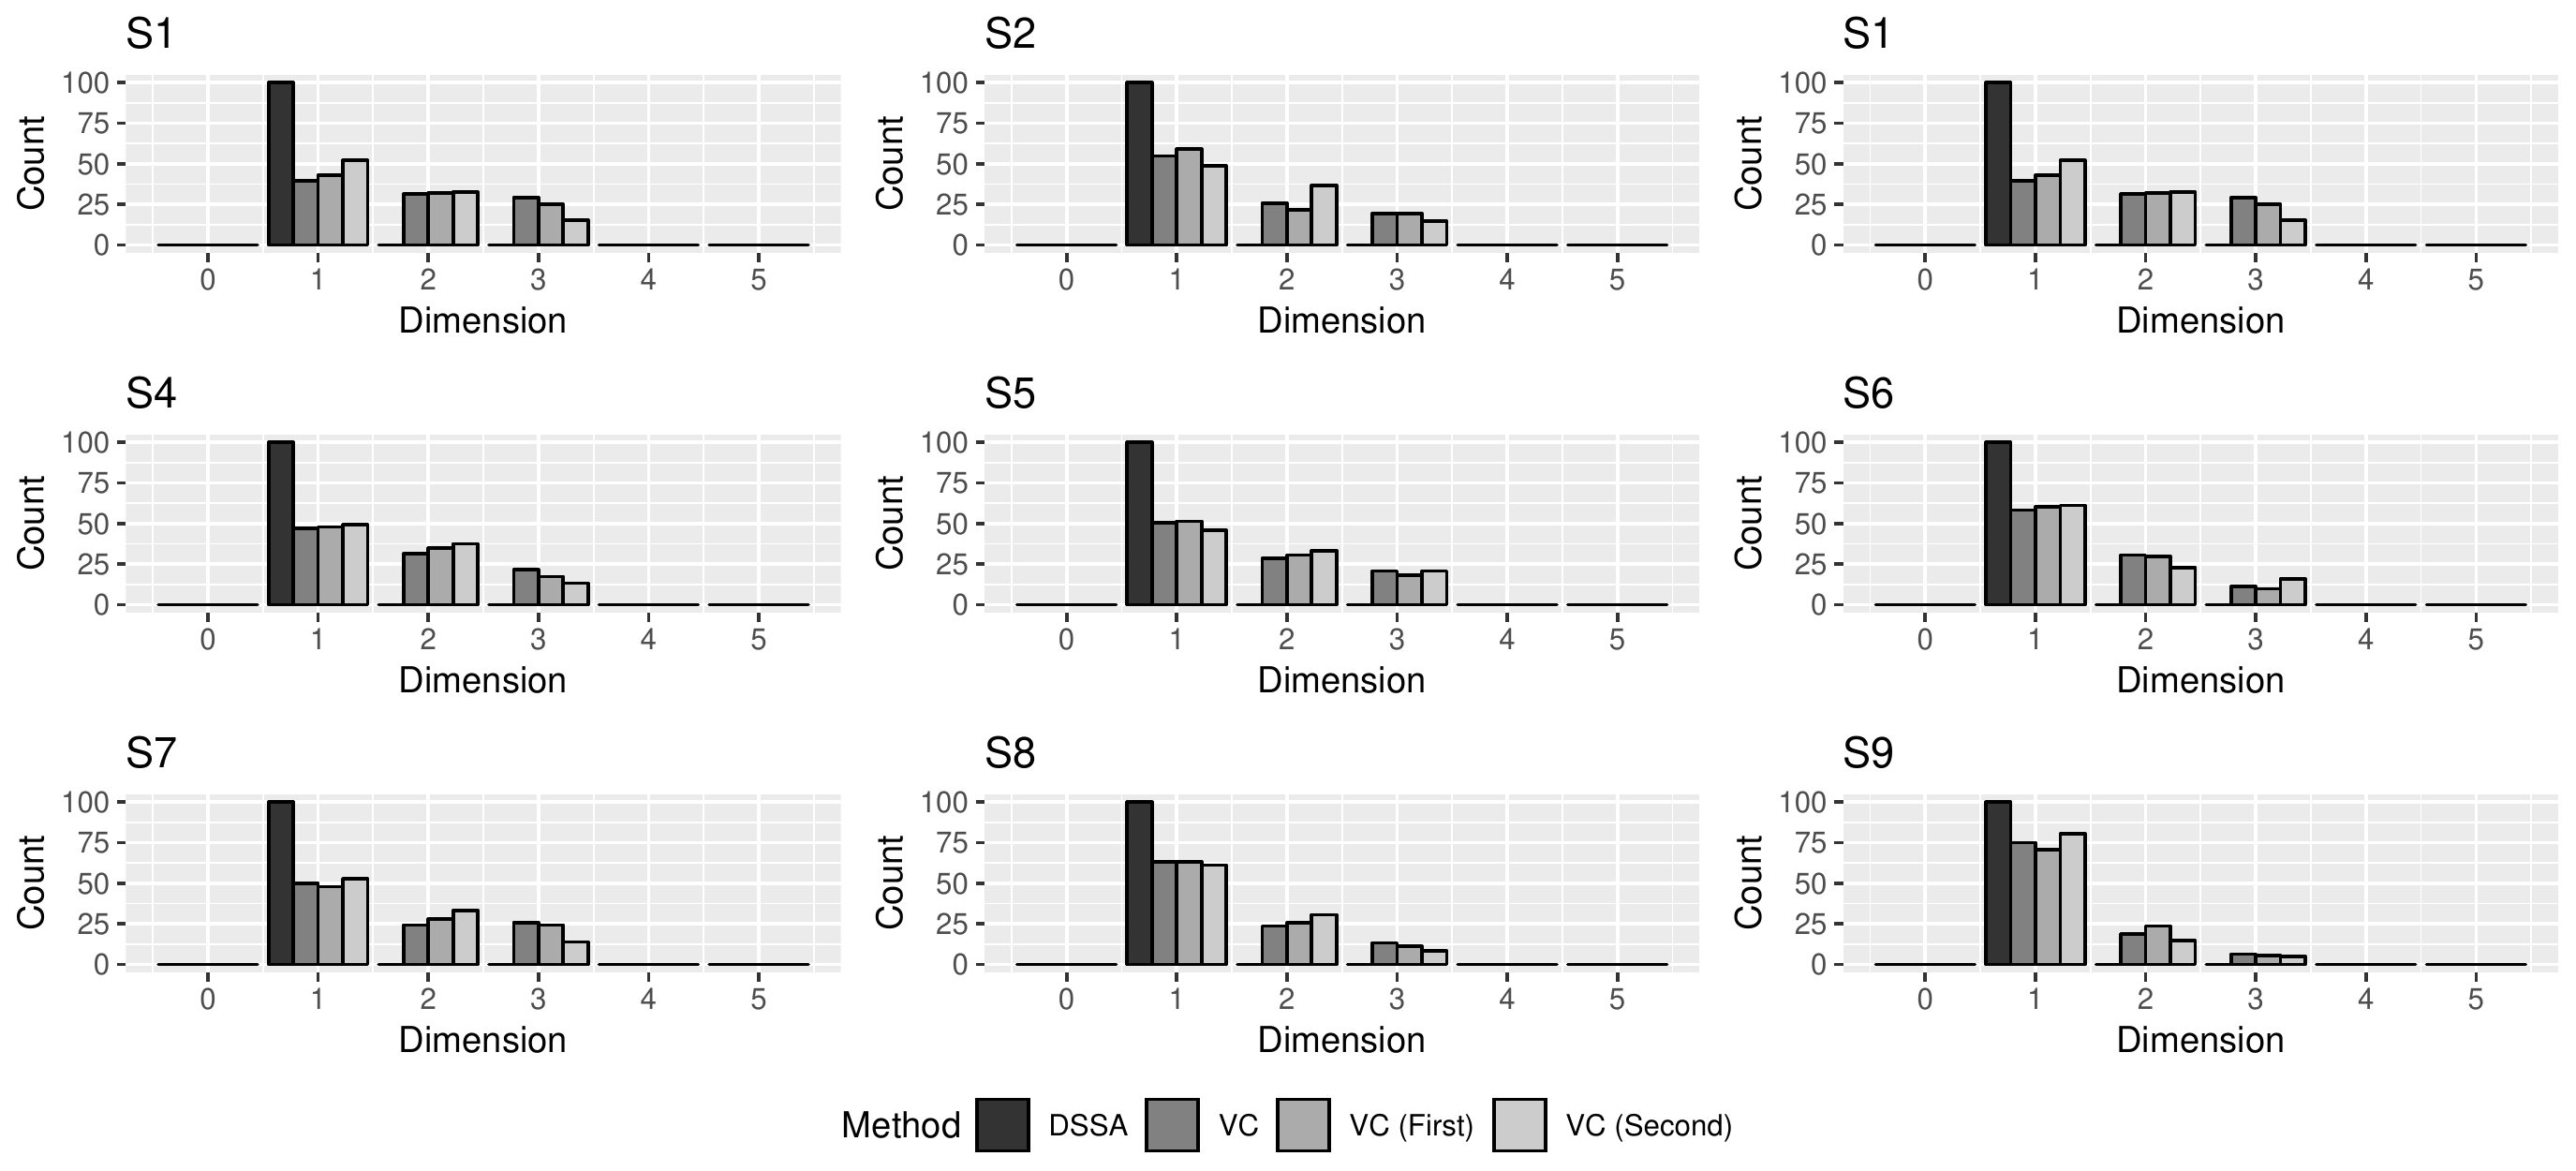}
\end{center}
\vspace{-0.75cm}
\caption{ Histogram of the dimension estimates $d$ by the two competing methods based on the 144 trials.   } \label{fig:bci_dim_plot_supp}
\end{figure}

\vspace{-0.8cm}
%\begin{center}
%\begin{table}[H]
%\begin{tabular}{|c |c | c | c |c| c| c |c| c | c| c |}
%\hline
%Distance Measure &  & S1 & S2 & S3 & S4 & S5 & S6 & S7 & S8 & S9 \\
%\hline
%\multirow{2}{*}{$D_3$} & Median & 0.74 & 0.73 & 0.75  & 0.73 & 0.74 & 0.77 & 0.76 & 0.74 & 0.78 \\
% & Mean & 0.68 & 0.68 & 0.67 & 0.69 & 0.67 & 0.69 & 0.68 & 0.69 & 0.73 \\
%\hline
%\multirow{2}{*}{$D_4$} & Median & 0.98 & 0.97 & 1.02  & 0.97 & 1 & 1.01 & 1.06 & 1 & 1.13 \\
% & Mean & 0.95 & 0.97 & 0.97 & 0.95 & 0.94 & 1 & 0.98 & 1 & 1.07 \\
%\hline
%\end{tabular}
%\caption{  Mean and median distance (in radians) between the estimated subspaces using DSSA and VC over %144 trials for subjects S1 to S9. Distances are based on $D_3$ and $D_4$ from Section %\ref{s:simulation_subspace}.} \label{tab:bci_subspace_distance_supp}
%\end{table}

\begin{table}[H]
\begin{tabular}{ |c |c |c |c | c| c |c| c | c| c |c | c|}
\hline
$d$ & & S1 & S2 & S3 & S4 & S5 & S6 & S7 & S8 & S9 & Avg \\
\hline
\multirow{2}{*}{$1$} & DSSA  & 51.22  & 54.86   & 56.25   &  58.33  & 49.03   & 45.13   & 54.16  &  51.11 &  51.38  & 52.38  \\
 & VC   &  50   & 49.31  & 50.69 & 46.52 & 52.08 & 54.16 & 50.69 & 46.15  & 54.86 & 50.49 \\
\hline
\multirow{2}{*}{$2$} & DSSA  & 58.37  & 57.63  & 54.86  & 61.11  & 54.16 & 52.08 & 52.77 & 56.45  & 52.78  & 55.57 \\
 & VC   &    53.14   & 59.72 & 48.61 & 57.63 & 55.56 & 52.77 & 54.17 &   45.05  & 50.69 &  53.10 \\
\hline
\multirow{2}{*}{$3$} & DSSA  & 60.48 & 58.33 & 59.02  & 55.56 & 59.33 & 56.20 & 62.50  & 64.39 & 56.94  & 59.19 \\
 & VC   &  60.13   & 61.11 & 47.22 & 56.94 & 57.63 & 55.56 & 61.81 &   54.54   & 54.16 &  56.57 \\
\hline
\multirow{2}{*}{$4$} & DSSA  & 60.17  & 62.50 & 56.25 & 66.67 & 62.50 & 55.56  & 65.27 & 66.28  & 55.56  & 61.19 \\
 & VC  &  58.04   & 60.41 & 65.97  & 66.67 & 64.58 & 57.63 & 66.67 &    59.44  & 56.94 & 61.82 \\
\hline
\end{tabular}
\caption{ Out-of-sample classification accuracy (in \%) for the 9 subjects S1-S9 for the two
  indicated methods.}  \label{tab:bci_acc_rate_supp}
\end{table}

\vspace{-0.8cm}

\begin{figure}[H]
\begin{center}
\includegraphics[scale=0.4]{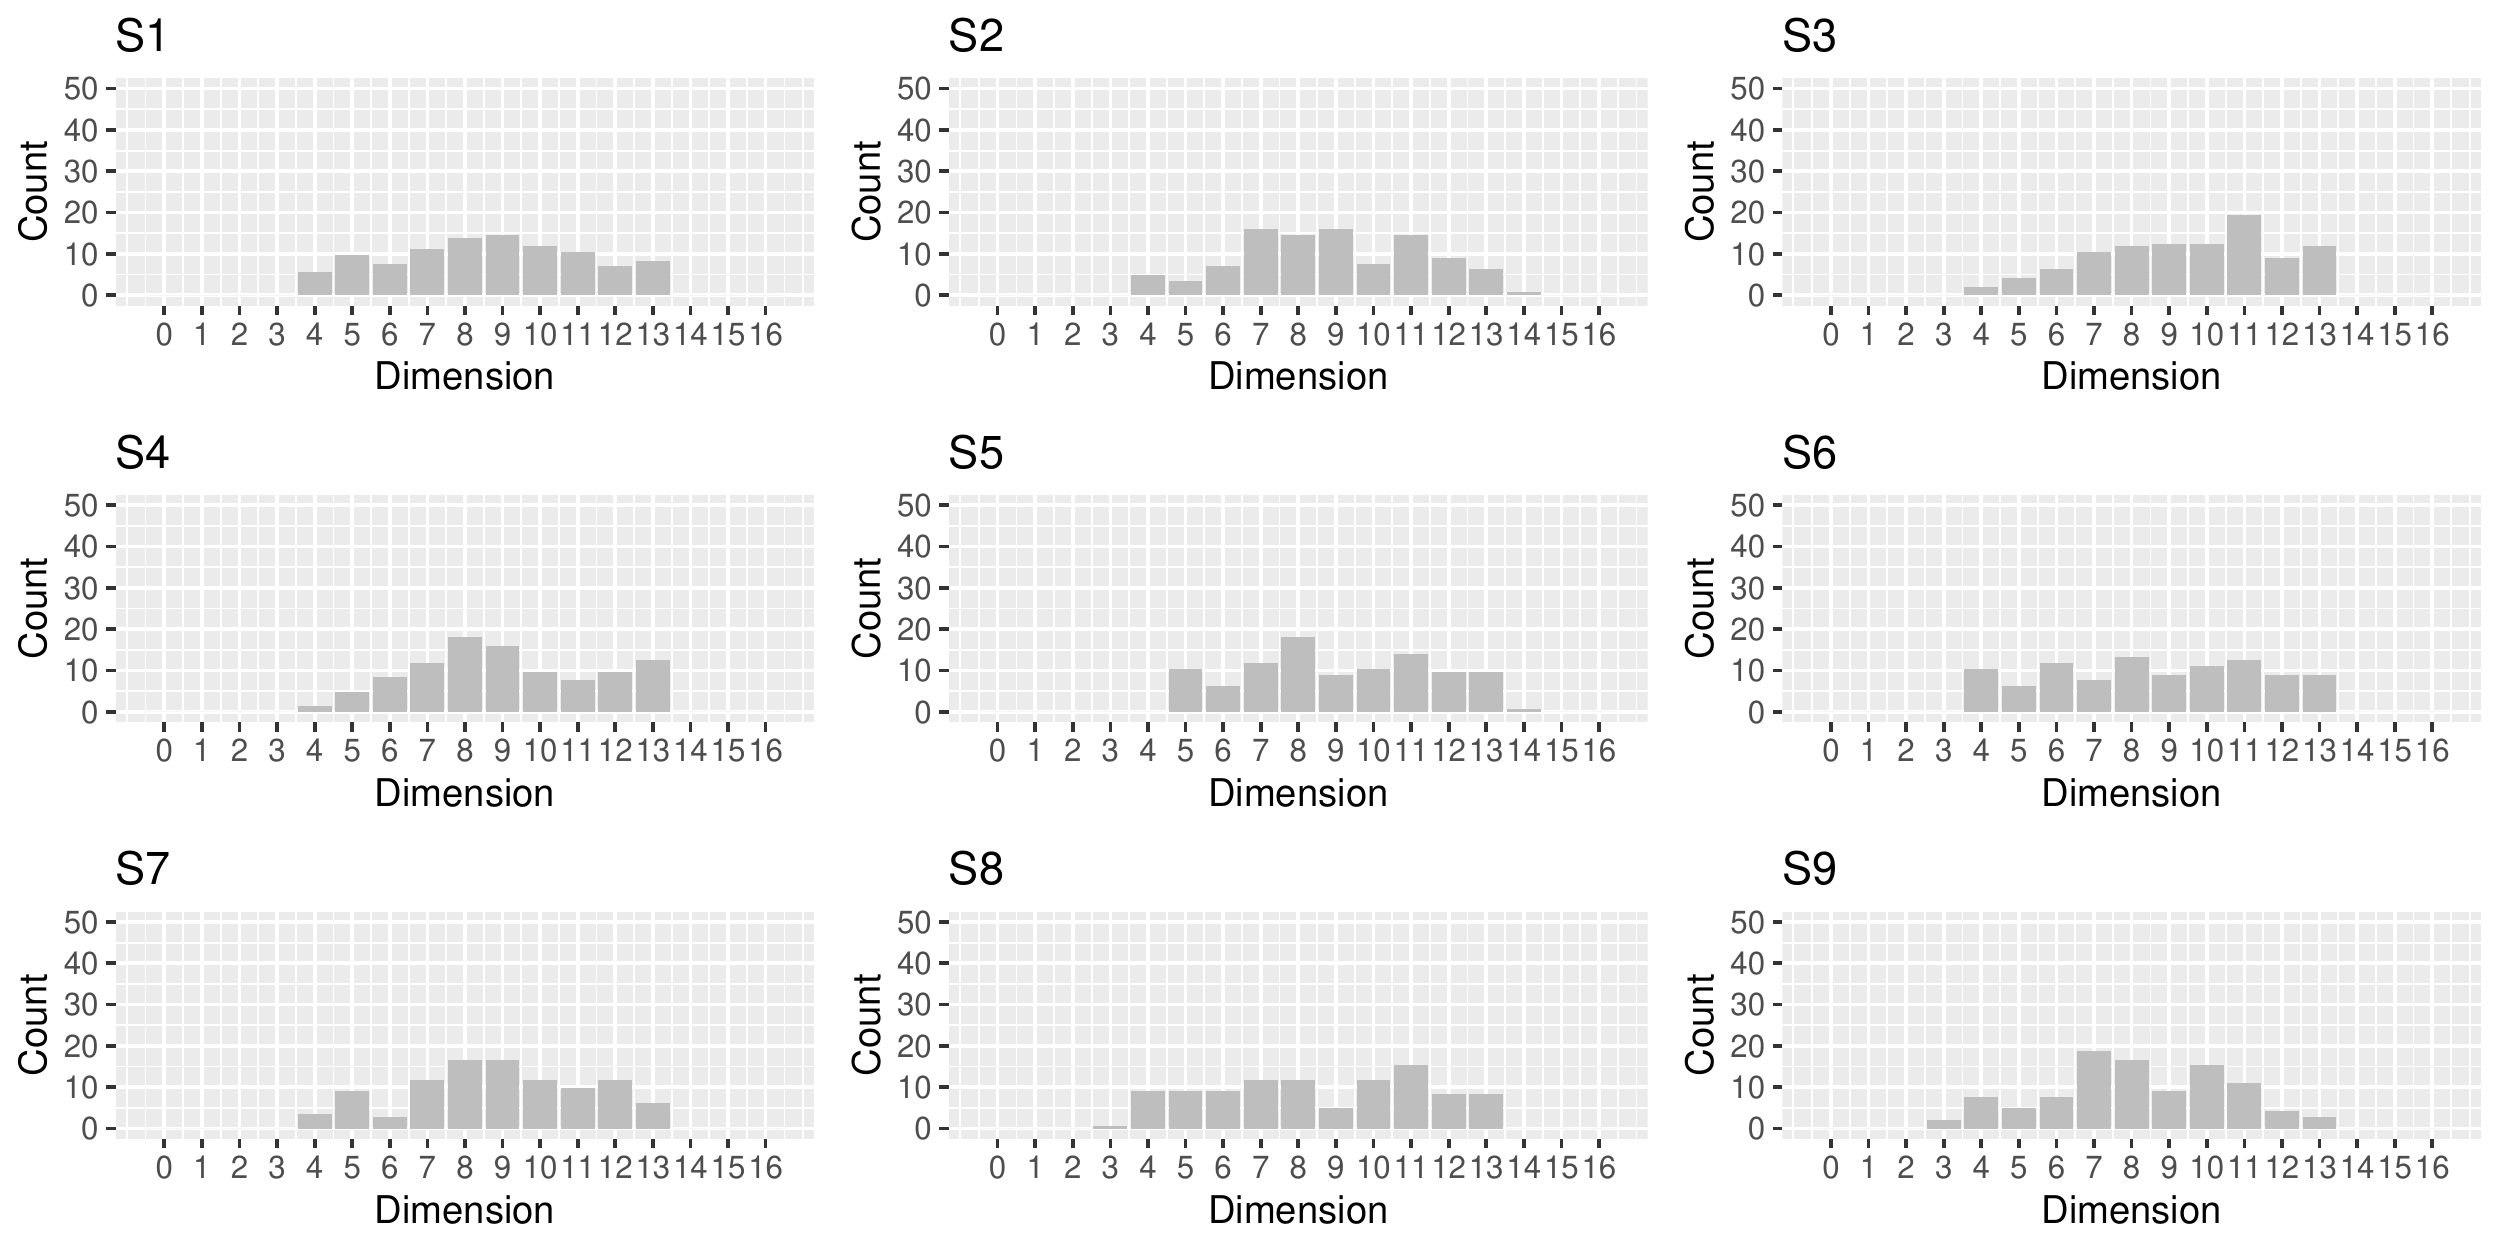}
\end{center}
\vspace{-0.75cm}
\caption{ $p=22$. Histogram of the stationary subspace dimension estimates based for VC method based on the 144 trials.   } \label{fig:bci_dim_plot_p-22_supp}
\end{figure}

\begin{table}[H]
\begin{center}
\begin{tabular}{ |c | c |c |c| c| c |c| c | c| c |c | c|}
\hline
$d$ & Method & S1 & S2 & S3 & S4 & S5 & S6 & S7 & S8 & S9 & Avg \\
\hline
\multirow{2}{*}{7} & VC  & 74.12   & 66.67  & 70.83 & 73.51 & 73.61 & 70.83 & 74.30 & 68.53  & 69.44 & 71.32  \\
 & DSSA  & 69.67 & 67.57 & 70.00 & 64.52 & 60.48 & 63.70 & 66.67 & 68.30 & 68.55 & 66.60  \\
\hline
\multirow{2}{*}{9} &  VC &    80.41   & 75 & 72.22 & 77.08 & 81.25 & 74.30 & 77.08 &  71.32  & 77.08 & 76.19  \\
 & DSSA  & 71.52 & 69.96 & 77.90 & 77.48 & 65.50 & 70.55 & 71.41 & 70.38 & 69.80 & 71.61 \\
\hline
\multirow{2}{*}{11} &  VC & 87.40   & 84.72 & 74.30 & 81.94 & 88.19 & 81.25 & 82.63 &  81.25 & 81.25 & 82.55 \\
 & DSSA  & 75.78 & 69.97 & 72.92 & 75.96 & 69.58 & 71.95 & 68.34 & 71.33 & 73.31  & 72.12 \\ 
\hline
\multirow{2}{*}{13} & VC &  89.50   & 90.97 & 85.41  & 88.19 & 89.58 & 88.19 & 90.27 &  84.72  & 84.72 & 87.95 \\
& DSSA  & 79.86 & 70.98 & 80.56 & 78.24 & 70.83 & 77.62 & 73.55 & 78.38 & 74.72 & 76.08 \\
\hline
\end{tabular}
\vspace{-0.3cm}
\caption{ Out-of-sample classification accuracy (in \%) for the 9 subjects S1-S9 corresponding to $d=$ 7, 9, 11, and 13 for the VC and DSSA methods with $p=22$.}  \label{tab:bci_acc_rate_p_22_supp}
\end{center}
\end{table}

\section{Consistent estimator of fourth moment}
\label{s:proofs-4moment}

The asymptotic results in Propositions \ref{p:M-loctest-vc-an} and \ref{p:global-an} involve the quantity $\mu_4 = \EE (Y_{i,t}^2-1)^2 = \EE Y_{i,t}^4-1$, that is, the fourth moment of the variables $Y_{i,t}$ in the VC model \eqref{e:intro-vcmodel}. One natural estimator of $\mu_4$ is to set 
\begin{equation}\label{e:est-mu4-0}
	\widehat \mu_4 = \frac{1}{Tp} \sum_{i=1}^p\sum_{t=1}^T \Big( (\widehat A(\frac{t}{T})^{-1} X_t)_i^4 - 1\Big).
\end{equation}
But analyzing this estimator would require being able to control $\widehat A(u)$ uniformly across $u$. This is certainly possible, and is essentially done in connection to global tests, but would require more stringent assumptions than those used for local tests in Appendix \ref{s:proofs-local} of the paper. Instead of (\ref{e:est-mu4-0}), a consistent estimator of $\mu_4$ can be constructed under the assumptions of Appendix \ref{s:proofs-local} of the paper based on the following argument. 

To get to the fourth moment of $Y_{i,t}$, we shall consider $(\mbox{tr}\{X_tX_t'\})^2$. Note that 
$$
\mbox{tr}\{X_tX_t'\} = \mbox{tr}\{A(\frac{t}{T})Y_tY_t'A(\frac{t}{T})'\} = \mbox{tr}\{A(\frac{t}{T})'A(\frac{t}{T})Y_tY_t'\} = \mbox{tr}\{A^2(\frac{t}{T})Y_tY_t'\} 
$$
$$
= \mbox{tr}\{A^2(\frac{t}{T})(Y_tY_t'-I_p)\} +  \mbox{tr}\{A^2(\frac{t}{T})\}, 
$$
where we used the symmetry of $A(u)$ to write $A(\cdot)'A(\cdot) = A(\cdot)A(\cdot)'=A^2(\cdot)$. Then,
\begin{eqnarray}
	\frac{1}{T} \sum_{t=1}^T (\mbox{tr}\{X_tX_t'\})^2 & = & \frac{1}{T} \sum_{t=1}^T \Big( \mbox{tr}\{A^2(\frac{t}{T})(Y_tY_t'-I_p)\}\Big)^2 \nonumber \\
	&  & +  \frac{2}{T} \sum_{t=1}^T  \mbox{tr}\{A^2(\frac{t}{T})(Y_tY_t'-I_p)\} \mbox{tr}\{A^2(\frac{t}{T})\} \nonumber \\
	& & +  \frac{1}{T} \sum_{t=1}^T \Big(\mbox{tr}\{A^2(\frac{t}{T})\} \Big)^2 =: R_1 + R_2 + R_3. \label{e:fourth-R123}
\end{eqnarray}

Under the assumptions of Appendix \ref{s:proofs-local} of the paper, note that $R_2\to 0$ a.s.\ Indeed, this follows from the following general argument that will be used on several occasions below. After expanding the traces, an entry in $R_2$ can be expressed as 
\begin{equation}\label{e:fourth-genarg}
	\frac{1}{T} \sum_{t=1}^T b(\frac{t}{T})Z_t,
\end{equation}
where $b(\cdot)$ is continuously differentiable and $Z_t$'s are i.i.d.\ with zero mean. By the summation by parts formula, 
$$
\frac{1}{T} \sum_{t=1}^{T}  b( \frac{t}{T} ) Z_t = \frac{1}{T} \sum_{t=1}^{T-1}  \Big( \sum_{s=1}^{t} Z_s \Big)  \Big( b( \frac{t}{T} ) - b( \frac{t+1}{T} ) \Big) +  \frac{b(1)}{T}  \sum_{t=1}^T Z_t - \frac{b(1/T)}{T}  \sum_{t=1}^{T-1} Z_t.
$$
All three last terms converge to $0$ a.s.\ by the law of large numbers. For the first term, in particular, this follows from bounding it by
$$
C \sum_{t=1}^T \Big| \sum_{s=1}^t Z_s \Big| \frac{1}{T^2} = C \sum_{t=1}^T \Big| \frac{1}{t} \sum_{s=1}^t Z_s \Big| \frac{t}{T^2} 
$$
and noting that $\frac{1}{t} \sum_{s=1}^t Z_s\to 0$ a.s.\ as $t\to\infty$. 

Under the assumptions of Appendix \ref{s:proofs-local} of the paper, $R_3\to \int_0^1 (\mbox{tr}\{A^2(u)\} )^2 du$. For the term $R_1$, note that 
$$
R_1 = \frac{1}{T} \sum_{t=1}^T \Big( \sum_{i,j=1}^p A^2_{ij}(\frac{t}{T})(Y_{i,t}Y_{j,t}-\delta_{ij}) \Big)^2 =: \frac{1}{T} \sum_{t=1}^T R_{1,t}, 
$$
where $\delta_{ij}=1$ if $i=j$, and $=0$ otherwise. By separating the sum $R_{1,t}$ into that over $i=j$ and that over $i<j$, and taking the square, we can further write
$$
R_{1,t} = R_{1,1,t} + R_{1,2,t} + R_{1,3,t} + R_{1,4,t} + R_{1,5,t},
$$
where 
\begin{eqnarray*}
	R_{1,1,t} & = & \sum_{i=1}^p (A^2_{ii}(\frac{t}{T}))^2 (Y_{i,t}^2-1)^2,\\
	R_{1,2,t} & = & \sum_{i\neq i'} A^2_{ii}(\frac{t}{T})  A^2_{i'i'}(\frac{t}{T})  (Y_{i,t}^2-1)  (Y_{i',t}^2-1),\\
	R_{1,3,t} & = & 4 \sum_{i'=1}^p A^2_{i'i'}(\frac{t}{T})  (Y_{i',t}^2-1) \sum_{i< j} A^2_{ij}(\frac{t}{T}) Y_{i,t}Y_{j,t},\\
	R_{1,4,t} & = & 4 \sum_{i< j} (A^2_{ij}(\frac{t}{T}))^2 Y_{i,t}^2 Y_{j,t}^2, \\
	R_{1,4,t} & = &  4 \sum_{i< j} \sum_{i'< j'} 1_{\{i\neq i'\ \mbox{\scriptsize or}\ j\neq j'\}} A^2_{ij}(\frac{t}{T}) A^2_{i'j'}(\frac{t}{T}) Y_{i,t}Y_{j,t}  Y_{i',t}Y_{j',t}.
\end{eqnarray*}
By the same reasoning following (\ref{e:fourth-genarg}), for $k=2,3,5$
$$
\frac{1}{T} \sum_{t=1}^T R_{1,k,t}\to 0\quad \mbox{a.s.}
$$
and 
$$
\frac{1}{T} \sum_{t=1}^T R_{1,1,t}\to \mu_4 \int_0^1 \sum_{i=1}^p (A^2_{ii}(u))^2 du,\quad 
\frac{1}{T} \sum_{t=1}^T R_{1,4,t}\to 4\int_0^1 \sum_{i<j} (A^2_{ij}(u))^2 du\quad \mbox{a.s.}
$$
By gathering the above observations, it follows from (\ref{e:fourth-R123}) that, almost surely, 
\begin{equation}\label{e:fourth-R123-conv}
	\frac{1}{T} \sum_{t=1}^T (\mbox{tr}\{X_tX_t'\})^2 \to \mu_4  \int_0^1 \sum_{i=1}^p (A^2_{ii}(u))^2 du + 4\int_0^1 \sum_{i<j} (A^2_{ij}(u))^2 du =: \mu_4  I_1 + 4I_2.
\end{equation}
We indicate how the integrals $I_1$ and $I_2$ can be estimated consistently, from which a consistent estimator of $\mu_4$ will follow.

The integrals $I_1$ and $I_2$ can be estimated through the following weighted $U$-statistics:
\begin{eqnarray*}
	\widehat I_1 & = & \frac{1}{T(T-1)} \sum_{t_1\neq t_2} \sum_{i=1}^p (X_{t_1}X_{t_1}')_{ii} (X_{t_2}X_{t_2}')_{ii} K_h(\frac{t_1}{T}-\frac{t_2}{T}),\\
	\widehat I_2 & = & \frac{1}{T(T-1)} \sum_{t_1\neq t_2} \sum_{i<j}(X_{t_1}X_{t_1}')_{ij} (X_{t_2}X_{t_2}')_{ij} K_h(\frac{t_1}{T}-\frac{t_2}{T}).
\end{eqnarray*}

\noindent The convergence of $\widehat{I}_1$ and $\widehat{I}_2$ to $I_1$ and $I_2$, respectively, can be attained by using Proposition \ref{p:proofs-global-2-Ustat-result} of the paper, which also yields convergence rates.
